# Supplementary material for: Anomalous propagators and the particle-particle channel: Bethe-Salpeter equation
Source: arXiv:2411.13167 ancillary file (2025-04-07)
Supplement: Supplementary file 1 [file si.pdf]

# Supporting information for "Anomalous propagators and the particle-particle channel: Bethe-Salpeter equation"

Antoine Marie,[1,*] Pina Romaniello,[2] Xavier Blase,[3] and Pierre-François Loos[1,†]

[1] *Laboratoire de Chimie et Physique Quantiques (UMR 5626), Université de Toulouse, CNRS, Toulouse, France*
[2] *Laboratoire de Physique Théorique, Université de Toulouse, CNRS, and European Theoretical Spectroscopy Facility (ETSF), Toulouse, France*
[3] *Université Grenoble Alpes, CNRS, Institut NÉEL, F-38042 Grenoble, France*

This document contains the detailed derivations of the equations reported in the associated main manuscript, where missing notations can be found. Section I presents the derivation of the particle-particle (pp) Bethe-Salpeter equation (BSE) in a linear-response framework. This equation is then transformed to frequency space in Sec. II and projected in a finite basis set in Sec. III. The derivation of various kernel approximations is performed in Sec. IV and the corresponding static and dynamic matrix elements are reported in Secs. V and VI, respectively. The spin adaptation of all these matrix elements is done in Sec. VII. Some additional results are given in Sec. VIII. Finally, the derivation of the $GW$ anomalous self-energies is performed in Appendix A by extending Hedin's equations to the case of the Gorkov propagator.

## CONTENTS

I. Particle-particle Bethe-Salpeter equation 2

II. Bethe-Salpeter equation in frequency space 3
A. Fourier transform 3
B. Effective dynamic kernel 4
C. Independent-particle propagator 4

III. Bethe-Salpeter equation in finite basis 5
A. Matrix elements of $K_0$ 6
B. Eigenvalue problem 7
C. Kernel matrix elements 8

IV. Kernel approximations 11
A. First-order Coulomb kernel 11
B. $GW$ kernel 11
C. Second-order Coulomb kernel 12
D. $T$-matrix kernel 12

V. Static kernel approximations 13
A. Static first-order Coulomb kernel 13
B. Static $GW$ kernel 14
C. Static second-order Coulomb kernel 15
D. Static $T$-matrix kernel 15

VI. Dynamic kernel approximations 16
A. Dynamic $GW$ kernel 16
B. Dynamic second-order Coulomb kernel 19

VII. Spin-adaptation 20
A. Spin-adaptation of the eigenvalue problem 20
B. Static first-order kernel 21
C. Static $GW$ kernel 21
D. Static second-order kernel 22

* amarie@irsamc.ups-tlse.fr
† loos@irsamc.ups-tlse.fr

E. Static $T$-matrix kernel 23
F. Dynamic $GW$ kernel 25

VIII. Results 26

A. Gorkov-Hedin equations 29

References 32

## I. PARTICLE-PARTICLE BETHE-SALPETER EQUATION

The pp-BSE is a Dyson equation for the pp propagator $K$. Its derivation in a linear-response formalism starts from the following Schwinger relation [1]

$$K(12;1'2') = \frac{1}{2}G_2(12;1'2') = \left.\frac{\delta G^{\text{ee}}(2'1';[U])}{\delta U^{\text{hh}}(12)}\right|_{U=0}, \tag{1}$$

which can then be recast as

$$\left.\frac{\delta G^{\text{ee}}(2'1')}{\delta U^{\text{hh}}(12)}\right|_{U=0} = G(32')\left.\frac{\delta (G^{-1})^{\text{ee}}(33')}{\delta U^{\text{hh}}(12)}\right|_{U=0} G(3'1') \tag{2}$$

using the definition of the inverse Gorkov propagator [1]. In the above equation and the following ones, integration over repeated indices is assumed. In addition, the explicit $U$ dependence is only written in Eq. (1) and is dropped after for the sake of conciseness. The Gorkov-Dyson equation,

$$\boldsymbol{G}^{-1}(11') = \boldsymbol{G}_0^{-1}(11') - \begin{pmatrix} \Sigma^{\text{he}}(11') & \Sigma^{\text{hh}}(11') + U^{\text{ee}}(11') \\ \Sigma^{\text{ee}}(11') + U^{\text{hh}}(11') & \Sigma^{\text{eh}}(11') \end{pmatrix}, \tag{3}$$

can now be inserted into the Schwinger relation which yields

$$K(12;1'2') = -G(32')\left.\frac{\delta U^{\text{hh}}(33')}{\delta U^{\text{hh}}(12)}\right|_{U=0} G(3'1') - G(32')\left.\frac{\delta \Sigma^{\text{ee}}(33')}{\delta U^{\text{hh}}(12)}\right|_{U=0} G(3'1'). \tag{4}$$

Using the following property

$$\frac{\delta U^{\text{hh}}(12)}{\delta U^{\text{hh}}(34)} = \frac{1}{2}[\delta(13)\delta(24) - \delta(14)\delta(23)], \tag{5}$$

the first term is identified as the pp non-interacting propagator

$$K_0(12;1'2') = \frac{1}{2}[G(11')G(22') - G(12')G(21')]. \tag{6}$$

The last step to obtain a Dyson equation for $K$ is to apply the derivative chain rule to the second term,

$$\begin{aligned} K(12;1'2') = K_0(12;1'2') - G(32')G(3'1')\Bigg[ &\left.\frac{\delta G^{\text{he}}(44')}{\delta U^{\text{hh}}(12)}\right|_{U=0}\left.\frac{\delta \Sigma^{\text{ee}}(33')}{\delta G^{\text{he}}(44')}\right|_{U=0} + \left.\frac{\delta G^{\text{hh}}(44')}{\delta U^{\text{hh}}(12)}\right|_{U=0}\left.\frac{\delta \Sigma^{\text{ee}}(33')}{\delta G^{\text{hh}}(44')}\right|_{U=0} \\ &+ \left.\frac{\delta G^{\text{ee}}(44')}{\delta U^{\text{hh}}(12)}\right|_{U=0}\left.\frac{\delta \Sigma^{\text{ee}}(33')}{\delta G^{\text{ee}}(44')}\right|_{U=0} + \left.\frac{\delta G^{\text{eh}}(44')}{\delta U^{\text{hh}}(12)}\right|_{U=0}\left.\frac{\delta \Sigma^{\text{ee}}(33')}{\delta G^{\text{eh}}(44')}\right|_{U=0}\Bigg], \end{aligned} \tag{7}$$

where, out of the four terms, only one survives at $U = 0$, that is,

$$K(12;1'2') = K_0(12;1'2') - G(32')\left.\frac{\delta G^{\text{ee}}(44')}{\delta U^{\text{hh}}(12)}\right|_{U=0}\left.\frac{\delta \Sigma^{\text{ee}}(33')}{\delta G^{\text{ee}}(44')}\right|_{U=0} G(3'1'). \tag{8}$$

Finally, once $K$ has been identified, the equation reads

$$K(12;1'2') = K_0(12;1'2') - K(12;44')\Xi^{\text{pp}}(44';33')K_0(33';1'2'), \tag{9}$$

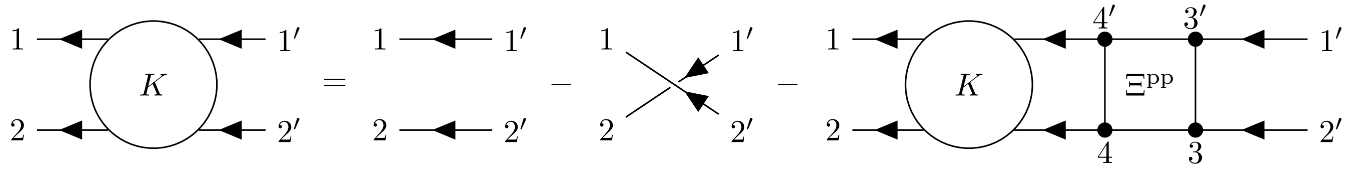


FIG. 1. Diagrammatic representations of the pp-BSE [see Eq. (9)]. Note that $K_0(33';1'2')$ has been replaced by the product $G(31')G(3'2')$ in the right-hand side of Eq. (9) using the antisymmetric nature of the kernel.

where the pp kernel

$$\Xi^{\text{pp}}(44';33') = \left.\frac{\delta\Sigma^{\text{ee}}(33')}{\delta G^{\text{ee}}(44')}\right|_{U=0}, \tag{10}$$

has been introduced and $K_0$ has been recovered by exploiting the antisymmetric nature of the kernel

$$\Xi^{\text{pp}}(44';33') = -\Xi^{\text{pp}}(4'4;33') = -\Xi^{\text{pp}}(44';3'3) = \Xi^{\text{pp}}(4'4;3'3). \tag{11}$$

This equation is represented diagrammatically in Fig. 1.

## II. BETHE-SALPETER EQUATION IN FREQUENCY SPACE

### A. Fourier transform

The aim of this first subsection is to Fourier transform the pp-BSE derived in Eq. (9). The pp propagator $K$ depends on four space-spin variables and, because the Hamiltonian is time-independent, on three time differences

$$K(12;1'2') = K(\mathbf{x}_1\mathbf{x}_2;\mathbf{x}_{1'}\mathbf{x}_{2'};\tau_{12},\tau_{1'2'},\tau_{12,1'2'}), \tag{12}$$

with $\tau_{ii'} = t_i - t_{i'}$ and $\tau_{ij,i'j'} = (\tau_{ii'} + \tau_{jj'})/2$. The triple Fourier transform is defined as

$$K(\mathbf{x}_1\mathbf{x}_2;\mathbf{x}_{1'}\mathbf{x}_{2'};\omega,\omega',\omega'') = \int \mathrm{d}(\tau_{12}\tau_{1'2'}\tau_{12,1'2'})\, e^{\mathrm{i}\omega\tau_{12}+\mathrm{i}\omega'\tau_{1'2'}+\mathrm{i}\omega''\tau_{12,1'2'}} K(\mathbf{x}_1\mathbf{x}_2;\mathbf{x}_{1'}\mathbf{x}_{2'};\tau_{12},\tau_{1'2'},\tau_{12,1'2'}). \tag{13}$$

In the following derivation, only the time variables and time integrals are explicitly written down. Using these notations, the time dependence of the pp-BSE reads

$$\begin{aligned} K(\tau_{12},\tau_{1'2'},\tau_{12,1'2'}) &= K_0(\tau_{12},\tau_{1'2'},\tau_{12,1'2'}) \\ &\quad - \int \mathrm{d}(t_3t_{3'}t_4t_{4'})\, K(\tau_{12},\tau_{44'},\tau_{12,44'})\Xi^{\text{pp}}(\tau_{44'},\tau_{33'},\tau_{44',33'})K_0(\tau_{33'},\tau_{1'2'},\tau_{33',1'2'}) \end{aligned} \tag{14}$$

and the Fourier transform of this equation is performed as follows

$$\begin{aligned} K(\omega,\omega',\omega'') &= K_0(\omega,\omega',\omega'') \\ &\quad - \int \mathrm{d}(\tau_{12,1'2'})\,\mathrm{d}(t_3t_{3'}t_4t_{4'})\, e^{\mathrm{i}\omega''\tau_{12,1'2'}} K(\omega,\tau_{44'},\tau_{12,44'})\Xi^{\text{pp}}(\tau_{44'},\tau_{33'},\tau_{44',33'})K_0(\tau_{33'},\omega',\tau_{33',1'2'}) \\ &= K_0(\omega,\omega',\omega'') \\ &\quad - \int \mathrm{d}(\tau_{12,1'2'})\,\mathrm{d}(t_3t_{3'}t_4t_{4'})\, e^{\mathrm{i}\omega''\tau_{12,1'2'}} K(\omega,\tau_{44'},\tau_{12,44'})\Xi^{\text{pp}}(\tau_{44'},\tau_{33'},\tau_{44',33'})\left(\frac{1}{2\pi}\int \mathrm{d}\bar{\omega}\, e^{-\mathrm{i}\bar{\omega}\tau_{33'}} K_0(\bar{\omega},\omega',\tau_{33',1'2'})\right) \\ &= K_0(\omega,\omega',\omega'') - \frac{1}{2\pi}\int \mathrm{d}(\tau_{12,1'2'})\,\mathrm{d}(\bar{\omega})\,\mathrm{d}(t_{3'}t_4t_{4'})\, e^{\mathrm{i}\omega''\tau_{12,1'2'}} K(\omega,\tau_{44'},\tau_{12,44'})\Xi^{\text{pp}}(\tau_{44'},-\bar{\omega},\tau_{44',33'})K_0(\bar{\omega},\omega',\tau_{33',1'2'}) \\ &= K_0(\omega,\omega',\omega'') - \frac{1}{(2\pi)^2}\int \mathrm{d}(\tau_{12,1'2'})\,\mathrm{d}(\bar{\omega}\tilde{\omega})\,\mathrm{d}(t_{3'}t_{4'})\, e^{\mathrm{i}\omega''\tau_{12,1'2'}} K(\omega,\tilde{\omega},\tau_{12,44'})\Xi^{\text{pp}}(-\tilde{\omega},-\bar{\omega},\tau_{44',33'})K_0(\bar{\omega},\omega',\tau_{33',1'2'}) \\ &= K_0(\omega,\omega',\omega'') \\ &\quad - \frac{1}{(2\pi)^2}\int \mathrm{d}(\tau_{12,1'2'})\,\mathrm{d}(\bar{\omega}\tilde{\omega})\,\mathrm{d}(t_{3'}t_{4'})\, e^{\mathrm{i}\omega''(\tau_{12,44'}+\tau_{44',33'}+\tau_{33',1'2'})} K(\omega,\tilde{\omega},\tau_{12,44'})\Xi^{\text{pp}}(-\tilde{\omega},-\bar{\omega},\tau_{44',33'})K_0(\bar{\omega},\omega',\tau_{33',1'2'}) \end{aligned}$$

$$= K_0(\omega,\omega',\omega'') - \frac{1}{(2\pi)^2}\int \mathrm{d}(\bar{\omega}\tilde{\omega})\, K(\omega,\tilde{\omega},\omega'')\Xi^{\mathrm{pp}}(-\tilde{\omega},-\bar{\omega},\omega'')K_0(\bar{\omega},\omega',\omega'').$$

In practice, the pairs of particles are assumed to be created and annihilated instantaneously, *i.e.*, $t_2 = t_1^+ = t_1 + \eta$ and $t_{2'} = t_{1'}^+$ where $\eta$ is a positive infinitesimal. Hence, one is interested in the single-frequency pp propagator $K(\omega) = \lim_{\eta\to 0^+} K(-\eta,-\eta,\omega)$. Under this assumption, the pp-BSE simplifies as

$$K(\omega'') = K_0(\omega'') - \frac{1}{(2\pi)^2}\int \mathrm{d}(\bar{\omega}\tilde{\omega})\, K(-\eta,\tilde{\omega},\omega'')\Xi^{\mathrm{pp}}(-\tilde{\omega},-\bar{\omega},\omega'')K_0(\bar{\omega},-\eta,\omega''), \tag{15}$$

where the $\eta$ limit has not been written for the sake of conciseness.

### B. Effective dynamic kernel

Unfortunately, because the kernel depends on three frequencies, the above equation cannot be inverted. Following the methodology introduced for the usual electron-hole (eh) BSE case [2], an effective dynamic kernel is defined as

$$\tilde{\Xi}^{\mathrm{pp}}(\omega) = \frac{1}{(2\pi)^2}\int \mathrm{d}(\tilde{\omega}\bar{\omega})\,(K^{-1})(\omega)K(\bar{\omega},-\eta,\omega)\Xi^{\mathrm{pp}}(-\tilde{\omega},-\bar{\omega},\omega)K_0(-\eta,\tilde{\omega},\omega)(K_0^{-1})(\omega) \tag{16}$$

such that the pp-BSE becomes

$$K(\omega) = K_0(\omega) - K(\omega)\tilde{\Xi}^{\mathrm{pp}}(\omega)K_0(\omega), \tag{17}$$

and is now easily invertible, as follows

$$K^{-1}(\omega) = K_0^{-1}(\omega) + \tilde{\Xi}^{\mathrm{pp}}(\omega). \tag{18}$$

However, as readily seen in Eq. (16), its kernel self-consistently depends on $K$. In order to suppress this dependency, the effective kernel is approximated as

$$\tilde{\Xi}^{\mathrm{pp}}(\omega) \approx \frac{1}{(2\pi)^2}\int \mathrm{d}(\tilde{\omega}\bar{\omega})\,(K_0^{-1})(\omega)K_0(\bar{\omega},-\eta,\omega)\Xi^{\mathrm{pp}}(-\tilde{\omega},-\bar{\omega},\omega)K_0(-\eta,\tilde{\omega},\omega)(K_0^{-1})(\omega), \tag{19}$$

where one simply replaces the kernel $K$ by its independent-particle version $K_0$ in Eq. (16).

### C. Independent-particle propagator

To conclude this section, the frequency-space expression of the non-interacting pp propagator is derived below. Its time dependence can be recast as

$$\begin{aligned}
K_0(\mathbf{x}_1\mathbf{x}_2;\mathbf{x}_{1'}\mathbf{x}_{2'};\tau_{12},\tau_{1'2'},\tau_{12,1'2'}) &= \frac{1}{2}G(\mathbf{x}_1\mathbf{x}_{1'};\tau_{11'})G(\mathbf{x}_2\mathbf{x}_{2'};\tau_{22'}) - \frac{1}{2}G(\mathbf{x}_2\mathbf{x}_{1'};\tau_{21'})G(\mathbf{x}_1\mathbf{x}_{2'};\tau_{12'})\\
&= \frac{1}{2}G(\mathbf{x}_1\mathbf{x}_{1'};\frac{\tau_{12}-\tau_{1'2'}}{2}+\tau_{12,1'2'})G(\mathbf{x}_2\mathbf{x}_{2'};\frac{-\tau_{12}+\tau_{1'2'}}{2}+\tau_{12,1'2'})\\
&\quad - \frac{1}{2}G(\mathbf{x}_2\mathbf{x}_{1'};\frac{-\tau_{12}-\tau_{1'2'}}{2}+\tau_{12,1'2'})G(\mathbf{x}_1\mathbf{x}_{2'};\frac{\tau_{12}+\tau_{1'2'}}{2}+\tau_{12,1'2'}),
\end{aligned}$$

which set the stage for the Fourier transform

$$\begin{aligned}
K_0(\omega,\omega',\omega'') &= \int \mathrm{d}(\tau_{12}\tau_{1'2'}\tau_{12,1'2'})\, e^{\mathrm{i}\omega\tau_{12}+\mathrm{i}\omega'\tau_{1'2'}+\mathrm{i}\omega''\tau_{12,1'2'}} K_0(\mathbf{x}_1\mathbf{x}_2;\mathbf{x}_{1'}\mathbf{x}_{2'};\tau_{12},\tau_{1'2'},\tau_{12,1'2'})\\
&= \frac{1}{2}\int \mathrm{d}(\tau_{12}\tau_{1'2'}\tau_{12,1'2'})\, e^{\mathrm{i}\omega\tau_{12}+\mathrm{i}\omega'\tau_{1'2'}+\mathrm{i}\omega''\tau_{12,1'2'}}\\
&\quad\times\left(\frac{1}{2\pi}\int \mathrm{d}\tilde{\omega} e^{-\mathrm{i}(\frac{\tau_{12}-\tau_{1'2'}}{2}+\tau_{12,1'2'})\tilde{\omega}}G(\mathbf{x}_1\mathbf{x}_{1'};\tilde{\omega})\right)\left(\frac{1}{2\pi}\int \mathrm{d}\bar{\omega} e^{-\mathrm{i}(\frac{-\tau_{12}+\tau_{1'2'}}{2}+\tau_{12,1'2'})\bar{\omega}}G(\mathbf{x}_2\mathbf{x}_{2'};\bar{\omega})\right)
\end{aligned}$$

$$
\begin{aligned}
&-\frac{1}{2}\int \mathrm{d}(\tau_{12}\tau_{1'2'}\tau_{12,1'2'})\, e^{\mathrm{i}\omega\tau_{12}+\mathrm{i}\omega'\tau_{1'2'}+\mathrm{i}\omega''\tau_{12,1'2'}} \\
&\qquad\qquad \times\left(\frac{1}{2\pi}\int \mathrm{d}\tilde{\omega} e^{-\mathrm{i}(\frac{-\tau_{12}-\tau_{1'2'}}{2}+\tau_{12,1'2'})\tilde{\omega}} G(\mathbf{x}_2\mathbf{x}_{1'};\tilde{\omega})\right)\left(\frac{1}{2\pi}\int \mathrm{d}\bar{\omega} e^{-\mathrm{i}(\frac{\tau_{12}+\tau_{1'2'}}{2}+\tau_{12,1'2'})\bar{\omega}} G(\mathbf{x}_1\mathbf{x}_{2'};\bar{\omega})\right) \\
&=\frac{1}{2(2\pi)^2}\int \mathrm{d}(\tilde{\omega}\bar{\omega})\, G(\mathbf{x}_1\mathbf{x}_{1'};\tilde{\omega})G(\mathbf{x}_2\mathbf{x}_{2'};\bar{\omega})\int \mathrm{d}\tau_{12} e^{\mathrm{i}\tau_{12}(\omega-\frac{\tilde{\omega}}{2}+\frac{\bar{\omega}}{2})}\int \mathrm{d}\tau_{1'2'} e^{\mathrm{i}\tau_{1'2'}(\omega'+\frac{\tilde{\omega}}{2}-\frac{\bar{\omega}}{2})}\int \mathrm{d}\tau_{12,1'2'} e^{\mathrm{i}\tau_{12,1'2'}(\omega''-\tilde{\omega}-\bar{\omega})} \\
&\quad -\frac{1}{2(2\pi)^2}\int \mathrm{d}(\tilde{\omega}\bar{\omega})\, G(\mathbf{x}_2\mathbf{x}_{1'};\tilde{\omega})G(\mathbf{x}_1\mathbf{x}_{2'};\bar{\omega})\int \mathrm{d}\tau_{12} e^{\mathrm{i}\tau_{12}(\omega+\frac{\tilde{\omega}}{2}-\frac{\bar{\omega}}{2})}\int \mathrm{d}\tau_{1'2'} e^{\mathrm{i}\tau_{1'2'}(\omega'+\frac{\tilde{\omega}}{2}-\frac{\bar{\omega}}{2})}\int \mathrm{d}\tau_{12,1'2'} e^{\mathrm{i}\tau_{12,1'2'}(\omega''-\tilde{\omega}-\bar{\omega})} \\
&=\frac{2\pi}{2}\int \mathrm{d}(\tilde{\omega}\bar{\omega})\, G(\mathbf{x}_1\mathbf{x}_{1'};\tilde{\omega})G(\mathbf{x}_2\mathbf{x}_{2'};\bar{\omega})\delta(\omega-\frac{\tilde{\omega}}{2}+\frac{\bar{\omega}}{2})\delta(\omega'+\frac{\tilde{\omega}}{2}-\frac{\bar{\omega}}{2})\delta(\omega''-\tilde{\omega}-\bar{\omega}) \\
&\qquad\qquad -\frac{2\pi}{2}\int \mathrm{d}(\tilde{\omega}\bar{\omega})\, G(\mathbf{x}_2\mathbf{x}_{1'};\tilde{\omega})G(\mathbf{x}_1\mathbf{x}_{2'};\bar{\omega})\delta(\omega+\frac{\tilde{\omega}}{2}-\frac{\bar{\omega}}{2})\delta(\omega'+\frac{\tilde{\omega}}{2}-\frac{\bar{\omega}}{2})\delta(\omega''-\tilde{\omega}-\bar{\omega}) \\
&=\frac{2\pi}{2}\int \mathrm{d}\tilde{\omega} G(\mathbf{x}_1\mathbf{x}_{1'};\tilde{\omega})G(\mathbf{x}_2\mathbf{x}_{2'};\omega''-\tilde{\omega})\delta(\omega-\tilde{\omega}+\frac{\omega''}{2})\delta(\omega'+\tilde{\omega}-\frac{\omega''}{2}) \\
&\qquad\qquad -\frac{2\pi}{2}\int \mathrm{d}\tilde{\omega} G(\mathbf{x}_2\mathbf{x}_{1'};\tilde{\omega})G(\mathbf{x}_1\mathbf{x}_{2'};\omega''-\tilde{\omega})\delta(\omega+\tilde{\omega}-\frac{\omega''}{2})\delta(\omega'+\tilde{\omega}-\frac{\omega''}{2}) \\
&=\pi G(\mathbf{x}_1\mathbf{x}_{1'};\frac{\omega''}{2}-\omega')G(\mathbf{x}_2\mathbf{x}_{2'};\frac{\omega''}{2}+\omega')\delta(\omega+\omega')-\pi G(\mathbf{x}_2\mathbf{x}_{1'};\frac{\omega''}{2}-\omega')G(\mathbf{x}_1\mathbf{x}_{2'};\frac{\omega''}{2}+\omega')\delta(\omega-\omega').
\end{aligned}
$$

The single-frequency non-interacting propagator can be obtained as a special case and is given by

$$
K_0(\omega'')=\frac{1}{4\pi}\int \mathrm{d}\omega'\, G(\mathbf{x}_1\mathbf{x}_{1'};\omega''-\omega')G(\mathbf{x}_2\mathbf{x}_{2'};\omega')-\frac{1}{4\pi}\int \mathrm{d}\omega'\, e^{\mathrm{i}2\eta\omega'} G(\mathbf{x}_2\mathbf{x}_{1'};\omega''-\omega')G(\mathbf{x}_1\mathbf{x}_{2'};\omega'). \tag{20}
$$

As can be seen in the expression of the effective kernel [see Eq. (19)], the two-frequency propagators are also required and can be obtained as

$$
K_0(-\eta,\omega',\omega'')=\frac{e^{-\mathrm{i}\eta\omega'}}{2}G(\mathbf{x}_1\mathbf{x}_{1'};\frac{\omega''}{2}-\omega')G(\mathbf{x}_2\mathbf{x}_{2'};\frac{\omega''}{2}+\omega')-\frac{e^{\mathrm{i}\eta\omega'}}{2}G(\mathbf{x}_2\mathbf{x}_{1'};\frac{\omega''}{2}-\omega')G(\mathbf{x}_1\mathbf{x}_{2'};\frac{\omega''}{2}+\omega'), \tag{21a}
$$

$$
K_0(\omega,-\eta,\omega'')=\frac{e^{-\mathrm{i}\eta\omega}}{2}G(\mathbf{x}_1\mathbf{x}_{1'};\frac{\omega''}{2}+\omega)G(\mathbf{x}_2\mathbf{x}_{2'};\frac{\omega''}{2}-\omega)-\frac{e^{\mathrm{i}\eta\omega}}{2}G(\mathbf{x}_2\mathbf{x}_{1'};\frac{\omega''}{2}-\omega)G(\mathbf{x}_1\mathbf{x}_{2'};\frac{\omega''}{2}+\omega). \tag{21b}
$$

Thus, we have $K_0(-\eta,\omega,\omega'')=K_0(\omega,-\eta,\omega'')$ and we shall use the same notation $K_0(\omega,\omega'')$ for both.

## III. BETHE-SALPETER EQUATION IN FINITE BASIS

We recall that a general 4-point quantity is projected into a finite basis set of one-body orbitals $\varphi_p(\mathbf{x})$ using

$$
K_{pqrs}(\omega)=\int \mathrm{d}(\mathbf{x}_1\mathbf{x}_2\mathbf{x}_{1'}\mathbf{x}_{2'})\,\varphi_p^*(\mathbf{x}_1)\varphi_q^*(\mathbf{x}_2)K(\mathbf{x}_1\mathbf{x}_2;\mathbf{x}_{1'}\mathbf{x}_{2'};\omega)\varphi_r(\mathbf{x}_{1'})\varphi_s(\mathbf{x}_{2'}). \tag{22}
$$

Thus, once projected, the pp-BSE given in Eq. (17) becomes

$$
K_{pqrs}(\omega)=(K_0)_{pqrs}(\omega)-K_{pqvw}(\omega)\tilde{\Xi}^{\text{pp}}_{vwtu}(\omega)(K_0)_{turs}(\omega). \tag{23}
$$

The 4-point tensors can be written as matrices with composite indices as $K_{pqrs}(\omega)=K_{pq,rs}(\omega)$ such that the pp-BSE becomes the following matrix equation

$$
\begin{aligned}
\boldsymbol{K}(\omega)&=\boldsymbol{K}_0(\omega)-\boldsymbol{K}(\omega)\cdot\tilde{\boldsymbol{\Xi}}(\omega)\cdot\boldsymbol{K}_0(\omega)\\
\boldsymbol{K}(\omega)\cdot\boldsymbol{K}_0^{-1}(\omega)&=\mathbf{1}-\boldsymbol{K}(\omega)\cdot\tilde{\boldsymbol{\Xi}}(\omega)\\
\boldsymbol{K}^{-1}(\omega)&=\boldsymbol{K}_0^{-1}(\omega)+\tilde{\boldsymbol{\Xi}}(\omega)
\end{aligned} \tag{24}
$$

where $\mathbf{1}$ is the identity matrix. The aim is to find the zeros of $\boldsymbol{K}^{-1}(\omega)$. Hence, as a first step, we compute the matrix elements of $\boldsymbol{K}_0(\omega)$ and $\tilde{\boldsymbol{\Xi}}(\omega)$. The matrix elements of $\boldsymbol{K}_0$ are explicitly given in the following subsection while, in this section, we assume a generic kernel with matrix elements $\tilde{\Xi}_{pq,rs}(\omega)$. The following sections report an in-depth discussion of kernel approximations.

### A. Matrix elements of $K_0$

The non-interacting pp propagator is composed of two terms, that is, $K_0(\omega) = K_0^{\text{I}}(\omega) + K_0^{\text{II}}(\omega)$ with

$$K_0^{\text{I}}(\omega) = \frac{1}{4\pi} \int d\omega' \, G(\mathbf{x}_1\mathbf{x}_{1'};\omega-\omega')G(\mathbf{x}_2\mathbf{x}_{2'};\omega'), \tag{25a}$$

$$K_0^{\text{II}}(\omega) = -\frac{1}{4\pi} \int d\omega' \, e^{\mathrm{i}2\eta\omega'} G(\mathbf{x}_2\mathbf{x}_{1'};\omega-\omega')G(\mathbf{x}_1\mathbf{x}_{2'};\omega'). \tag{25b}$$

Their matrix elements will be computed separately. We recall the Lehmann representation of the one-body Green's function in the quasiparticle approximation

$$G(\mathbf{x}_1\mathbf{x}_{1'};\omega) = \sum_i \frac{\varphi_i(\mathbf{x}_1)\varphi_i^*(\mathbf{x}_{1'})}{\omega-\epsilon_i-\mathrm{i}\eta} + \sum_a \frac{\varphi_a(\mathbf{x}_1)\varphi_a^*(\mathbf{x}_{1'})}{\omega-\epsilon_a+\mathrm{i}\eta}, \tag{26}$$

where $\epsilon_i$ and $\epsilon_a$ are occupied and virtual one-body energies, respectively.

The first term is computed as

$$\begin{aligned}
K_0^{\text{I}}(\omega) &= \frac{1}{4\pi} \int d\omega' \, e^{\mathrm{i}2\eta\omega'} G(\mathbf{x}_1\mathbf{x}_{1'};\omega-\omega')G(\mathbf{x}_2\mathbf{x}_{2'};\omega') \\
&= \frac{1}{4\pi} \int d\omega' \, e^{\mathrm{i}2\eta\omega'} \left[\sum_i \frac{\varphi_i(\mathbf{x}_1)\varphi_i^*(\mathbf{x}_{1'})}{\omega-\omega'-(\epsilon_i+\mathrm{i}\eta)} + \sum_a \frac{\varphi_a(\mathbf{x}_1)\varphi_a^*(\mathbf{x}_{1'})}{\omega-\omega'-(\epsilon_a-\mathrm{i}\eta)}\right] \left[\sum_j \frac{\varphi_j(\mathbf{x}_2)\varphi_j^*(\mathbf{x}_{2'})}{\omega'-(\epsilon_j+\mathrm{i}\eta)} + \sum_b \frac{\varphi_b(\mathbf{x}_2)\varphi_b^*(\mathbf{x}_{2'})}{\omega'-(\epsilon_b-\mathrm{i}\eta)}\right] \\
&= -\frac{1}{4\pi} \int d\omega' \, e^{\mathrm{i}2\eta\omega'} \left[\sum_i \frac{\varphi_i(\mathbf{x}_1)\varphi_i^*(\mathbf{x}_{1'})}{\omega'-(\omega-\epsilon_i-\mathrm{i}\eta)} + \sum_a \frac{\varphi_a(\mathbf{x}_1)\varphi_a^*(\mathbf{x}_{1'})}{\omega'-(\omega-\epsilon_a+\mathrm{i}\eta)}\right] \left[\sum_j \frac{\varphi_j(\mathbf{x}_2)\varphi_j^*(\mathbf{x}_{2'})}{\omega'-(\epsilon_j+\mathrm{i}\eta)} + \sum_b \frac{\varphi_b(\mathbf{x}_2)\varphi_b^*(\mathbf{x}_{2'})}{\omega'-(\epsilon_b-\mathrm{i}\eta)}\right] \\
&= -\frac{1}{4\pi} \int d\omega' \, e^{\mathrm{i}2\eta\omega'} \sum_{ij} \frac{\varphi_i(\mathbf{x}_1)\varphi_i^*(\mathbf{x}_{1'})}{\omega'-(\omega-\epsilon_i-\mathrm{i}\eta)} \frac{\varphi_j(\mathbf{x}_2)\varphi_j^*(\mathbf{x}_{2'})}{\omega'-(\epsilon_j+\mathrm{i}\eta)} - \frac{1}{4\pi} \int d\omega' \, e^{\mathrm{i}2\eta\omega'} \sum_{ab} \frac{\varphi_a(\mathbf{x}_1)\varphi_a^*(\mathbf{x}_{1'})}{\omega'-(\omega-\epsilon_a+\mathrm{i}\eta)} \frac{\varphi_b(\mathbf{x}_2)\varphi_b^*(\mathbf{x}_{2'})}{\omega'-(\epsilon_b-\mathrm{i}\eta)} \\
&= -\frac{2\pi\mathrm{i}}{4\pi} \sum_{ij} \frac{\varphi_i(\mathbf{x}_1)\varphi_i^*(\mathbf{x}_{1'})\varphi_j(\mathbf{x}_2)\varphi_j^*(\mathbf{x}_{2'})}{(\epsilon_j+\mathrm{i}\eta)-(\omega-\epsilon_i-\mathrm{i}\eta)} - \frac{2\pi\mathrm{i}}{4\pi} \sum_{ab} \frac{\varphi_a(\mathbf{x}_1)\varphi_a^*(\mathbf{x}_{1'})\varphi_b(\mathbf{x}_2)\varphi_b^*(\mathbf{x}_{2'})}{(\omega-\epsilon_a+\mathrm{i}\eta)-(\epsilon_b-\mathrm{i}\eta)} \\
&= \frac{\mathrm{i}}{2} \sum_{ij} \frac{\varphi_i(\mathbf{x}_1)\varphi_i^*(\mathbf{x}_{1'})\varphi_j(\mathbf{x}_2)\varphi_j^*(\mathbf{x}_{2'})}{\omega-(\epsilon_j+\epsilon_i+2\mathrm{i}\eta)} - \frac{\mathrm{i}}{2} \sum_{ab} \frac{\varphi_a(\mathbf{x}_1)\varphi_a^*(\mathbf{x}_{1'})\varphi_b(\mathbf{x}_2)\varphi_b^*(\mathbf{x}_{2'})}{\omega-(\epsilon_a+\epsilon_b-2\mathrm{i}\eta)},
\end{aligned}$$

and, once projected in the finite basis set, reads

$$(K_0^{\text{I}})_{pqrs}(\omega) = \frac{\mathrm{i}}{2}\left[\sum_{ij} \frac{\delta_{pi}\delta_{qj}\delta_{ri}\delta_{sj}}{\omega-(\epsilon_j+\epsilon_i+2\mathrm{i}\eta)} - \sum_{ab} \frac{\delta_{pa}\delta_{qb}\delta_{ra}\delta_{sb}}{\omega-(\epsilon_a+\epsilon_b-2\mathrm{i}\eta)}\right]. \tag{27}$$

The second term is computed as

$$\begin{aligned}
K_0^{\text{II}}(\omega) &= -\frac{1}{4\pi} \int d\omega' \, G(\mathbf{x}_2\mathbf{x}_{1'};\omega-\omega')G(\mathbf{x}_1\mathbf{x}_{2'};\omega') \\
&= -\frac{1}{4\pi} \int d\omega' \left[\sum_i \frac{\varphi_i(\mathbf{x}_2)\varphi_i^*(\mathbf{x}_{1'})}{\omega-\omega'-(\epsilon_i+\mathrm{i}\eta)} + \sum_a \frac{\varphi_a(\mathbf{x}_2)\varphi_a^*(\mathbf{x}_{1'})}{\omega-\omega'-(\epsilon_a-\mathrm{i}\eta)}\right] \left[\sum_j \frac{\varphi_j(\mathbf{x}_1)\varphi_j^*(\mathbf{x}_{2'})}{\omega'-(\epsilon_j+\mathrm{i}\eta)} + \sum_b \frac{\varphi_b(\mathbf{x}_1)\varphi_b^*(\mathbf{x}_{2'})}{\omega'-(\epsilon_b-\mathrm{i}\eta)}\right] \\
&= \frac{1}{4\pi} \int d\omega' \left[\sum_i \frac{\varphi_i(\mathbf{x}_2)\varphi_i^*(\mathbf{x}_{1'})}{\omega'-(\omega-\epsilon_i-\mathrm{i}\eta)} + \sum_a \frac{\varphi_a(\mathbf{x}_2)\varphi_a^*(\mathbf{x}_{1'})}{\omega'-(\omega-\epsilon_a+\mathrm{i}\eta)}\right] \left[\sum_j \frac{\varphi_j(\mathbf{x}_1)\varphi_j^*(\mathbf{x}_{2'})}{\omega'-(\epsilon_j+\mathrm{i}\eta)} + \sum_b \frac{\varphi_b(\mathbf{x}_1)\varphi_b^*(\mathbf{x}_{2'})}{\omega'-(\epsilon_b-\mathrm{i}\eta)}\right] \\
&= \frac{1}{4\pi} \int d\omega' \sum_{ij} \frac{\varphi_i(\mathbf{x}_2)\varphi_i^*(\mathbf{x}_{1'})}{\omega'-(\omega-\epsilon_i-\mathrm{i}\eta)} \frac{\varphi_j(\mathbf{x}_1)\varphi_j^*(\mathbf{x}_{2'})}{\omega'-(\epsilon_j+\mathrm{i}\eta)} + \frac{1}{4\pi} \int d\omega' \sum_{ab} \frac{\varphi_a(\mathbf{x}_2)\varphi_a^*(\mathbf{x}_{1'})}{\omega'-(\omega-\epsilon_a+\mathrm{i}\eta)} \frac{\varphi_b(\mathbf{x}_1)\varphi_b^*(\mathbf{x}_{2'})}{\omega'-(\epsilon_b-\mathrm{i}\eta)} \\
&= \frac{2\pi\mathrm{i}}{4\pi} \sum_{ij} \frac{\varphi_i(\mathbf{x}_2)\varphi_i^*(\mathbf{x}_{1'})\varphi_j(\mathbf{x}_1)\varphi_j^*(\mathbf{x}_{2'})}{(\epsilon_j+\mathrm{i}\eta)-(\omega-\epsilon_i-\mathrm{i}\eta)} + \frac{2\pi\mathrm{i}}{4\pi} \sum_{ab} \frac{\varphi_a(\mathbf{x}_2)\varphi_a^*(\mathbf{x}_{1'})\varphi_b(\mathbf{x}_1)\varphi_b^*(\mathbf{x}_{2'})}{(\omega-\epsilon_a+\mathrm{i}\eta)-(\epsilon_b-\mathrm{i}\eta)} \\
&= -\frac{\mathrm{i}}{2} \sum_{ij} \frac{\varphi_i(\mathbf{x}_2)\varphi_i^*(\mathbf{x}_{1'})\varphi_j(\mathbf{x}_1)\varphi_j^*(\mathbf{x}_{2'})}{\omega-(\epsilon_j+\epsilon_i+2\mathrm{i}\eta)} + \frac{\mathrm{i}}{2} \sum_{ab} \frac{\varphi_a(\mathbf{x}_2)\varphi_a^*(\mathbf{x}_{1'})\varphi_b(\mathbf{x}_1)\varphi_b^*(\mathbf{x}_{2'})}{\omega-(\epsilon_a+\epsilon_b-2\mathrm{i}\eta)},
\end{aligned}$$

and, once projected in the finite basis set, reads

$$(K_0^{\mathrm{II}})_{pqrs}(\omega) = \frac{\mathrm{i}}{2}\left[-\sum_{ij}\frac{\delta_{qi}\delta_{pj}\delta_{ri}\delta_{sj}}{\omega-(\epsilon_j+\epsilon_i+2\mathrm{i}\eta)}+\sum_{ab}\frac{\delta_{qa}\delta_{pb}\delta_{ra}\delta_{sb}}{\omega-(\epsilon_a+\epsilon_b-2\mathrm{i}\eta)}\right]. \tag{28}$$

These two expressions are gathered to form the tensor elements of $K_0$

$$\begin{aligned}(K_0)_{pqrs}(\omega) &= (K_0^{\mathrm{I}})_{pqrs}(\omega)+(K_0^{\mathrm{II}})_{pqrs}(\omega)\\ &= \frac{\mathrm{i}}{2}\left[\sum_{ij}\frac{\delta_{qj}\delta_{pi}\delta_{ri}\delta_{sj}}{\omega-(\epsilon_j+\epsilon_i+2\mathrm{i}\eta)}-\sum_{ab}\frac{\delta_{qb}\delta_{pa}\delta_{ra}\delta_{sb}}{\omega-(\epsilon_a+\epsilon_b-2\mathrm{i}\eta)}\right]\\ &\quad-\frac{\mathrm{i}}{2}\left[\sum_{ij}\frac{\delta_{pj}\delta_{qi}\delta_{ri}\delta_{sj}}{\omega-(\epsilon_j+\epsilon_i+2\mathrm{i}\eta)}-\sum_{ab}\frac{\delta_{pb}\delta_{qa}\delta_{ra}\delta_{sb}}{\omega-(\epsilon_a+\epsilon_b-2\mathrm{i}\eta)}\right].\end{aligned} \tag{29}$$

Therefore, $K_0$ has the following antisymmetric properties $(K_0)_{pqrs} = -(K_0)_{qprs} = -(K_0)_{pqsr} = (K_0)_{qpsr}$, which can be used to reduce the size of the space that one must consider. The two-electron basis set $\{\varphi_p(\mathbf{x}_1)\varphi_q(\mathbf{x}_2)\}_{\{p,q\}\in[1,N]^2}$ (where $N$ is the size of the basis set) is recast as

$$\left\{\frac{\varphi_p(\mathbf{x}_1)\varphi_q(\mathbf{x}_2)-\varphi_q(\mathbf{x}_1)\varphi_p(\mathbf{x}_2)}{\sqrt{2}}\right\}_{p<q,q\in[1,N]}\bigcup\{\varphi_p(\mathbf{x}_1)\varphi_p(\mathbf{x}_2)\}_{p\in[1,N]}\bigcup\left\{\frac{\varphi_p(\mathbf{x}_1)\varphi_q(\mathbf{x}_2)+\varphi_q(\mathbf{x}_1)\varphi_p(\mathbf{x}_2)}{\sqrt{2}}\right\}_{p<q,q\in[1,N]}. \tag{30}$$

In other words, the basis set is decomposed into its antisymmetric and symmetric parts. Because of its antisymmetric nature, the non-interacting pp propagator is non-zero only in the first subset and the corresponding elements are $(\bar{K}_0)_{pqrs} = 2(K_0)_{pqrs}$. Note that in this subset we have $p < q$ and $r < s$. Hence, due to these restrictions on $p$, $q$, $r$, and $s$, only the second term in Eq. (29) is non-zero and the matrix elements in the antisymmetric basis are

$$(\bar{K}_0)_{pqrs}(\omega) = \mathrm{i}\sum_{i<j}\frac{\delta_{ri}\delta_{sj}\delta_{pi}\delta_{qj}}{\omega-(\epsilon_i+\epsilon_j+2\mathrm{i}\eta)}-\mathrm{i}\sum_{a<b}\frac{\delta_{ra}\delta_{sb}\delta_{pa}\delta_{qb}}{\omega-(\epsilon_a+\epsilon_b-2\mathrm{i}\eta)}. \tag{31}$$

In the following, we drop the bar symbol and remain in the antisymmetrized basis set. The corresponding matrix reads

$$(\boldsymbol{K}_0)^{-1} = \begin{pmatrix}(K_0)_{ab,ab} & \mathbf{0}\\ \mathbf{0} & (K_0)_{ij,ij}\end{pmatrix}^{-1} = \begin{pmatrix}\mathrm{i}\,\mathrm{diag}[\omega-(\epsilon_a+\epsilon_b)] & \mathbf{0}\\ \mathbf{0} & \mathrm{i}\,\mathrm{diag}[(\epsilon_i+\epsilon_j)-\omega]\end{pmatrix}, \tag{32}$$

where $\mathrm{diag}(\epsilon_p)$ is a diagonal matrix with elements $\epsilon_p$.

### B. Eigenvalue problem

The aim of this subsection is to show that finding the poles of $\boldsymbol{K}(\omega)$ is equivalent to solving an eigenvalue problem. The matrix equation for the inverse pp propagator can be recast as

$$\begin{aligned}\boldsymbol{K}^{-1}(\omega) &= \boldsymbol{K}_0^{-1}(\omega)+\tilde{\boldsymbol{\Xi}}(\omega) = \mathrm{i}\begin{pmatrix}\boldsymbol{\omega} & \mathbf{0}\\ \mathbf{0} & -\boldsymbol{\omega}\end{pmatrix}+\mathrm{i}\begin{pmatrix}-\boldsymbol{\epsilon}_{ab} & \mathbf{0}\\ \mathbf{0} & \boldsymbol{\epsilon}_{ij}\end{pmatrix}+\tilde{\boldsymbol{\Xi}}(\omega)\\ &= \mathrm{i}\left[\begin{pmatrix}\boldsymbol{\omega} & \mathbf{0}\\ \mathbf{0} & -\boldsymbol{\omega}\end{pmatrix}-\begin{pmatrix}\boldsymbol{\epsilon}_{ab} & \mathbf{0}\\ \mathbf{0} & -\boldsymbol{\epsilon}_{ij}\end{pmatrix}-\mathrm{i}\tilde{\boldsymbol{\Xi}}(\omega)\right] = -\mathrm{i}\boldsymbol{\mathcal{M}}\cdot[\boldsymbol{\mathcal{H}}(\omega)-\omega\mathbf{1}],\end{aligned}$$

where $\boldsymbol{\epsilon}_{ij} = \mathrm{diag}(\epsilon_i+\epsilon_j)$, $\boldsymbol{\epsilon}_{ab} = \mathrm{diag}(\epsilon_a+\epsilon_b)$, and $\boldsymbol{\omega} = \omega\mathbf{1}$. The metric $\boldsymbol{\mathcal{M}}$ and the dynamic Hamiltonian matrix $\boldsymbol{\mathcal{H}}(\omega)$ are defined as

$$\boldsymbol{\mathcal{M}} = \begin{pmatrix}\mathbf{1} & \mathbf{0}\\ \mathbf{0} & -\mathbf{1}\end{pmatrix}, \qquad \boldsymbol{\mathcal{H}}(\omega) = \begin{pmatrix}\boldsymbol{C}(\omega) & \boldsymbol{B}\\ -\boldsymbol{B}^\dagger & -\boldsymbol{D}(-\omega)\end{pmatrix}, \tag{33}$$

and the latter can be decomposed as $\boldsymbol{\mathcal{R}}(\omega)\cdot\boldsymbol{\mathcal{E}}(\omega)\cdot\boldsymbol{\mathcal{L}}^\dagger(\omega)$, where the diagonal matrix $\boldsymbol{\mathcal{E}}(\omega)$ gathers the (frequency-dependent) eigenvalues and the left and right eigenvectors are given by

$$\boldsymbol{\mathcal{H}}(\omega)\cdot\boldsymbol{\mathcal{R}}(\omega) = \boldsymbol{\mathcal{R}}(\omega)\cdot\boldsymbol{\mathcal{E}}(\omega), \qquad \boldsymbol{\mathcal{H}}^\dagger(\omega)\cdot\boldsymbol{\mathcal{L}}(\omega) = \boldsymbol{\mathcal{L}}(\omega)\cdot\boldsymbol{\mathcal{E}}(\omega), \tag{34}$$

and fulfil the orthonormality condition $\boldsymbol{\mathcal{L}}^\dagger(\omega) \cdot \boldsymbol{\mathcal{R}}(\omega) = \mathbf{1}$. The blocks of $\boldsymbol{\mathcal{H}}(\omega)$ are given by

$$C_{ab,cd}(\omega) = (\epsilon_a + \epsilon_b)\delta_{ac}\delta_{bd} + \mathrm{i}\tilde{\Xi}^{\mathrm{pp}}_{ab,cd}(\omega), \tag{35a}$$

$$B_{ab,ij}(\omega) = +\mathrm{i}\tilde{\Xi}^{\mathrm{pp}}_{ab,ij}, \tag{35b}$$

$$D_{ij,kl}(-\omega) = -(\epsilon_i + \epsilon_j)\delta_{ik}\delta_{jl} + \mathrm{i}\tilde{\Xi}^{\mathrm{pp}}_{ij,kl}(-\omega), \tag{35c}$$

with the following restrictions on the indices $i < j$, $k < l$, $a < b$, and $c < d$. Remember that $\tilde{\Xi}^{\mathrm{pp}}_{pq,rs}(\omega)$ are the matrix elements in the antisymmetrized basis sets. (In addition, note that $\tilde{\Xi}^{\mathrm{pp}}_{ab,ij}$ is, in general, frequency-dependent. However, for every kernel considered in this work, this coupling block is found to be static.) These three blocks will be referred to as the hh-hh, hh-ee, and ee-ee blocks, respectively.

Using the eigenvalue decomposition of $\boldsymbol{\mathcal{H}}(\omega)$, $\boldsymbol{K}^{-1}(\omega)$ can be written as

$$\boldsymbol{K}^{-1}(\omega) = -\mathrm{i}\boldsymbol{\mathcal{M}} \cdot \boldsymbol{\mathcal{R}}(\omega) \cdot [\boldsymbol{\mathcal{E}}(\omega) - \omega\mathbf{1}] \cdot \boldsymbol{\mathcal{L}}^\dagger(\omega).$$

Thus, the pp propagator is

$$\boldsymbol{K}(\omega) = \mathrm{i}\boldsymbol{\mathcal{R}}(\omega) \cdot [\boldsymbol{\mathcal{E}}(\omega) - \omega\mathbf{1}]^{-1} \cdot \boldsymbol{\mathcal{L}}^\dagger(\omega) \cdot \boldsymbol{\mathcal{M}}, \tag{36}$$

and its poles are obtained through the non-linear eigenvalue problem

$$\begin{pmatrix} \boldsymbol{C}(\omega) & \boldsymbol{B} \\ \boldsymbol{B}^\dagger & \boldsymbol{D}(-\omega) \end{pmatrix} \cdot \begin{pmatrix} \boldsymbol{X} \\ \boldsymbol{Y} \end{pmatrix} = \omega \begin{pmatrix} \mathbf{1} & \mathbf{0} \\ \mathbf{0} & -\mathbf{1} \end{pmatrix} \cdot \begin{pmatrix} \boldsymbol{X} \\ \boldsymbol{Y} \end{pmatrix}, \tag{37}$$

which determines $\boldsymbol{\mathcal{E}}(\omega)$. Therefore, to solve this problem, one must find the $\omega$ values such that $\omega$ is an eigenvalue of the $\omega$-dependent matrix $\boldsymbol{\mathcal{H}}(\omega)$.

### C. Kernel matrix elements

Now that the eigenvalue equation has been derived, the last missing ingredient is the expression of the dynamic kernel matrix elements. The projection in a basis set of Eq. (19) yields

$$\begin{aligned} \tilde{\Xi}^{\mathrm{pp}}_{pq,rs}(\omega) &= \frac{1}{(2\pi)^2} \int \mathrm{d}(\tilde{\omega}\bar{\omega})\, (K_0^{-1})_{pq,\mu}(\omega)(K_0)_{\mu,\nu}(\tilde{\omega},\omega)\Xi^{\mathrm{pp}}_{\nu,\lambda}(-\tilde{\omega},-\bar{\omega},\omega)(K_0)_{\lambda,\sigma}(\bar{\omega},\omega)(K_0^{-1})_{\sigma,rs}(\omega) \\ &= \frac{1}{(2\pi)^2} \int \mathrm{d}(\tilde{\omega}\bar{\omega})\, (K_0^{-1})_{pq,pq}(\omega)(K_0)_{pq,\nu}(\tilde{\omega},\omega)\Xi^{\mathrm{pp}}_{\nu,\lambda}(-\tilde{\omega},-\bar{\omega},\omega)(K_0)_{\lambda,rs}(\bar{\omega},\omega)(K_0^{-1})_{rs,rs}(\omega) \end{aligned} \tag{38}$$

where the simplification of the second line comes from the diagonal structure of $K_0$ [see Eq. (32)]. As can be readily seen, the two-frequency non-interacting pp propagators matrix elements have to be computed first. Once again, the non-interacting propagator is decomposed in two terms

$$\begin{aligned} K_0(\mathbf{x}_1\mathbf{x}_2;\mathbf{x}_{1'}\mathbf{x}_{2'};\tilde{\omega},\omega) &= K_0^{\mathrm{I}}(\mathbf{x}_1\mathbf{x}_2;\mathbf{x}_{1'}\mathbf{x}_{2'};\tilde{\omega},\omega) + K_0^{\mathrm{II}}(\mathbf{x}_1\mathbf{x}_2;\mathbf{x}_{1'}\mathbf{x}_{2'};\tilde{\omega},\omega) \\ &= \frac{e^{-\mathrm{i}\eta\tilde{\omega}}}{2} G(\mathbf{x}_1\mathbf{x}_{1'};\frac{\omega}{2}+\tilde{\omega})G(\mathbf{x}_2\mathbf{x}_{2'};\frac{\omega}{2}-\tilde{\omega}) - \frac{e^{\mathrm{i}\eta\tilde{\omega}}}{2} G(\mathbf{x}_2\mathbf{x}_{1'};\frac{\omega}{2}-\tilde{\omega})G(\mathbf{x}_1\mathbf{x}_{2'};\frac{\omega}{2}+\tilde{\omega}). \end{aligned} \tag{39}$$

The second term can be computed as

$$K_0^{\mathrm{II}}(\mathbf{x}_1\mathbf{x}_2;\mathbf{x}_{1'}\mathbf{x}_{2'};\tilde{\omega},\omega) = -\frac{1}{2}e^{\mathrm{i}\eta\tilde{\omega}}G(\mathbf{x}_2\mathbf{x}_{1'};\frac{\omega}{2}-\tilde{\omega})G(\mathbf{x}_1\mathbf{x}_{2'};\frac{\omega}{2}+\tilde{\omega})$$
$$= -\frac{1}{2}e^{\mathrm{i}\eta\tilde{\omega}}\left[\sum_i \frac{\varphi_i(\mathbf{x}_2)\varphi_i^*(\mathbf{x}_{1'})}{\frac{\omega}{2}-\tilde{\omega}-(\epsilon_i+\mathrm{i}\eta)} + \sum_a \frac{\varphi_a(\mathbf{x}_2)\varphi_a^*(\mathbf{x}_{1'})}{\frac{\omega}{2}-\tilde{\omega}-(\epsilon_a-\mathrm{i}\eta)}\right]\left[\sum_j \frac{\varphi_j(\mathbf{x}_1)\varphi_j^*(\mathbf{x}_{2'})}{\frac{\omega}{2}+\tilde{\omega}-(\epsilon_j+\mathrm{i}\eta)} + \sum_b \frac{\varphi_b(\mathbf{x}_1)\varphi_b^*(\mathbf{x}_{2'})}{\frac{\omega}{2}+\tilde{\omega}-(\epsilon_b-\mathrm{i}\eta)}\right]$$
$$= \frac{1}{2}e^{\mathrm{i}\eta\tilde{\omega}}\left[\sum_i \frac{\varphi_i(\mathbf{x}_2)\varphi_i^*(\mathbf{x}_{1'})}{\tilde{\omega}-\left(\frac{\omega}{2}-\epsilon_i-\mathrm{i}\eta\right)} + \sum_a \frac{\varphi_a(\mathbf{x}_2)\varphi_a^*(\mathbf{x}_{1'})}{\tilde{\omega}-\left(\frac{\omega}{2}-\epsilon_a+\mathrm{i}\eta\right)}\right]\left[\sum_j \frac{\varphi_j(\mathbf{x}_1)\varphi_j^*(\mathbf{x}_{2'})}{\tilde{\omega}-\left(\epsilon_j-\frac{\omega}{2}+\mathrm{i}\eta\right)} + \sum_b \frac{\varphi_b(\mathbf{x}_1)\varphi_b^*(\mathbf{x}_{2'})}{\tilde{\omega}-\left(\epsilon_b-\frac{\omega}{2}-\mathrm{i}\eta\right)}\right]$$
$$= \frac{1}{2}e^{\mathrm{i}\eta\tilde{\omega}}\sum_{ij}\frac{\varphi_i(\mathbf{x}_2)\varphi_i^*(\mathbf{x}_{1'})\varphi_j(\mathbf{x}_1)\varphi_j^*(\mathbf{x}_{2'})}{\omega-\epsilon_i-\epsilon_j-2\mathrm{i}\eta}\left[\frac{1}{\tilde{\omega}-\left(\frac{\omega}{2}-\epsilon_i-\mathrm{i}\eta\right)} - \frac{1}{\tilde{\omega}-\left(\epsilon_j-\frac{\omega}{2}+\mathrm{i}\eta\right)}\right]$$
$$+ \frac{1}{2}e^{\mathrm{i}\eta\tilde{\omega}}\sum_{ib}\frac{\varphi_i(\mathbf{x}_2)\varphi_i^*(\mathbf{x}_{1'})\varphi_b(\mathbf{x}_1)\varphi_b^*(\mathbf{x}_{2'})}{\omega-\epsilon_i-\epsilon_b}\left[\frac{1}{\tilde{\omega}-\left(\frac{\omega}{2}-\epsilon_i-\mathrm{i}\eta\right)} - \frac{1}{\tilde{\omega}-\left(\epsilon_b-\frac{\omega}{2}-\mathrm{i}\eta\right)}\right]$$
$$+ \frac{1}{2}e^{\mathrm{i}\eta\tilde{\omega}}\sum_{aj}\frac{\varphi_a(\mathbf{x}_2)\varphi_a^*(\mathbf{x}_{1'})\varphi_j(\mathbf{x}_1)\varphi_j^*(\mathbf{x}_{2'})}{\omega-\epsilon_a-\epsilon_j}\left[\frac{1}{\tilde{\omega}-\left(\frac{\omega}{2}-\epsilon_a+\mathrm{i}\eta\right)} - \frac{1}{\tilde{\omega}-\left(\epsilon_j-\frac{\omega}{2}+\mathrm{i}\eta\right)}\right]$$
$$+ \frac{1}{2}e^{\mathrm{i}\eta\tilde{\omega}}\sum_{ab}\frac{\varphi_a(\mathbf{x}_2)\varphi_a^*(\mathbf{x}_{1'})\varphi_b(\mathbf{x}_1)\varphi_b^*(\mathbf{x}_{2'})}{\omega-\epsilon_a-\epsilon_b+2\mathrm{i}\eta}\left[\frac{1}{\tilde{\omega}-\left(\frac{\omega}{2}-\epsilon_a+\mathrm{i}\eta\right)} - \frac{1}{\tilde{\omega}-\left(\epsilon_b-\frac{\omega}{2}-\mathrm{i}\eta\right)}\right],$$

where we have used the well-known identity

$$\frac{1}{(\omega-a)(\omega-b)} = \frac{1}{a-b}\left(\frac{1}{\omega-a}-\frac{1}{\omega-b}\right).$$

The second term is computed in a very similar way and the final expression combining both terms is

$$(K_0)(\mathbf{x}_1\mathbf{x}_2;\mathbf{x}_{1'}\mathbf{x}_{2'};\tilde{\omega},-\eta,\omega) =$$
$$-\frac{1}{2}\sum_{ij}\frac{e^{-\mathrm{i}\eta\tilde{\omega}}\varphi_i(\mathbf{x}_2)\varphi_i^*(\mathbf{x}_{2'})\varphi_j(\mathbf{x}_1)\varphi_j^*(\mathbf{x}_{1'}) - e^{\mathrm{i}\eta\tilde{\omega}}\varphi_i(\mathbf{x}_2)\varphi_i^*(\mathbf{x}_{1'})\varphi_j(\mathbf{x}_1)\varphi_j^*(\mathbf{x}_{2'})}{\omega-\epsilon_i-\epsilon_j-2\mathrm{i}\eta}\left[\frac{1}{\tilde{\omega}-\left(\frac{\omega}{2}-\epsilon_i-\mathrm{i}\eta\right)} - \frac{1}{\tilde{\omega}-\left(\epsilon_j-\frac{\omega}{2}+\mathrm{i}\eta\right)}\right]$$
$$-\frac{1}{2}\sum_{ib}\frac{e^{-\mathrm{i}\eta\tilde{\omega}}\varphi_i(\mathbf{x}_2)\varphi_i^*(\mathbf{x}_{2'})\varphi_b(\mathbf{x}_1)\varphi_b^*(\mathbf{x}_{1'}) - e^{\mathrm{i}\eta\tilde{\omega}}\varphi_i(\mathbf{x}_2)\varphi_i^*(\mathbf{x}_{1'})\varphi_b(\mathbf{x}_1)\varphi_b^*(\mathbf{x}_{2'})}{\omega-\epsilon_i-\epsilon_b}\left[\frac{1}{\tilde{\omega}-\left(\frac{\omega}{2}-\epsilon_i-\mathrm{i}\eta\right)} - \frac{1}{\tilde{\omega}-\left(\epsilon_b-\frac{\omega}{2}-\mathrm{i}\eta\right)}\right]$$
$$-\frac{1}{2}\sum_{aj}\frac{e^{-\mathrm{i}\eta\tilde{\omega}}\varphi_a(\mathbf{x}_2)\varphi_a^*(\mathbf{x}_{2'})\varphi_j(\mathbf{x}_1)\varphi_j^*(\mathbf{x}_{1'}) - e^{\mathrm{i}\eta\tilde{\omega}}\varphi_a(\mathbf{x}_2)\varphi_a^*(\mathbf{x}_{1'})\varphi_j(\mathbf{x}_1)\varphi_j^*(\mathbf{x}_{2'})}{\omega-\epsilon_a-\epsilon_j}\left[\frac{1}{\tilde{\omega}-\left(\frac{\omega}{2}-\epsilon_a+\mathrm{i}\eta\right)} - \frac{1}{\tilde{\omega}-\left(\epsilon_j-\frac{\omega}{2}+\mathrm{i}\eta\right)}\right]$$
$$-\frac{1}{2}\sum_{ab}\frac{e^{-\mathrm{i}\eta\tilde{\omega}}\varphi_a(\mathbf{x}_2)\varphi_a^*(\mathbf{x}_{2'})\varphi_b(\mathbf{x}_1)\varphi_b^*(\mathbf{x}_{1'}) - e^{\mathrm{i}\eta\tilde{\omega}}\varphi_a(\mathbf{x}_2)\varphi_a^*(\mathbf{x}_{1'})\varphi_b(\mathbf{x}_1)\varphi_b^*(\mathbf{x}_{2'})}{\omega-\epsilon_a-\epsilon_b+2\mathrm{i}\eta}\left[\frac{1}{\tilde{\omega}-\left(\frac{\omega}{2}-\epsilon_a+\mathrm{i}\eta\right)} - \frac{1}{\tilde{\omega}-\left(\epsilon_b-\frac{\omega}{2}-\mathrm{i}\eta\right)}\right].$$

Once projected in the antisymmetrized basis, $(K_0)(\mathbf{x}_1\mathbf{x}_2;\mathbf{x}_{1'}\mathbf{x}_{2'};\tilde{\omega},-\eta,\omega)$ becomes

$$(K_0)_{pq,rs}(\tilde{\omega},-\eta,\omega) = -e^{-\mathrm{i}\eta\tilde{\omega}}\sum_{j<i}\frac{\delta_{pj}\delta_{qi}\delta_{rj}\delta_{si}}{\omega-\epsilon_i-\epsilon_j-2\mathrm{i}\eta}\left[\frac{1}{\tilde{\omega}-\left(\frac{\omega}{2}-\epsilon_i-\mathrm{i}\eta\right)} - \frac{1}{\tilde{\omega}-\left(\epsilon_j-\frac{\omega}{2}+\mathrm{i}\eta\right)}\right]$$
$$- e^{-\mathrm{i}\eta\tilde{\omega}}\sum_{bi}\frac{\delta_{pb}\delta_{qi}\delta_{rb}\delta_{si}}{\omega-\epsilon_i-\epsilon_b-2\mathrm{i}\eta}\left[\frac{1}{\tilde{\omega}-\left(\frac{\omega}{2}-\epsilon_i-\mathrm{i}\eta\right)} - \frac{1}{\tilde{\omega}-\left(\epsilon_b-\frac{\omega}{2}-\mathrm{i}\eta\right)}\right]$$
$$- e^{-\mathrm{i}\eta\tilde{\omega}}\sum_{ja}\frac{\delta_{pj}\delta_{qa}\delta_{rj}\delta_{sa}}{\omega-\epsilon_a-\epsilon_j+2\mathrm{i}\eta}\left[\frac{1}{\tilde{\omega}-\left(\frac{\omega}{2}-\epsilon_a+\mathrm{i}\eta\right)} - \frac{1}{\tilde{\omega}-\left(\epsilon_j-\frac{\omega}{2}+\mathrm{i}\eta\right)}\right]$$
$$- e^{-\mathrm{i}\eta\tilde{\omega}}\sum_{b<a}\frac{\delta_{pb}\delta_{qa}\delta_{rb}\delta_{sa}}{\omega-\epsilon_a-\epsilon_b+2\mathrm{i}\eta}\left[\frac{1}{\tilde{\omega}-\left(\frac{\omega}{2}-\epsilon_a+\mathrm{i}\eta\right)} - \frac{1}{\tilde{\omega}-\left(\epsilon_b-\frac{\omega}{2}-\mathrm{i}\eta\right)}\right].$$

This shows that the two-frequency propagator is diagonal. Because of this diagonal structure, only $(K_0)_{ji,ji}(\tilde{\omega}, -\eta, \omega)$ and $(K_0)_{ba,ba}(\tilde{\omega}, -\eta, \omega)$ are required to compute $\tilde{\Xi}^{\text{pp}}_{pq,rs}(\omega)$. Using Eq. (31), these matrix elements can be recast as

$$(K_0)_{ji,ji}(\tilde{\omega}, -\eta, \omega) = +\text{i}e^{-\text{i}\eta\tilde{\omega}}(K_0)_{ji,ji}(\omega)\left[\frac{1}{\tilde{\omega} - \left(\frac{\omega}{2} - \epsilon_i - \text{i}\eta\right)} - \frac{1}{\tilde{\omega} - \left(\epsilon_j - \frac{\omega}{2} + \text{i}\eta\right)}\right] \tag{40}$$

$$(K_0)_{ba,ba}(\tilde{\omega}, -\eta, \omega) = -\text{i}e^{-\text{i}\eta\tilde{\omega}}(K_0)_{ba,ba}(\omega)\left[\frac{1}{\tilde{\omega} - \left(\frac{\omega}{2} - \epsilon_a + \text{i}\eta\right)} - \frac{1}{\tilde{\omega} - \left(\epsilon_b - \frac{\omega}{2} - \text{i}\eta\right)}\right]. \tag{41}$$

This factorization is particularly convenient as it greatly simplifies the expression of the dynamic kernel. For example, the ee-ee block of the kernel reads

$$\begin{aligned}
\tilde{\Xi}^{\text{pp}}_{ij,kl}(\omega) &= \frac{1}{(2\pi)^2}\int \text{d}(\tilde{\omega}\bar{\omega})\,(K_0^{-1})_{ij,ij}(\omega)(K_0)_{ij,ij}(-\eta,\tilde{\omega},\omega)\Xi^{\text{pp}}_{ij,kl}(-\tilde{\omega},-\bar{\omega},\omega)(K_0)_{kl,kl}(\bar{\omega},-\eta,\omega)(K_0^{-1})_{kl,kl}(\omega)\\
&= \frac{1}{(2\pi)^2}\int \text{d}(\tilde{\omega}\bar{\omega})\,(K_0^{-1})_{ij,ij}(\omega)\text{i}e^{-\text{i}\eta\tilde{\omega}}(K_0)_{ij,ij}(\omega)\left[\frac{1}{\tilde{\omega} - \left(\frac{\omega}{2} - \epsilon_j - \text{i}\eta\right)} - \frac{1}{\tilde{\omega} - \left(\epsilon_i - \frac{\omega}{2} + \text{i}\eta\right)}\right]\\
&\qquad\times\Xi^{\text{pp}}_{ij,kl}(-\tilde{\omega},-\bar{\omega},\omega)(K_0)_{kl,kl}(\bar{\omega},-\eta,\omega)(K_0^{-1})_{kl,kl}(\omega)\\
&= \frac{\text{i}}{(2\pi)^2}\int \text{d}(\tilde{\omega}\bar{\omega})\,e^{-\text{i}\eta\tilde{\omega}}\left[\frac{1}{\tilde{\omega} - \left(\frac{\omega}{2} - \epsilon_j - \text{i}\eta\right)} - \frac{1}{\tilde{\omega} - \left(\epsilon_i - \frac{\omega}{2} + \text{i}\eta\right)}\right]\\
&\qquad\times\Xi^{\text{pp}}_{ij,kl}(-\tilde{\omega},-\bar{\omega},\omega)(K_0)_{kl,kl}(\bar{\omega},-\eta,\omega)(K_0^{-1})_{kl,kl}(\omega)\\
&= \frac{\text{i}}{(2\pi)^2}\int \text{d}(\tilde{\omega}\bar{\omega})\,e^{-\text{i}\eta\tilde{\omega}}\left[\frac{1}{\tilde{\omega} - \left(\frac{\omega}{2} - \epsilon_j - \text{i}\eta\right)} - \frac{1}{\tilde{\omega} - \left(\epsilon_i - \frac{\omega}{2} + \text{i}\eta\right)}\right]\\
&\qquad\times\Xi^{\text{pp}}_{ij,kl}(-\tilde{\omega},-\bar{\omega},\omega)\text{i}e^{-\text{i}\eta\bar{\omega}}\left[\frac{1}{\bar{\omega} - \left(\frac{\omega}{2} - \epsilon_l - \text{i}\eta\right)} - \frac{1}{\bar{\omega} - \left(\epsilon_k - \frac{\omega}{2} + \text{i}\eta\right)}\right](K_0)_{kl,kl}(\omega)(K_0^{-1})_{kl,kl}(\omega)\\
&= \frac{\text{i}^2}{(2\pi)^2}\int \text{d}(\tilde{\omega}\bar{\omega})\,e^{-\text{i}\eta\tilde{\omega}}\left[\frac{1}{\tilde{\omega} - \left(\frac{\omega}{2} - \epsilon_j - \text{i}\eta\right)} - \frac{1}{\tilde{\omega} - \left(\epsilon_i - \frac{\omega}{2} + \text{i}\eta\right)}\right]\\
&\qquad\times\Xi^{\text{pp}}_{ij,kl}(-\tilde{\omega},-\bar{\omega},\omega)e^{-\text{i}\eta\bar{\omega}}\left[\frac{1}{\bar{\omega} - \left(\frac{\omega}{2} - \epsilon_l - \text{i}\eta\right)} - \frac{1}{\bar{\omega} - \left(\epsilon_k - \frac{\omega}{2} + \text{i}\eta\right)}\right]
\end{aligned} \tag{42}$$

If the kernel is static, *i.e.*, $\Xi^{\text{pp}}_{pq,rs}(\tilde{\omega}, \bar{\omega}, \omega) = \Xi^{\text{pp}}_{pq,rs}$, then the integral is evaluated as

$$\begin{aligned}
\tilde{\Xi}^{\text{pp}}_{ij,kl}(\omega) &= \frac{\text{i}^2}{(2\pi)^2}\Xi^{\text{pp}}_{ij,kl}\left\{\int \text{d}\tilde{\omega}\,e^{-\text{i}\eta\tilde{\omega}}\left[\frac{1}{\tilde{\omega} - \left(\frac{\omega}{2} - \epsilon_j - \text{i}\eta\right)} - \frac{1}{\tilde{\omega} - \left(\epsilon_i - \frac{\omega}{2} + \text{i}\eta\right)}\right]\right\}\\
&\qquad\times\left\{\int \text{d}\bar{\omega}\,e^{-\text{i}\eta\bar{\omega}}\left[\frac{1}{\bar{\omega} - \left(\frac{\omega}{2} - \epsilon_l - \text{i}\eta\right)} - \frac{1}{\bar{\omega} - \left(\epsilon_k - \frac{\omega}{2} + \text{i}\eta\right)}\right]\right\}\\
&= \Xi^{\text{pp}}_{ij,kl}.
\end{aligned} \tag{43}$$

This means that the approximate dynamic kernel $\tilde{\Xi}^{\text{pp}}$ reduces to the static one.

On the other hand, if one wishes to use a dynamic kernel $\Xi^{\text{pp}}_{pq,rs}(\tilde{\omega}, \bar{\omega}, \omega)$, the corresponding integrals have to be evaluated to obtain $\tilde{\Xi}^{\text{pp}}_{pq,rs}(\omega)$. This will be done in Sec. VI. To conclude this section, we report, for the sake of completeness, the hh-hh and hh-ee matrix elements of the effective dynamic kernel

$$\begin{aligned}
\tilde{\Xi}^{\text{pp}}_{ab,cd}(\omega) &= \frac{(-\text{i})^2}{(2\pi)^2}\int \text{d}(\tilde{\omega}\bar{\omega})\,e^{-\text{i}\eta\tilde{\omega}}\left[\frac{1}{\tilde{\omega} - \left(\frac{\omega}{2} - \epsilon_b + \text{i}\eta\right)} - \frac{1}{\tilde{\omega} - \left(\epsilon_a - \frac{\omega}{2} - \text{i}\eta\right)}\right]\\
&\qquad\times\Xi^{\text{pp}}_{ab,cd}(-\tilde{\omega},-\bar{\omega},\omega)e^{-\text{i}\eta\bar{\omega}}\left[\frac{1}{\bar{\omega} - \left(\frac{\omega}{2} - \epsilon_d + \text{i}\eta\right)} - \frac{1}{\bar{\omega} - \left(\epsilon_c - \frac{\omega}{2} - \text{i}\eta\right)}\right],
\end{aligned} \tag{44}$$

and

$$\tilde{\Xi}^{\text{pp}}_{ab,ij}(\omega) = \frac{-\mathrm{i}^2}{(2\pi)^2} \int \mathrm{d}(\tilde{\omega}\bar{\omega})\, e^{-\mathrm{i}\eta\tilde{\omega}} \left[ \frac{1}{\tilde{\omega} - \left(\frac{\omega}{2} - \epsilon_b + \mathrm{i}\eta\right)} - \frac{1}{\tilde{\omega} - \left(\epsilon_a - \frac{\omega}{2} - \mathrm{i}\eta\right)} \right] \times \Xi^{\text{pp}}_{ab,ij}(-\tilde{\omega}, -\bar{\omega}, \omega) e^{-\mathrm{i}\eta\bar{\omega}} \left[ \frac{1}{\bar{\omega} - \left(\frac{\omega}{2} - \epsilon_j - \mathrm{i}\eta\right)} - \frac{1}{\bar{\omega} - \left(\epsilon_i - \frac{\omega}{2} + \mathrm{i}\eta\right)} \right]. \tag{45}$$

## IV. KERNEL APPROXIMATIONS

In this section, the kernel [see Eq. (10)] corresponding to various self-energy approximations are computed.

### A. First-order Coulomb kernel

The simplest anomalous self-energy is the static Bogoliubov (B)

$$\Sigma^{\text{ee,B}}(11') = -\mathrm{i}v(33'^{+}; 11'^{++}) G^{\text{ee}}(33'), \tag{46}$$

which is of first order in the Coulomb interaction $v$. The corresponding kernel is easily computed as

$$\begin{aligned} \Xi^{\text{pp,B}}(22'; 11') &= -\mathrm{i}v(33'^{+}; 11'^{++}) \left. \frac{\delta G^{\text{ee}}(33')}{\delta G^{\text{ee}}(22')} \right|_{U=0} \\ &= -\frac{\mathrm{i}}{2} v(33'^{+}; 11'^{++})[\delta(32)\delta(3'2') - \delta(32')\delta(3'2)] \\ &= -\frac{\mathrm{i}}{2}[v(22'^{+}; 11'^{++}) - v(2'2^{+}; 11'^{++})] \\ &= -\frac{\mathrm{i}}{2}\bar{v}(22'; 11'). \end{aligned} \tag{47}$$

where we have introduced $\bar{v}(22'; 11') = v(22'; 11') - v(2'2; 11')$. Hence, this kernel is recognized to be the antisymmetric Coulomb interaction. The corresponding diagrammatic representation of the pp-BSE is represented in Fig. 2.

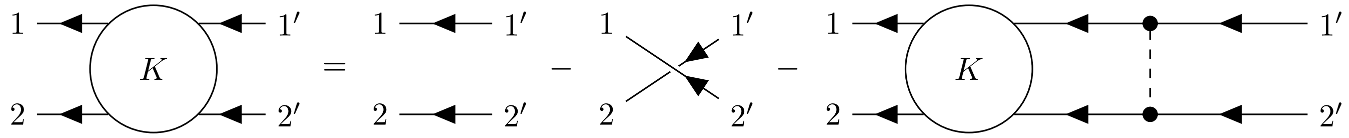


FIG. 2. Diagrammatic representation of the pp-BSE with a first-order Coulomb kernel. The dashed line represents the Coulomb interaction while the solid lines correspond to one-body propagators.

### B. *GW* kernel

By extending the conventional Hedin equations to the case of the Gorkov propagator, one can derive a *GW* approximation for the Nambu self-energy (see Appendix A). In particular, the ee component reads

$$\Sigma^{\text{ee},GW}(11') = -\mathrm{i}W(33'; 11') G^{\text{ee}}(33'). \tag{48}$$

In this case, $W$ is a generalized screened interaction that accounts for anomalous bubbles as well (see Fig. 7). This effective interaction reduces to the usual pp-RPA screened interaction in the normal phase limit. The corresponding kernel is derived as

$$\begin{aligned} \Xi^{\text{pp},GW}(22'; 11') &= -\mathrm{i}W(33'; 11') \left. \frac{\delta G^{\text{ee}}(33')}{\delta G^{\text{ee}}(22')} \right|_{U=0} \\ &= -\frac{\mathrm{i}}{2} W(33'; 11')[\delta(32)\delta(3'2') - \delta(32')\delta(3'2)] \\ &= -\frac{\mathrm{i}}{2}[W(22'; 11') - W(2'2; 11')], \end{aligned} \tag{49}$$

and corresponds to a screened version of the kernel obtained using the Bogoliubov self-energy in Sec. IV A. It is interesting to note that the derivative of $W$ has not been neglected as usually done in the eh-BSE case [3–5]. Within the pp-BSE formalism, the corresponding term is exactly zero because the anomalous propagator vanishes in the normal phase.

The screened interaction is given by

$$W(33';11') = v(33';11') - \mathrm{i}v(34';14)L(42;4'2')v(2'3';21'), \tag{50}$$

where $L(12;1'2') = L_0(12;1'2') + L_0(13;1'4)v(46;35)L(52;62')$ is the eh-RPA propagator and $L_0(12;1'2') = G(12')G(21')$ is the non-interacting eh propagator.

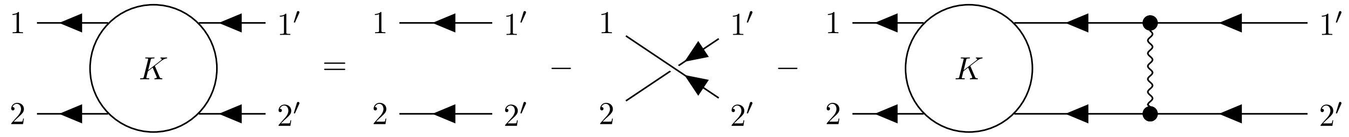


FIG. 3. Diagrammatic representations of the pp-BSE with a $GW$-based kernel. The wiggly line represents the screened interaction while the solid lines correspond to one-body propagators.

### C. Second-order Coulomb kernel

The self-energy of second-order in terms of the Coulomb interaction can be written as

$$\Sigma^{\mathrm{ee},(2)}(11') = -\mathrm{i}W^{(2)}(33';11')G^{\mathrm{ee}}(33') \tag{51}$$

where $W^{(2)}$ is an antisymmetrized interaction screened up to second-order, *i.e.*,

$$W^{(2)}(33';11') = v(33';11') - \mathrm{i}\bar{v}(34';14)L_0(42;4'2')\bar{v}(2'3';21'). \tag{52}$$

Hence, the kernel is

$$\Xi^{\mathrm{pp},(2)}(22';11') = -\frac{\mathrm{i}}{2}[W^{(2)}(22';11') - W^{(2)}(2'2;11')]. \tag{53}$$

The second-order kernel $\Xi^{\mathrm{pp},(2)}(22';11')$ has the same functional form and time dependence as the $GW$ kernel $\Xi^{\mathrm{pp},GW}(22';11')$.

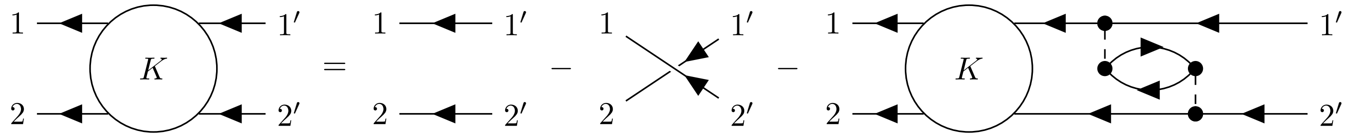


FIG. 4. Diagrammatic representation of the pp-BSE with a second-order Coulomb kernel. (The first-order diagram is not drawn.) The dashed lines represent the Coulomb interaction while the solid lines correspond to one-body propagators.

### D. $T$-matrix kernel

Finally, another usual self-energy approximation is considered, the so-called pp $T$-matrix approximation [6, 7]. This approximation has first been generalized to the Gorkov propagator by Bozek in a diagrammatic framework [8], before being derived in a functional derivative framework by some of us [1]. The self-energy approximation of interest in this context is

$$\Sigma^{\mathrm{ee},GT}(11') = \mathrm{i}G^{\mathrm{hh}}(22')T^{\mathrm{ee}}(12;2'1'), \tag{54}$$

where $T^{\mathrm{ee}}$ is the anomalous component of the generalized pp $T$-matrix. Hence, this means that the kernel associated with this self-energy is zero in the normal phase.

Using the pp Gorkov-Hedin equations [1], one can derive self-energy approximations of higher order in $T$ through vertex corrections. The self-energies employed to derive approximate kernels that do not vanish in the normal phase must be composed by a single anomalous propagator. One example of such self-energy is produced during the first iteration of Hedin's self-consistency procedure, as performed in Ref. 1

$$\Sigma^{\text{ee},G_3T_2}(11') = (-i)^2 T(34';14) G(4^{--}2') G(24') T(2'3';21') G^{\text{ee}}(33'). \tag{55}$$

where

$$T(12;1'2') = -\bar{v}(12;1'2') - \mathrm{i} T(12;33') K_0(33';44') v(44';1'2') \tag{56}$$

is the usual $T$-matrix computed at the pp-RPA level. Hence, the corresponding kernel is of second order in $T$. It is interesting to note that this self-energy is exactly the same as the second-order one of Eq. (51) but with a frequency-dependent effective interaction $T$ instead of the Coulomb interaction.

Once the first-order self-energy of Eq. (46) has been added, the kernel is found to be

$$\Xi^{\text{pp},(2T)}(22';11') = -\frac{\mathrm{i}}{2}[W^{(2T)}(22';11') - W^{(2T)}(2'2;11')], \tag{57}$$

where $W^{(2T)}$ is an effective interaction analog to $W^{(2)}$, *i.e.*,

$$W^{(2T)}(22';11') = v(22';11') - \mathrm{i} T(24';14) L_0(43;4'3') T(3'2';31'). \tag{58}$$

This $T$-matrix kernel $\Xi^{\text{pp},(2T)}(22';11')$ has the same functional form as the second-order and $GW$ kernels but the time dependence is more involved because $T$ is not an instantaneous interaction. Computing the full frequency-dependent kernel $\Xi^{\text{pp},(2T)}(22';11')$ is beyond the scope of this work. However, this kernel will be computed in the approximate case where the $T$-matrix effective interaction is considered static.

## V. STATIC KERNEL APPROXIMATIONS

### A. Static first-order Coulomb kernel

The first-order kernel, *i.e.*, the one arising from $\Sigma^{\text{ee,B}}$ (see Sec. IV A), is the antisymmetrized Coulomb interaction. This kernel is static because the Coulomb interaction is instantaneous,

$$\Xi^{\text{pp,B}}(\mathbf{x}_2\mathbf{x}_{2'};\mathbf{x}_1\mathbf{x}_{1'};\tilde{\omega},\bar{\omega},\omega) = \Xi^{\text{pp,B}}(\mathbf{x}_2\mathbf{x}_{2'};\mathbf{x}_1\mathbf{x}_{1'}). \tag{59}$$

Its matrix elements in the antisymmetrized basis are

$$\Xi^{\text{pp,B}}_{pq,rs} = -\mathrm{i} \langle pq||rs\rangle . \tag{60}$$

Thus, the associated eigenvalue equation reads

$$C^{\text{RPA}}_{ab,cd} = (\epsilon_a + \epsilon_b)\delta_{ac}\delta_{bd} + \langle ab||cd\rangle , \tag{61a}$$
$$B^{\text{RPA}}_{ab,ij} = \langle ab||ij\rangle , \tag{61b}$$
$$D^{\text{RPA}}_{ij,kl} = -(\epsilon_i + \epsilon_j)\delta_{ik}\delta_{jl} + \langle ij||kl\rangle , \tag{61c}$$

where the antisymmetrized integrals are defined as $\langle pq||rs\rangle = \langle pq|rs\rangle - \langle pq|sr\rangle$ in terms of the bare two-electron integrals in the spinorbital basis

$$\langle pq|rs\rangle = \iint \frac{\varphi_p(\mathbf{x}_1)\varphi_q(\mathbf{x}_2)\varphi_r(\mathbf{x}_1)\varphi_s(\mathbf{x}_2)}{|\mathbf{r}_1 - \mathbf{r}_2|} \mathrm{d}\mathbf{x}_1 \, \mathrm{d}\mathbf{x}_2 \, . \tag{62}$$

This is the well-known pp-RPA eigenvalue problem.

### B. Static $GW$ kernel

Before projecting the $GW$ kernel (see Sec. IV B) in a basis of spinorbitals, it must be transformed to frequency space. The screened interaction is not instantaneous and its Fourier transform is obtained as

$$\begin{aligned}
&\Xi^{\text{pp},GW}(\mathbf{x}_2\mathbf{x}_{2'};\mathbf{x}_1\mathbf{x}_{1'};\tilde{\omega},\bar{\omega},\omega)\\
&= -\frac{\mathrm{i}}{2}\int \mathrm{d}(\tau_{22'}\tau_{11'}\tau_{22',11'})\, e^{\mathrm{i}(\tilde{\omega}\tau_{22'}+\bar{\omega}\tau_{11'}+\omega\tau_{22',11'})}\, [W(\mathbf{x}_2\mathbf{x}_{2'};\mathbf{x}_1\mathbf{x}_{1'};\tau_{22'},\tau_{11'},\tau_{22',11'})\\
&\qquad\qquad - W(\mathbf{x}_{2'}\mathbf{x}_2;\mathbf{x}_1\mathbf{x}_{1'};\tau_{2'2},\tau_{11'},\tau_{2'2,11'})]\\
&= -\frac{\mathrm{i}}{2}\int \mathrm{d}(\tau_{22'}\tau_{11'}\tau_{22',11'})\, e^{\mathrm{i}(\tilde{\omega}\tau_{22'}+\bar{\omega}\tau_{11'}+\omega\tau_{22',11'})}\, [\delta(\tau_{21})\delta(\tau_{2'1'})W(\mathbf{x}_2\mathbf{x}_{2'};\mathbf{x}_1\mathbf{x}_{1'};\tau_{22'})\\
&\qquad\qquad - \delta(\tau_{2'1})\delta(\tau_{21'})W(\mathbf{x}_{2'}\mathbf{x}_2;\mathbf{x}_1\mathbf{x}_{1'};\tau_{2'2})]\\
&= -\frac{\mathrm{i}}{2}\int \mathrm{d}(\tau_{11'}\tau_{22',11'})\, \Big[\delta(\tau_{2'1'})e^{\mathrm{i}(\tilde{\omega}\tau_{12'}+\bar{\omega}\tau_{11'}+\omega\tau_{2'1'})}W(\mathbf{x}_2\mathbf{x}_{2'};\mathbf{x}_1\mathbf{x}_{1'};\tau_{12'})\\
&\qquad\qquad - \delta(\tau_{2'1})e^{\mathrm{i}(\tilde{\omega}\tau_{1'2'}+\bar{\omega}\tau_{11'}+\omega\tau_{2'1})}W(\mathbf{x}_{2'}\mathbf{x}_2;\mathbf{x}_1\mathbf{x}_{1'};\tau_{2'1'})\Big]\\
&= -\frac{\mathrm{i}}{2}\int \mathrm{d}(\tau_{11'})\, \Big[e^{\mathrm{i}(\tilde{\omega}\tau_{11'}+\bar{\omega}\tau_{11'})}W(\mathbf{x}_2\mathbf{x}_{2'};\mathbf{x}_1\mathbf{x}_{1'};\tau_{11'}) - e^{\mathrm{i}(\tilde{\omega}\tau_{1'1}+\bar{\omega}\tau_{11'})}W(\mathbf{x}_{2'}\mathbf{x}_2;\mathbf{x}_1\mathbf{x}_{1'};\tau_{11'})\Big].
\end{aligned} \tag{63}$$

This finally yields a kernel that depends only on two frequencies

$$\Xi^{\text{pp},GW}(\mathbf{x}_2\mathbf{x}_{2'};\mathbf{x}_1\mathbf{x}_{1'};\tilde{\omega},\bar{\omega}) = -\frac{\mathrm{i}}{2}\left[W(\mathbf{x}_2\mathbf{x}_{2'};\mathbf{x}_1\mathbf{x}_{1'};\tilde{\omega}+\bar{\omega}) - W(\mathbf{x}_{2'}\mathbf{x}_2;\mathbf{x}_1\mathbf{x}_{1'};\bar{\omega}-\tilde{\omega})\right]. \tag{64}$$

Once projected in the antisymmetrized basis set, the above expression reads

$$\Xi^{\text{pp},GW}_{pq,rs}(\tilde{\omega},\bar{\omega},\omega) = -\frac{\mathrm{i}}{2}[W_{pqrs}(\bar{\omega}+\tilde{\omega}) + W_{pqrs}(\bar{\omega}-\tilde{\omega}) - W_{qprs}(\bar{\omega}+\tilde{\omega}) - W_{qprs}(\bar{\omega}-\tilde{\omega})]. \tag{65}$$

The static limit of this kernel corresponds to taking the zero-frequency limit, that is, $W(\omega=0)$. Therefore, the associated eigenvalue equation is

$$C^{GW}_{ab,cd} = (\epsilon_a+\epsilon_b)\delta_{ac}\delta_{bd} + \langle ab||cd\rangle + (W^{\text{c}}_{abcd} - W^{\text{c}}_{bacd}), \tag{66a}$$

$$B^{GW}_{ab,ij} = \langle ab||ij\rangle + (W^{\text{c}}_{abij} - W^{\text{c}}_{baij}), \tag{66b}$$

$$D^{GW}_{ij,kl} = -(\epsilon_i+\epsilon_j)\delta_{ik}\delta_{jl} + \langle ij||kl\rangle + (W^{\text{c}}_{ijkl} - W^{\text{c}}_{jikl}), \tag{66c}$$

where $W^{\text{c}} \equiv W^{\text{c}}(\omega=0)$ is the correlation part of $W$. Its matrix elements are given by

$$\begin{aligned}
W_{pqrs}(\omega) &= \int \mathrm{d}(\mathbf{x}_1\mathbf{x}_{1'}\mathbf{x}_2\mathbf{x}_{2'})\, \varphi^*_p(\mathbf{x}_1)\varphi^*_q(\mathbf{x}_2)W(\mathbf{x}_1\mathbf{x}_2;\mathbf{x}_{1'}\mathbf{x}_{2'};\omega)\varphi_r(\mathbf{x}_{1'})\varphi_s(\mathbf{x}_{2'})\\
&= \langle pq|rs\rangle + \sum_\mu \left[\frac{M_{pr,\mu}M^*_{sq,\mu}}{\omega-\Omega_\mu+\mathrm{i}\eta} - \frac{M^*_{rp,\mu}M_{qs,\mu}}{\omega+\Omega_\mu-\mathrm{i}\eta}\right]\\
&= \langle pq|rs\rangle + W^{\text{c}}_{pqrs}(\omega),
\end{aligned} \tag{67}$$

and the two-electron screened integrals (or transition densities) are defined as

$$M_{pq,\mu} = \sum_{ia}[X_{ia,\mu}\langle ap|iq\rangle + Y_{ia,\mu}\langle ip|aq\rangle]. \tag{68}$$

Here, $X_{ia,\mu}$ and $Y_{ia,\mu}$ are the matrix elements of the eigenvectors of the eh-RPA problem

$$\begin{pmatrix} \boldsymbol{A}^{\text{RPA}} & \boldsymbol{B}^{\text{RPA}} \\ -\boldsymbol{B}^{\text{RPA}} & -\boldsymbol{A}^{\text{RPA}} \end{pmatrix} \cdot \begin{pmatrix} \boldsymbol{X}_\mu \\ \boldsymbol{Y}_\mu \end{pmatrix} = \Omega_\mu \begin{pmatrix} \boldsymbol{X}_\mu \\ \boldsymbol{Y}_\mu \end{pmatrix} \tag{69}$$

where $\Omega_\mu$ is the associated eigenvalue. The matrix elements of the (anti)resonant block $\boldsymbol{A}^{\text{RPA}}$ and the coupling block $\boldsymbol{B}^{\text{RPA}}$ read

$$A^{\text{RPA}}_{ia,jb} = (\epsilon_a-\epsilon_i)\delta_{ij}\delta_{ab} + \langle ib|aj\rangle, \tag{70a}$$

$$B^{\text{RPA}}_{ia,jb} = \langle ij|ab\rangle. \tag{70b}$$

Finally, note that the indices of $W$ in Eq. (66) are not exactly the same as the ones reported in the main manuscript. This is because the expressions of the main manuscript are simplified under the assumption that the orbitals are real-valued.

### C. Static second-order Coulomb kernel

As mentioned in Sec. IV C, the second-order kernel has exactly the same functional form as its $GW$ counterpart. Hence, the Fourier transform and the basis set projection do not have to be performed again. This subsection is just concerned with the matrix elements of $W^{(2)}$ (which are obtained by projecting Eq. (52) in the finite basis set)

$$W^{(2)}_{pqrs}(\omega) = \langle pq|rs\rangle - \mathrm{i} \sum_{tuvw} \langle pv||rt\rangle \, (L_0)_{tuvw}(\omega) \, \langle wq||us\rangle \,, \tag{71}$$

where the matrix elements of the non-interacting eh propagator are [9]

$$(L_0)_{tuvw}(\omega) = \mathrm{i} \sum_{me} \frac{\delta_{twe}\delta_{uvm}}{\omega - (\epsilon_e - \epsilon_m - 2\mathrm{i}\eta)} - \mathrm{i} \sum_{me} \frac{\delta_{twm}\delta_{uve}}{\omega - (\epsilon_m - \epsilon_e + 2\mathrm{i}\eta)}, \tag{72}$$

where $\delta_{pqr} = \delta_{pq}\delta_{qr}$. This yields

$$\begin{aligned} W^{(2)}_{pqrs}(\omega) &= \langle pq|rs\rangle + \sum_{me} \left[ \frac{\langle pm||re\rangle \, \langle eq||ms\rangle}{\omega - (\epsilon_e - \epsilon_m - 2\mathrm{i}\eta)} - \frac{\langle pe||rm\rangle \, \langle mq||es\rangle}{\omega - (\epsilon_m - \epsilon_e + 2\mathrm{i}\eta)} \right] \\ &= \langle pq|rs\rangle + W^{\mathrm{c},(2)}_{pqrs}(\omega). \end{aligned} \tag{73}$$

Finally, within the static approximation, the elements of the various blocks are

$$C^{(2)}_{ab,cd} = (\epsilon_a + \epsilon_b)\delta_{ac}\delta_{bd} + \langle ab||cd\rangle + (W^{\mathrm{c},(2)}_{abcd} - W^{\mathrm{c},(2)}_{bacd}), \tag{74a}$$

$$B^{(2)}_{ab,ij} = \langle ab||ij\rangle + (W^{\mathrm{c},(2)}_{abij} - W^{\mathrm{c},(2)}_{baij}), \tag{74b}$$

$$D^{(2)}_{ij,kl} = -(\epsilon_i + \epsilon_j)\delta_{ik}\delta_{jl} + \langle ij||kl\rangle + (W^{\mathrm{c},(2)}_{ijkl} - W^{\mathrm{c},(2)}_{jikl}). \tag{74c}$$

### D. Static $T$-matrix kernel

Once again the Fourier transform and projection does not need to be performed and similarly the matrix elements of $W^{(2T)}$ reads

$$W^{(2T)}_{pqrs}(\omega) = \langle pq|rs\rangle + \sum_{me} \left[ \frac{T_{pmre}T_{eqms}}{\omega - (\epsilon_e - \epsilon_m - 2\mathrm{i}\eta)} - \frac{T_{perm}T_{mqes}}{\omega - (\epsilon_m - \epsilon_e + 2\mathrm{i}\eta)} \right], \tag{75}$$

where the tensor elements of the effective interaction $T$ are given by

$$\begin{aligned} T_{pqrs}(\omega) &= \langle pq||rs\rangle + \sum_{\nu} \frac{M^{N+2}_{pq,\nu}(M^{N+2}_{rs,\nu})^*}{\omega - \Omega^{N+2}_\nu + \mathrm{i}\eta} - \sum_{\nu} \frac{M^{N-2}_{pq,\nu}(M^{N-2}_{rs,\nu})^*}{\omega - \Omega^{N-2}_\nu - \mathrm{i}\eta} \\ &= \langle pq||rs\rangle + T^{\mathrm{c}}_{pqrs}(\omega). \end{aligned} \tag{76}$$

The elements of the numerator are defined as

$$M^{N+2}_{pq,\nu} = \sum_{c<d} \langle pq||cd\rangle \, X^{N+2}_{cd,\nu} + \sum_{k<l} \langle pq||kl\rangle \, Y^{N+2}_{kl,\nu}, \tag{77a}$$

$$M^{N-2}_{pq,\nu} = \sum_{c<d} \langle pq||cd\rangle \, X^{N-2}_{cd,\nu} + \sum_{k<l} \langle pq||kl\rangle \, Y^{N-2}_{kl,\nu}. \tag{77b}$$

in terms of the eigenvectors of the pp-RPA problem

$$\begin{pmatrix} \boldsymbol{C}^{\mathrm{RPA}} & \boldsymbol{B}^{\mathrm{RPA}} \\ -\boldsymbol{B}^{\mathrm{RPA}} & -\boldsymbol{D}^{\mathrm{RPA}} \end{pmatrix} \cdot \begin{pmatrix} \boldsymbol{X}^{N+2} & \boldsymbol{Y}^{N-2} \\ \boldsymbol{Y}^{N+2} & \boldsymbol{X}^{N-2} \end{pmatrix} = \begin{pmatrix} \boldsymbol{X}^{N+2} & \boldsymbol{Y}^{N-2} \\ \boldsymbol{Y}^{N+2} & \boldsymbol{X}^{N-2} \end{pmatrix} \cdot \begin{pmatrix} \Omega^{N+2} & \boldsymbol{0} \\ \boldsymbol{0} & \Omega^{N-2} \end{pmatrix}. \tag{78}$$

Finally, within the static approximation, the elements of the various blocks are

$$C^{(2T)}_{ab,cd} = (\epsilon_a + \epsilon_b)\delta_{ac}\delta_{bd} + \langle ab||cd\rangle + (W^{\mathrm{c},(2T)}_{abcd} - W^{\mathrm{c},(2T)}_{bacd}), \tag{79a}$$

$$B^{(2T)}_{ab,ij} = \langle ab||ij\rangle + (W^{\mathrm{c},(2T)}_{abij} - W^{\mathrm{c},(2T)}_{baij}), \tag{79b}$$

$$D^{(2T)}_{ij,kl} = -(\epsilon_i + \epsilon_j)\delta_{ik}\delta_{jl} + \langle ij||kl\rangle + (W^{\mathrm{c},(2T)}_{ijkl} - W^{\mathrm{c},(2T)}_{jikl}). \tag{79c}$$

## VI. DYNAMIC KERNEL APPROXIMATIONS

This section aims to compute the effective dynamic kernels [see Eq. (19)] associated with the $GW$ and second-order kernels derived in the previous section. We recall that the static part of the kernel is left unchanged in $\tilde{\Xi}^{\text{pp}}$.

### A. Dynamic $GW$ kernel

#### 1. The hh-hh block

The expression of the hh-hh block matrix elements is obtained by combining Eqs. (42) and (65)

$$\tilde{\Xi}^{\text{pp},GW}_{ij,kl}(\omega) = \frac{\mathrm{i}}{2(2\pi)^2}\int \mathrm{d}(\tilde{\omega}\bar{\omega})\, e^{-\mathrm{i}\eta\tilde{\omega}}\left(\frac{1}{\tilde{\omega}-(\frac{\omega}{2}-\epsilon_j-\mathrm{i}\eta)}-\frac{1}{\tilde{\omega}-(\epsilon_i-\frac{\omega}{2}+\mathrm{i}\eta)}\right)$$
$$\times[W_{ijkl}(-\bar{\omega}-\tilde{\omega})+W_{ijkl}(-\bar{\omega}+\tilde{\omega})-W_{jikl}(-\bar{\omega}-\tilde{\omega})-W_{jikl}(-\bar{\omega}+\tilde{\omega})]e^{-\mathrm{i}\eta\bar{\omega}}\left(\frac{1}{\bar{\omega}-(\frac{\omega}{2}-\epsilon_l-\mathrm{i}\eta)}-\frac{1}{\bar{\omega}-(\epsilon_k-\frac{\omega}{2}+\mathrm{i}\eta)}\right). \tag{80}$$

We start by computing the dynamic part of the first term $W_{ijkl}(-\bar{\omega}-\tilde{\omega})$

$$\begin{aligned}
&\frac{\mathrm{i}}{2(2\pi)^2}\int \mathrm{d}(\tilde{\omega}\bar{\omega})\, e^{-\mathrm{i}\eta\tilde{\omega}}\left(\frac{1}{\tilde{\omega}-(\frac{\omega}{2}-\epsilon_j-\mathrm{i}\eta)}-\frac{1}{\tilde{\omega}-(\epsilon_i-\frac{\omega}{2}+\mathrm{i}\eta)}\right)\\
&\qquad\times\left(\sum_\mu\left[\frac{M_{ik,\mu}M^*_{lj,\mu}}{-\bar{\omega}-\tilde{\omega}-(\Omega_\mu-\mathrm{i}\eta)}-\frac{M^*_{ki,\mu}M_{jl,\mu}}{-\bar{\omega}-\tilde{\omega}-(-\Omega_\mu+\mathrm{i}\eta)}\right]\right)e^{-\mathrm{i}\eta\bar{\omega}}\left(\frac{1}{\bar{\omega}-(\frac{\omega}{2}-\epsilon_l-\mathrm{i}\eta)}-\frac{1}{\bar{\omega}-(\epsilon_k-\frac{\omega}{2}+\mathrm{i}\eta)}\right)\\
&=\frac{-\mathrm{i}}{2(2\pi)^2}\int \mathrm{d}(\tilde{\omega}\bar{\omega})\, e^{-\mathrm{i}\eta\tilde{\omega}}\left(\frac{1}{\tilde{\omega}-(\frac{\omega}{2}-\epsilon_j-\mathrm{i}\eta)}-\frac{1}{\tilde{\omega}-(\epsilon_i-\frac{\omega}{2}+\mathrm{i}\eta)}\right)\\
&\qquad\times\left(\sum_\mu\left[\frac{M_{ik,\mu}M^*_{lj,\mu}}{\bar{\omega}-(-\tilde{\omega}-\Omega_\mu+\mathrm{i}\eta)}-\frac{M^*_{ki,\mu}M_{jl,\mu}}{\bar{\omega}-(-\tilde{\omega}+\Omega_\mu-\mathrm{i}\eta)}\right]\right)e^{-\mathrm{i}\eta\bar{\omega}}\left(\frac{1}{\bar{\omega}-(\frac{\omega}{2}-\epsilon_l-\mathrm{i}\eta)}-\frac{1}{\bar{\omega}-(\epsilon_k-\frac{\omega}{2}+\mathrm{i}\eta)}\right)\\
&=\frac{-\mathrm{i}}{2(2\pi)^2}\int \mathrm{d}(\tilde{\omega}\bar{\omega})\, e^{-\mathrm{i}\eta\tilde{\omega}}\left(\frac{1}{\tilde{\omega}-(\frac{\omega}{2}-\epsilon_j-\mathrm{i}\eta)}-\frac{1}{\tilde{\omega}-(\epsilon_i-\frac{\omega}{2}+\mathrm{i}\eta)}\right)\\
&\qquad\times\left(\sum_\mu\frac{M_{ik,\mu}M^*_{lj,\mu}}{\bar{\omega}-(-\tilde{\omega}-\Omega_\mu+\mathrm{i}\eta)}\frac{1}{\bar{\omega}-(\frac{\omega}{2}-\epsilon_l-\mathrm{i}\eta)}+\frac{M^*_{ki,\mu}M_{jl,\mu}}{\bar{\omega}-(-\tilde{\omega}+\Omega_\mu-\mathrm{i}\eta)}\frac{1}{\bar{\omega}-(\epsilon_k-\frac{\omega}{2}+\mathrm{i}\eta)}\right)e^{-\mathrm{i}\eta\bar{\omega}}\\
&=\frac{-\mathrm{i}(-2\pi\mathrm{i})}{2(2\pi)^2}\int \mathrm{d}(\tilde{\omega})\, e^{-\mathrm{i}\eta\tilde{\omega}}\left(\frac{1}{\tilde{\omega}-(\frac{\omega}{2}-\epsilon_j-\mathrm{i}\eta)}-\frac{1}{\tilde{\omega}-(\epsilon_i-\frac{\omega}{2}+\mathrm{i}\eta)}\right)\\
&\qquad\times\left(\sum_\mu\frac{M_{ik,\mu}M^*_{lj,\mu}}{(\frac{\omega}{2}-\epsilon_l-\mathrm{i}\eta)-(-\tilde{\omega}-\Omega_\mu+\mathrm{i}\eta)}+\frac{M^*_{ki,\mu}M_{jl,\mu}}{(-\tilde{\omega}+\Omega_\mu-\mathrm{i}\eta)-(\epsilon_k-\frac{\omega}{2}+\mathrm{i}\eta)}\right)\\
&=\frac{-1}{4\pi}\int \mathrm{d}(\tilde{\omega})\, e^{-\mathrm{i}\eta\tilde{\omega}}\left(\frac{1}{\tilde{\omega}-(\frac{\omega}{2}-\epsilon_j-\mathrm{i}\eta)}-\frac{1}{\tilde{\omega}-(\epsilon_i-\frac{\omega}{2}+\mathrm{i}\eta)}\right)\\
&\qquad\times\left(\sum_\mu\frac{M_{ik,\mu}M^*_{lj,\mu}}{\tilde{\omega}-(-\frac{\omega}{2}+\epsilon_l-\Omega_\mu+2\mathrm{i}\eta)}-\frac{M^*_{ki,\mu}M_{jl,\mu}}{\tilde{\omega}-(\Omega_\mu-\epsilon_k+\frac{\omega}{2}-2\mathrm{i}\eta)}\right)\\
&=\frac{-1}{4\pi}\int \mathrm{d}(\tilde{\omega})\, e^{-\mathrm{i}\eta\tilde{\omega}}\sum_\mu\left(\frac{1}{\tilde{\omega}-(\frac{\omega}{2}-\epsilon_j-\mathrm{i}\eta)}\frac{M_{ik,\mu}M^*_{lj,\mu}}{\tilde{\omega}-(-\frac{\omega}{2}+\epsilon_l-\Omega_\mu+2\mathrm{i}\eta)}+\frac{1}{\tilde{\omega}-(\epsilon_i-\frac{\omega}{2}+\mathrm{i}\eta)}\frac{M^*_{ki,\mu}M_{jl,\mu}}{\tilde{\omega}-(\Omega_\mu-\epsilon_k+\frac{\omega}{2}-2\mathrm{i}\eta)}\right)\\
&=\frac{-(-2\pi\mathrm{i})}{4\pi}\sum_\mu\left(\frac{M_{ik,\mu}M^*_{lj,\mu}}{(\frac{\omega}{2}-\epsilon_j-\mathrm{i}\eta)-(-\frac{\omega}{2}+\epsilon_l-\Omega_\mu+2\mathrm{i}\eta)}+\frac{M^*_{ki,\mu}M_{jl,\mu}}{(\Omega_\mu-\epsilon_k+\frac{\omega}{2}-2\mathrm{i}\eta)-(\epsilon_i-\frac{\omega}{2}+\mathrm{i}\eta)}\right)\\
&=\frac{\mathrm{i}}{2}\sum_\mu\left(\frac{M_{ik,\mu}M^*_{lj,\mu}}{\omega-\epsilon_j-\epsilon_l+\Omega_\mu-3\mathrm{i}\eta}+\frac{M^*_{ki,\mu}M_{jl,\mu}}{\omega-\epsilon_k-\epsilon_i+\Omega_\mu-3\mathrm{i}\eta}\right).
\end{aligned}$$

The dynamic part of the second term $W_{ijkl}(-\bar{\omega}+\tilde{\omega})$ is computed similarly

$$
\begin{aligned}
&\frac{-\mathrm{i}(-2\pi\mathrm{i})}{2(2\pi)^2}\int \mathrm{d}(\tilde{\omega})\, e^{-\mathrm{i}\eta\tilde{\omega}}\left(\frac{1}{\tilde{\omega}-(\frac{\omega}{2}-\epsilon_j-\mathrm{i}\eta)}-\frac{1}{\tilde{\omega}-(\epsilon_i-\frac{\omega}{2}+\mathrm{i}\eta)}\right)\\
&\qquad\qquad\times\left(\sum_\mu \frac{M_{ik,\mu}M^*_{lj,\mu}}{(\frac{\omega}{2}-\epsilon_l-\mathrm{i}\eta)-(\tilde{\omega}-\Omega_\mu+\mathrm{i}\eta)}+\frac{M^*_{ki,\mu}M_{jl,\mu}}{(\tilde{\omega}+\Omega_\mu-\mathrm{i}\eta)-(\epsilon_k-\frac{\omega}{2}+\mathrm{i}\eta)}\right)\\
&=\frac{-1}{4\pi}\int \mathrm{d}(\tilde{\omega})\, e^{-\mathrm{i}\eta\tilde{\omega}}\left(\frac{1}{\tilde{\omega}-(\frac{\omega}{2}-\epsilon_j-\mathrm{i}\eta)}-\frac{1}{\tilde{\omega}-(\epsilon_i-\frac{\omega}{2}+\mathrm{i}\eta)}\right)\\
&\qquad\qquad\times\left(-\sum_\mu \frac{M_{ik,\mu}M^*_{lj,\mu}}{\tilde{\omega}-(\frac{\omega}{2}+\Omega_\mu-\epsilon_l-2\mathrm{i}\eta)}+\frac{M^*_{ki,\mu}M_{jl,\mu}}{\tilde{\omega}-(-\Omega_\mu+\epsilon_k-\frac{\omega}{2}+2\mathrm{i}\eta)}\right)\\
&=\frac{-1}{4\pi}\int \mathrm{d}(\tilde{\omega})\, e^{-\mathrm{i}\eta\tilde{\omega}}\sum_\mu\left(\frac{1}{\tilde{\omega}-(\frac{\omega}{2}-\epsilon_j-\mathrm{i}\eta)}\frac{M^*_{ki,\mu}M_{jl,\mu}}{\tilde{\omega}-(-\Omega_\mu+\epsilon_k-\frac{\omega}{2}+2\mathrm{i}\eta)}+\frac{1}{\tilde{\omega}-(\epsilon_i-\frac{\omega}{2}+\mathrm{i}\eta)}\frac{M_{ik,\mu}M^*_{lj,\mu}}{\tilde{\omega}-(\frac{\omega}{2}+\Omega_\mu-\epsilon_l-2\mathrm{i}\eta)}\right)\\
&=\frac{-(-2\pi\mathrm{i})}{4\pi}\sum_\mu\left(\frac{M^*_{ki,\mu}M_{jl,\mu}}{(\frac{\omega}{2}-\epsilon_j-\mathrm{i}\eta)-(-\Omega_\mu+\epsilon_k-\frac{\omega}{2}+2\mathrm{i}\eta)}+\frac{M_{ik,\mu}M^*_{lj,\mu}}{(\frac{\omega}{2}+\Omega_\mu-\epsilon_l-2\mathrm{i}\eta)-(\epsilon_i-\frac{\omega}{2}+\mathrm{i}\eta)}\right)\\
&=\frac{\mathrm{i}}{2}\sum_\mu\left(\frac{M^*_{ki,\mu}M_{jl,\mu}}{\omega-\epsilon_j-\epsilon_k+\Omega_\mu-3\mathrm{i}\eta}+\frac{M_{ik,\mu}M^*_{lj,\mu}}{\omega-\epsilon_l-\epsilon_i+\Omega_\mu-3\mathrm{i}\eta}\right).
\end{aligned}
$$

This finally gives the following matrix elements

$$
\begin{aligned}
\tilde{\Xi}^{\mathrm{pp},GW}_{ij,kl}(-\omega)=-\mathrm{i}\,\langle ij||kl\rangle-\frac{\mathrm{i}}{2}\sum_\mu&\left(\frac{M_{ik,\mu}M^*_{lj,\mu}-M_{jk,\mu}M^*_{li,\mu}}{\omega-(-\epsilon_j-\epsilon_l+\Omega_\mu-3\mathrm{i}\eta)}+\frac{M^*_{ki,\mu}M_{jl,\mu}-M^*_{kj,\mu}M_{il,\mu}}{\omega-(-\epsilon_i-\epsilon_k+\Omega_\mu-3\mathrm{i}\eta)}\right.\\
&\left.+\frac{M_{ik,\mu}M^*_{lj,\mu}-M_{jk,\mu}M^*_{li,\mu}}{\omega-(-\epsilon_i-\epsilon_l+\Omega_\mu-3\mathrm{i}\eta)}+\frac{M^*_{ki,\mu}M_{jl,\mu}-M^*_{kj,\mu}M_{il,\mu}}{\omega-(-\epsilon_j-\epsilon_k+\Omega_\mu-3\mathrm{i}\eta)}\right). \quad (81)
\end{aligned}
$$

### 2. *The hh-ee block*

The expression of the hh-ee block matrix elements reads

$$
\begin{aligned}
\tilde{\Xi}^{\mathrm{pp},GW}_{ab,ij}(\omega)&=\frac{-\mathrm{i}}{2(2\pi)^2}\int \mathrm{d}(\tilde{\omega}\bar{\omega})\, e^{-\mathrm{i}\eta\tilde{\omega}}\left(\frac{1}{\tilde{\omega}-(\frac{\omega}{2}-\epsilon_b+\mathrm{i}\eta)}-\frac{1}{\tilde{\omega}-(\epsilon_a-\frac{\omega}{2}-\mathrm{i}\eta)}\right)\\
\times[W_{abij}(-\bar{\omega}-\tilde{\omega})&+W_{abij}(-\bar{\omega}+\tilde{\omega})-W_{baij}(-\bar{\omega}-\tilde{\omega})-W_{baij}(-\bar{\omega}+\tilde{\omega})]e^{-\mathrm{i}\eta\bar{\omega}}\left(\frac{1}{\bar{\omega}-(\frac{\omega}{2}-\epsilon_j-\mathrm{i}\eta)}-\frac{1}{\bar{\omega}-(\epsilon_i-\frac{\omega}{2}+\mathrm{i}\eta)}\right). \quad (82)
\end{aligned}
$$

We start by computing the dynamic part of the first term $W_{abij}(-\bar{\omega}-\tilde{\omega})$

$$
\begin{aligned}
&\frac{1}{4\pi}\int \mathrm{d}(\tilde{\omega})\, e^{-\mathrm{i}\eta\tilde{\omega}}\left(\frac{1}{\tilde{\omega}-(\frac{\omega}{2}-\epsilon_b+\mathrm{i}\eta)}-\frac{1}{\tilde{\omega}-(\epsilon_a-\frac{\omega}{2}-\mathrm{i}\eta)}\right)\\
&\qquad\qquad\times\left(\sum_\mu \frac{M_{ai,\mu}M^*_{jb,\mu}}{\tilde{\omega}-(-\frac{\omega}{2}+\epsilon_j-\Omega_\mu+2\mathrm{i}\eta)}-\frac{M^*_{ia,\mu}M_{bj,\mu}}{\tilde{\omega}-(\Omega_\mu-\epsilon_i+\frac{\omega}{2}-2\mathrm{i}\eta)}\right)\\
&=\frac{1}{4\pi}\int \mathrm{d}(\tilde{\omega})\, e^{-\mathrm{i}\eta\tilde{\omega}}\sum_\mu\left(-\frac{1}{\tilde{\omega}-(\epsilon_a-\frac{\omega}{2}-\mathrm{i}\eta)}\frac{M_{ai,\mu}M^*_{jb,\mu}}{\tilde{\omega}-(-\frac{\omega}{2}+\epsilon_j-\Omega_\mu+2\mathrm{i}\eta)}-\frac{1}{\tilde{\omega}-(\frac{\omega}{2}-\epsilon_b+\mathrm{i}\eta)}\frac{M^*_{ia,\mu}M_{bj,\mu}}{\tilde{\omega}-(\Omega_\mu-\epsilon_i+\frac{\omega}{2}-2\mathrm{i}\eta)}\right)\\
&=\frac{-(-2\pi\mathrm{i})}{4\pi}\sum_\mu\left(\frac{M_{ai,\mu}M^*_{jb,\mu}}{(\epsilon_a-\frac{\omega}{2}-\mathrm{i}\eta)-(-\frac{\omega}{2}+\epsilon_j-\Omega_\mu+2\mathrm{i}\eta)}+\frac{M^*_{ia,\mu}M_{bj,\mu}}{(\Omega_\mu-\epsilon_i+\frac{\omega}{2}-2\mathrm{i}\eta)-(\frac{\omega}{2}-\epsilon_b+\mathrm{i}\eta)}\right)\\
&=\frac{\mathrm{i}}{2}\sum_\mu\left(\frac{M_{ai,\mu}M^*_{jb,\mu}}{\epsilon_a-\epsilon_j+\Omega_\mu-3\mathrm{i}\eta}+\frac{M^*_{ia,\mu}M_{bj,\mu}}{\epsilon_b-\epsilon_i+\Omega_\mu-3\mathrm{i}\eta}\right).
\end{aligned}
$$

The dynamic part of the second term $W_{abij}(-\bar{\omega}+\tilde{\omega})$ is computed similarly

$$= \frac{1}{4\pi}\int \mathrm{d}(\tilde{\omega})\, e^{-\mathrm{i}\eta\tilde{\omega}} \left( \frac{1}{\tilde{\omega}-(\frac{\omega}{2}-\epsilon_b+\mathrm{i}\eta)} - \frac{1}{\tilde{\omega}-(\epsilon_a-\frac{\omega}{2}-\mathrm{i}\eta)} \right) \times \left( -\sum_\mu \frac{M_{ai,\mu}M^*_{jb,\mu}}{\tilde{\omega}-(\frac{\omega}{2}+\Omega_\mu-\epsilon_j-2\mathrm{i}\eta)} + \frac{M^*_{ia,\mu}M_{bj,\mu}}{\tilde{\omega}-(-\Omega_\mu+\epsilon_i-\frac{\omega}{2}+2\mathrm{i}\eta)} \right)$$

$$= \frac{-1}{4\pi}\int \mathrm{d}(\tilde{\omega})\, e^{-\mathrm{i}\eta\tilde{\omega}} \sum_\mu \left( \frac{1}{\tilde{\omega}-(\epsilon_a-\frac{\omega}{2}-\mathrm{i}\eta)} \frac{M^*_{ia,\mu}M_{bj,\mu}}{\tilde{\omega}-(-\Omega_\mu+\epsilon_i-\frac{\omega}{2}+2\mathrm{i}\eta)} + \frac{1}{\tilde{\omega}-(\frac{\omega}{2}-\epsilon_b+\mathrm{i}\eta)} \frac{M_{ai,\mu}M^*_{jb,\mu}}{\tilde{\omega}-(\frac{\omega}{2}+\Omega_\mu-\epsilon_j-2\mathrm{i}\eta)} \right)$$

$$= \frac{-(-2\pi\mathrm{i})}{4\pi} \sum_\mu \left( \frac{M^*_{ia,\mu}M_{bj,\mu}}{(\epsilon_a-\frac{\omega}{2}-\mathrm{i}\eta)-(-\Omega_\mu+\epsilon_i-\frac{\omega}{2}+2\mathrm{i}\eta)} + \frac{M_{ai,\mu}M^*_{jb,\mu}}{(\frac{\omega}{2}+\Omega_\mu-\epsilon_j-2\mathrm{i}\eta)-(\frac{\omega}{2}-\epsilon_b+\mathrm{i}\eta)} \right)$$

$$= \frac{\mathrm{i}}{2}\sum_\mu \left( \frac{M^*_{ia,\mu}M_{bj,\mu}}{\epsilon_a-\epsilon_i+\Omega_\mu-3\mathrm{i}\eta} + \frac{M_{ai,\mu}M^*_{jb,\mu}}{\epsilon_b-\epsilon_j+\Omega_\mu-3\mathrm{i}\eta} \right).$$

The two remaining exchange terms are easily computed and this finally gives the following matrix elements

$$\tilde{\Xi}^{\mathrm{pp},GW}_{ab,ij}(\omega) = -\mathrm{i}\,\langle ab||ij\rangle - \frac{\mathrm{i}}{2}\sum_\mu \left( \frac{M_{ai,\mu}M^*_{jb,\mu}-M_{bi,\mu}M^*_{ja,\mu}}{-(\epsilon_a-\epsilon_j+\Omega_\mu-3\mathrm{i}\eta)} + \frac{M^*_{ia,\mu}M_{bj,\mu}-M^*_{ib,\mu}M_{aj,\mu}}{-(\epsilon_b-\epsilon_i+\Omega_\mu-3\mathrm{i}\eta)} + \frac{M_{ai,\mu}M^*_{jb,\mu}-M_{bi,\mu}M^*_{ja,\mu}}{-(\epsilon_b-\epsilon_j+\Omega_\mu-3\mathrm{i}\eta)} + \frac{M^*_{ia,\mu}M_{bj,\mu}-M^*_{ib,\mu}M_{aj,\mu}}{-(\epsilon_a-\epsilon_i+\Omega_\mu-3\mathrm{i}\eta)} \right). \quad (83)$$

### *3. The ee-ee block*

The expression of the ee-ee block matrix elements reads

$$\tilde{\Xi}^{\mathrm{pp},GW}_{ab,cd}(\omega) = \frac{\mathrm{i}}{2(2\pi)^2}\int \mathrm{d}(\tilde{\omega}\bar{\omega})\, e^{-\mathrm{i}\eta\tilde{\omega}} \left( \frac{1}{\tilde{\omega}-(\frac{\omega}{2}-\epsilon_b+\mathrm{i}\eta)} - \frac{1}{\tilde{\omega}-(\epsilon_a-\frac{\omega}{2}-\mathrm{i}\eta)} \right) \times [W_{abcd}(-\bar{\omega}-\tilde{\omega})+W_{abcd}(-\bar{\omega}+\tilde{\omega})-W_{bacd}(-\bar{\omega}-\tilde{\omega})-W_{bacd}(-\bar{\omega}+\tilde{\omega})] e^{-\mathrm{i}\eta\bar{\omega}} \left( \frac{1}{\bar{\omega}-(\frac{\omega}{2}-\epsilon_d+\mathrm{i}\eta)} - \frac{1}{\bar{\omega}-(\epsilon_c-\frac{\omega}{2}-\mathrm{i}\eta)} \right). \quad (84)$$

We start by computing the dynamic part of the first term $W_{abcd}(-\bar{\omega}-\tilde{\omega})$

$$\frac{-\mathrm{i}}{2(2\pi)^2}\int \mathrm{d}(\tilde{\omega}\bar{\omega})\, e^{-\mathrm{i}\eta\tilde{\omega}} \left( \frac{1}{\tilde{\omega}-(\frac{\omega}{2}-\epsilon_b+\mathrm{i}\eta)} - \frac{1}{\tilde{\omega}-(\epsilon_a-\frac{\omega}{2}-\mathrm{i}\eta)} \right) \left( \sum_\mu \left[ \frac{M_{ac,\mu}M^*_{db,\mu}}{\bar{\omega}-(-\tilde{\omega}-\Omega_\mu+\mathrm{i}\eta)} - \frac{M^*_{ca,\mu}M_{bd,\mu}}{\bar{\omega}-(-\tilde{\omega}+\Omega_\mu-\mathrm{i}\eta)} \right] \right) \times e^{-\mathrm{i}\eta\bar{\omega}} \left( \frac{1}{\bar{\omega}-(\frac{\omega}{2}-\epsilon_d+\mathrm{i}\eta)} - \frac{1}{\bar{\omega}-(\epsilon_c-\frac{\omega}{2}-\mathrm{i}\eta)} \right)$$

$$= \frac{-\mathrm{i}}{2(2\pi)^2}\int \mathrm{d}(\tilde{\omega}\bar{\omega})\, e^{-\mathrm{i}\eta\tilde{\omega}} \left( \frac{1}{\tilde{\omega}-(\frac{\omega}{2}-\epsilon_b+\mathrm{i}\eta)} - \frac{1}{\tilde{\omega}-(\epsilon_a-\frac{\omega}{2}-\mathrm{i}\eta)} \right) \times \left( -\sum_\mu \frac{M_{ac,\mu}M^*_{db,\mu}}{\bar{\omega}-(-\tilde{\omega}-\Omega_\mu+\mathrm{i}\eta)} \frac{1}{\bar{\omega}-(\epsilon_c-\frac{\omega}{2}-\mathrm{i}\eta)} - \sum_\mu \frac{M^*_{ca,\mu}M_{bd,\mu}}{\bar{\omega}-(-\tilde{\omega}+\Omega_\mu-\mathrm{i}\eta)} \frac{1}{\bar{\omega}-(\frac{\omega}{2}-\epsilon_d+\mathrm{i}\eta)} \right) e^{-\mathrm{i}\eta\bar{\omega}}$$

$$= \frac{\mathrm{i}(-2\pi\mathrm{i})}{2(2\pi)^2}\int \mathrm{d}\tilde{\omega}\, e^{-\mathrm{i}\eta\tilde{\omega}} \left( \frac{1}{\tilde{\omega}-(\frac{\omega}{2}-\epsilon_b+\mathrm{i}\eta)} - \frac{1}{\tilde{\omega}-(\epsilon_a-\frac{\omega}{2}-\mathrm{i}\eta)} \right) \times \left( \sum_\mu \frac{M_{ac,\mu}M^*_{db,\mu}}{(\epsilon_c-\frac{\omega}{2}-\mathrm{i}\eta)-(-\tilde{\omega}-\Omega_\mu+\mathrm{i}\eta)} + \sum_\mu \frac{M^*_{ca,\mu}M_{bd,\mu}}{(-\tilde{\omega}+\Omega_\mu-\mathrm{i}\eta)-(\frac{\omega}{2}-\epsilon_d+\mathrm{i}\eta)} \right)$$

$$= \frac{1}{4\pi}\int \mathrm{d}\tilde{\omega}\, e^{-\mathrm{i}\eta\tilde{\omega}} \left( \frac{1}{\tilde{\omega}-(\frac{\omega}{2}-\epsilon_b+\mathrm{i}\eta)} - \frac{1}{\tilde{\omega}-(\epsilon_a-\frac{\omega}{2}-\mathrm{i}\eta)} \right) \times \left( \sum_\mu \frac{M_{ac,\mu}M^*_{db,\mu}}{\tilde{\omega}-(\frac{\omega}{2}-\epsilon_c-\Omega_\mu+2\mathrm{i}\eta)} - \sum_\mu \frac{M^*_{ca,\mu}M_{bd,\mu}}{\tilde{\omega}-(-\frac{\omega}{2}+\epsilon_d+\Omega_\mu-2\mathrm{i}\eta)} \right)$$

$$= \frac{-1}{4\pi} \int \mathrm{d}\tilde{\omega}\, e^{-\mathrm{i}\eta\tilde{\omega}} \left( \sum_\mu \frac{1}{\tilde{\omega} - (\frac{\omega}{2} - \epsilon_b + \mathrm{i}\eta)} \frac{M^*_{ca,\mu} M_{bd,\mu}}{\tilde{\omega} - (-\frac{\omega}{2} + \epsilon_d + \Omega_\mu - 2\mathrm{i}\eta)} \right.$$

$$\left. + \sum_\mu \frac{M_{ac,\mu} M^*_{db,\mu}}{\tilde{\omega} - (\frac{\omega}{2} - \epsilon_c - \Omega_\mu + 2\mathrm{i}\eta)} \frac{1}{\tilde{\omega} - (\epsilon_a - \frac{\omega}{2} - \mathrm{i}\eta)} \right)$$

$$= \frac{-(-2\pi\mathrm{i})}{4\pi} \left( \sum_\mu \frac{M^*_{ca,\mu} M_{bd,\mu}}{(-\frac{\omega}{2} + \epsilon_d + \Omega_\mu - 2\mathrm{i}\eta) - (\frac{\omega}{2} - \epsilon_b + \mathrm{i}\eta)} + \sum_\mu \frac{M_{ac,\mu} M^*_{db,\mu}}{(\epsilon_a - \frac{\omega}{2} - \mathrm{i}\eta) - (\frac{\omega}{2} - \epsilon_c - \Omega_\mu + 2\mathrm{i}\eta)} \right)$$

$$= -\frac{\mathrm{i}}{2} \sum_\mu \left( \frac{M^*_{ca,\mu} M_{bd,\mu}}{\omega - (\epsilon_d + \epsilon_b + \Omega_\mu - 3\mathrm{i}\eta)} + \frac{M_{ac,\mu} M^*_{db,\mu}}{\omega - (\epsilon_a + \epsilon_c + \Omega_\mu - 3\mathrm{i}\eta)} \right).$$

The dynamic part of the second term $W_{abcd}(-\bar{\omega} + \tilde{\omega})$ is computed similarly

$$\frac{1}{4\pi} \int \mathrm{d}\tilde{\omega}\, e^{-\mathrm{i}\eta\tilde{\omega}} \left( \frac{1}{\tilde{\omega} - (\frac{\omega}{2} - \epsilon_b + \mathrm{i}\eta)} - \frac{1}{\tilde{\omega} - (\epsilon_a - \frac{\omega}{2} - \mathrm{i}\eta)} \right)$$

$$\times \left( -\sum_\mu \frac{M_{ac,\mu} M^*_{db,\mu}}{\tilde{\omega} - (\epsilon_c - \frac{\omega}{2} + \Omega_\mu - 2\mathrm{i}\eta)} + \sum_\mu \frac{M^*_{ca,\mu} M_{bd,\mu}}{\tilde{\omega} - (\frac{\omega}{2} - \Omega_\mu - \epsilon_d + 2\mathrm{i}\eta)} \right)$$

$$= \frac{-1}{4\pi} \int \mathrm{d}\tilde{\omega}\, e^{-\mathrm{i}\eta\tilde{\omega}} \left( \sum_\mu \frac{1}{\tilde{\omega} - (\frac{\omega}{2} - \epsilon_b + \mathrm{i}\eta)} \frac{M_{ac,\mu} M^*_{db,\mu}}{\tilde{\omega} - (\epsilon_c - \frac{\omega}{2} + \Omega_\mu - 2\mathrm{i}\eta)} \right.$$

$$\left. + \sum_\mu \frac{M^*_{ca,\mu} M_{bd,\mu}}{\tilde{\omega} - (\frac{\omega}{2} - \Omega_\mu - \epsilon_d + 2\mathrm{i}\eta)} \frac{1}{\tilde{\omega} - (\epsilon_a - \frac{\omega}{2} - \mathrm{i}\eta)} \right)$$

$$= \frac{-(-2\pi\mathrm{i})}{4\pi} \left( \sum_\mu \frac{M_{ac,\mu} M^*_{db,\mu}}{(\epsilon_c - \frac{\omega}{2} + \Omega_\mu - 2\mathrm{i}\eta) - (\frac{\omega}{2} - \epsilon_b + \mathrm{i}\eta)} + \sum_\mu \frac{M^*_{ca,\mu} M_{bd,\mu}}{(\epsilon_a - \frac{\omega}{2} - \mathrm{i}\eta) - (\frac{\omega}{2} - \Omega_\mu - \epsilon_d + 2\mathrm{i}\eta)} \right)$$

$$= -\frac{\mathrm{i}}{2} \sum_\mu \left( \frac{M_{ac,\mu} M^*_{db,\mu}}{\omega - (\epsilon_b + \epsilon_c + \Omega_\mu - 3\mathrm{i}\eta)} + \frac{M^*_{ca,\mu} M_{bd,\mu}}{\omega - (\epsilon_a + \epsilon_d + \Omega_\mu - 3\mathrm{i}\eta)} \right).$$

which, finally, gives the following matrix elements

$$\tilde{\Xi}^{\mathrm{pp},GW}_{ab,cd}(\omega) = -\mathrm{i} \langle ab||cd\rangle - \frac{\mathrm{i}}{2} \sum_\mu \left( \frac{M_{ac,\mu} M^*_{db,\mu} - M_{bc,\mu} M^*_{da,\mu}}{\omega - (\epsilon_a + \epsilon_c + \Omega_\mu - 3\mathrm{i}\eta)} + \frac{M^*_{ca,\mu} M_{bd,\mu} - M^*_{cb,\mu} M_{ad,\mu}}{\omega - (\epsilon_b + \epsilon_d + \Omega_\mu - 3\mathrm{i}\eta)} \right.$$
$$\left. + \frac{M_{ac,\mu} M^*_{db,\mu} - M_{bc,\mu} M^*_{da,\mu}}{\omega - (\epsilon_b + \epsilon_c + \Omega_\mu - 3\mathrm{i}\eta)} + \frac{M^*_{ca,\mu} M_{bd,\mu} - M^*_{cb,\mu} M_{ad,\mu}}{\omega - (\epsilon_a + \epsilon_d + \Omega_\mu - 3\mathrm{i}\eta)} \right). \quad (85)$$

### B. Dynamic second-order Coulomb kernel

The derivation of the matrix elements of the dynamic second-order kernel is almost the same but with $W^{(2)}_{pqrs}(\omega)$ instead of $W_{pqrs}(\omega)$. The corresponding expressions are reported below.

#### 1. *The hh-hh block*

$$\tilde{\Xi}^{\mathrm{pp},(2)}_{ij,kl}(-\omega) = -\mathrm{i} \langle ij||kl\rangle - \frac{\mathrm{i}}{2} \sum_{me} \left( \frac{\langle im||ke\rangle \langle ej||ml\rangle - \langle jm||ke\rangle \langle ei||ml\rangle}{\omega - (-\epsilon_j - \epsilon_l + \epsilon_e - \epsilon_m - 3\mathrm{i}\eta)} + \frac{\langle ie||km\rangle \langle mj||el\rangle - \langle je||km\rangle \langle mi||el\rangle}{\omega - (-\epsilon_i - \epsilon_k + \epsilon_e - \epsilon_m - 3\mathrm{i}\eta)} \right.$$
$$\left. + \frac{\langle im||ke\rangle \langle ej||ml\rangle - \langle jm||ke\rangle \langle ei||ml\rangle}{\omega - (-\epsilon_i - \epsilon_l + \epsilon_e - \epsilon_m - 3\mathrm{i}\eta)} + \frac{\langle ie||km\rangle \langle mj||el\rangle - \langle je||km\rangle \langle mi||el\rangle}{\omega - (-\epsilon_j - \epsilon_k + \epsilon_e - \epsilon_m - 3\mathrm{i}\eta)} \right). \quad (86)$$

### 2. The hh-ee block

$$\tilde{\Xi}^{\text{pp},(2)}_{ab,ij}(\omega) = -\mathrm{i}\langle ab||ij\rangle - \frac{\mathrm{i}}{2}\sum_{me}\left(\frac{\langle am||ie\rangle\,\langle eb||mj\rangle - \langle bm||ie\rangle\,\langle ea||mj\rangle}{-(\epsilon_a - \epsilon_j + \epsilon_e - \epsilon_m - 3\mathrm{i}\eta)} + \frac{\langle ae||im\rangle\,\langle mb||ej\rangle - \langle be||im\rangle\,\langle ma||ej\rangle}{-(\epsilon_b - \epsilon_i + \epsilon_e - \epsilon_m - 3\mathrm{i}\eta)} + \frac{\langle am||ie\rangle\,\langle eb||mj\rangle - \langle bm||ie\rangle\,\langle ea||mj\rangle}{-(\epsilon_b - \epsilon_j + \epsilon_e - \epsilon_m - 3\mathrm{i}\eta)} + \frac{\langle ae||im\rangle\,\langle mb||ej\rangle - \langle be||im\rangle\,\langle ma||ej\rangle}{-(\epsilon_a - \epsilon_i + \epsilon_e - \epsilon_m - 3\mathrm{i}\eta)}\right). \tag{87}$$

### 3. The ee-ee block

$$\tilde{\Xi}^{\text{pp},(2)}_{ab,cd}(\omega) = -\mathrm{i}\langle ab||cd\rangle - \frac{\mathrm{i}}{2}\sum_{me}\left(\frac{\langle am||ce\rangle\,\langle eb||md\rangle - \langle bm||ce\rangle\,\langle ea||md\rangle}{\omega - (\epsilon_a + \epsilon_c + \epsilon_e - \epsilon_m - 3\mathrm{i}\eta)} + \frac{\langle ae||cm\rangle\,\langle mb||ed\rangle - \langle be||cm\rangle\,\langle ma||ed\rangle}{\omega - (\epsilon_b + \epsilon_d + \epsilon_e - \epsilon_m - 3\mathrm{i}\eta)} + \frac{\langle am||ce\rangle\,\langle eb||md\rangle - \langle bm||ce\rangle\,\langle ea||md\rangle}{\omega - (\epsilon_b + \epsilon_c + \epsilon_e - \epsilon_m - 3\mathrm{i}\eta)} + \frac{\langle ae||cm\rangle\,\langle mb||ed\rangle - \langle be||cm\rangle\,\langle ma||ed\rangle}{\omega - (\epsilon_a + \epsilon_d + \epsilon_e - \epsilon_m - 3\mathrm{i}\eta)}\right). \tag{88}$$

## VII. SPIN-ADAPTATION

### A. Spin-adaptation of the eigenvalue problem

In Sec. III, the antisymmetry of $\boldsymbol{K}$, $\boldsymbol{K}_0$, and $\tilde{\boldsymbol{\Xi}}$ has been used to reduce the dimension of the matrix to diagonalize from $4K^2$ to $K(2K-1)$ (where $K$ is the number of spatial orbitals). This can be further reduced by spin-adapting the antisymmetrized basis set defined in Eq. (30). This is the purpose of the present subsection but, first, additional notations must be introduced. For the sake of conciseness, the notation $\overline{\varphi_p(\mathbf{x}_1)\varphi_q(\mathbf{x}_2)} = (\varphi_p(\mathbf{x}_1)\varphi_q(\mathbf{x}_2) - \varphi_q(\mathbf{x}_1)\varphi_p(\mathbf{x}_2))/\sqrt{2}$ will be used. In addition, we write a spinorbital index $p$ with the more general notation $p_\sigma$ (with $\sigma = \uparrow$ or $\downarrow$) as the spin must now be specified. Hence, in the remainder of this subsection, Roman letters $p, q, r, \ldots$ correspond to spatial orbitals instead of spinorbitals.

The $K(2K-1)$ antisymmetric basis functions of Eq. (30) can be further divided in three sets of size $K$, $K(K-1)$, and $K(K-1)$ as

$$\left\{\overline{\varphi_{p_\uparrow}(\mathbf{x}_1)\varphi_{p_\downarrow}(\mathbf{x}_2)}\right\}_{p\in[1,K]} \bigcup \left\{\overline{\varphi_{p_\sigma}(\mathbf{x}_1)\varphi_{q_{\sigma'}}(\mathbf{x}_2)}\right\}_{p<q,q\in[1,K],\sigma\in\{\uparrow,\downarrow\},\sigma'\neq\sigma} \bigcup \left\{\overline{\varphi_{p_\sigma}(\mathbf{x}_1)\varphi_{q_\sigma}(\mathbf{x}_2)}\right\}_{p<q,q\in[1,K],\sigma\in\{\uparrow,\downarrow\}}. \tag{89}$$

In the first set, the two spinorbitals have the same spatial part but a different spin. This corresponds to a set of singlet states ($S=0$). In the third set, the situation is reversed. This forms two sets of triplet states ($S=1$) corresponding to $M_S = \pm 1$ with $K(K-1)/2$ terms each. The basis functions composing the remaining set are not spin eigenfunctions but this set can be combined as

$$\left\{\frac{\overline{\varphi_{p_\uparrow}(\mathbf{x}_1)\varphi_{q_\downarrow}(\mathbf{x}_2)} + \overline{\varphi_{p_\downarrow}(\mathbf{x}_1)\varphi_{q_\uparrow}(\mathbf{x}_2)}}{\sqrt{2}}\right\}_{p<q,q\in[1,K]} \bigcup \left\{\frac{\overline{\varphi_{p_\uparrow}(\mathbf{x}_1)\varphi_{q_\downarrow}(\mathbf{x}_2)} - \overline{\varphi_{p_\downarrow}(\mathbf{x}_1)\varphi_{q_\uparrow}(\mathbf{x}_2)}}{\sqrt{2}}\right\}_{p<q,q\in[1,K]} \tag{90}$$

to produce a set of $K(K-1)/2$ triplet states with $M_S = 0$ and $K(K-1)/2$ singlet states, respectively. Finally, the two sets of singlet states can be combined as a unique set of $K(K+1)/2$ singlet states, as follows

$$\left\{\frac{\overline{\varphi_{p_\uparrow}(\mathbf{x}_1)\varphi_{q_\downarrow}(\mathbf{x}_2)} - \overline{\varphi_{p_\downarrow}(\mathbf{x}_1)\varphi_{q_\uparrow}(\mathbf{x}_2)}}{\sqrt{2}\sqrt{1+\delta_{pq}}}\right\}_{p\leqslant q,q\in[1,K]}. \tag{91}$$

Because the Hamiltonian is spin-independent, the coupling between triplet blocks, and between singlet and triplet blocks, is zero. Hence, instead of diagonalizing a matrix of size $K(2K-1)$, one can diagonalize two independent matrices of size $K(K+1)/2$ and $K(K-1)/2$ to get the singlet and triplet states, respectively. The matrix elements of one of the three equivalent triplet eigenvalue problems read

$${}^3C_{ab,cd} = C_{a_\uparrow b_\uparrow, c_\uparrow d_\uparrow}, \tag{92a}$$

$$ {}^3B_{ab,ij} = B_{a_\uparrow b_\uparrow, i_\uparrow j_\uparrow}, \tag{92b} $$

$$ {}^3D_{ij,kl} = D_{i_\uparrow j_\uparrow, k_\uparrow l_\uparrow}, \tag{92c} $$

with the following restrictions on the spatial orbital indices $i < j$, $k < l$, $a < b$ and $c < d$. The singlet matrix elements are slightly more involved

$$ {}^1C_{ab,cd} = \frac{C_{a_\uparrow b_\downarrow, c_\uparrow d_\downarrow} - C_{a_\downarrow b_\uparrow, c_\uparrow d_\downarrow}}{\sqrt{1+\delta_{ab}}\sqrt{1+\delta_{cd}}}, \tag{93a} $$

$$ {}^1B_{ab,ij} = \frac{B_{a_\uparrow b_\downarrow, i_\uparrow j_\downarrow} - B_{a_\downarrow b_\uparrow, i_\uparrow j_\downarrow}}{\sqrt{1+\delta_{ab}}\sqrt{1+\delta_{ij}}}, \tag{93b} $$

$$ {}^1D_{ij,kl} = \frac{D_{i_\uparrow j_\downarrow, k_\uparrow l_\downarrow} - D_{i_\downarrow j_\uparrow, k_\uparrow l_\downarrow}}{\sqrt{1+\delta_{ij}}\sqrt{1+\delta_{kl}}}, \tag{93c} $$

with the following restrictions on the spatial orbital indices $i \leq j$, $k \leq l$, $a \leq b$ and $c \leq d$.

### B. Static first-order kernel

The triplet block in spatial orbitals is equal to the following spinorbital block

$$ {}^3C_{ab,cd} = (\epsilon_{a_\uparrow} + \epsilon_{b_\uparrow})\delta_{a_\uparrow c_\uparrow}\delta_{b_\uparrow d_\uparrow} + \langle a_\uparrow b_\uparrow || c_\uparrow d_\uparrow \rangle = (\epsilon_a + \epsilon_b)\delta_{ac}\delta_{bd} + \langle ab||cd \rangle \,, \tag{94} $$

and this leads to the following triplet pp-RPA eigenvalue problem

$$ {}^3C_{ab,cd} = (\epsilon_a + \epsilon_b)\delta_{ac}\delta_{bd} + \langle ab||cd \rangle \,, \tag{95a} $$

$$ {}^3B_{ab,ij} = \langle ab||ij \rangle \,, \tag{95b} $$

$$ {}^3D_{ij,kl} = -(\epsilon_i + \epsilon_j)\delta_{ik}\delta_{jl} + \langle ij||kl \rangle \,, \tag{95c} $$

which is identical to the one of Sec. IV. Remember though that the indices now correspond to spatial orbitals. The singlet block is worked out as

$$ \begin{aligned} {}^1C_{ab,cd} &= \frac{(\epsilon_{a_\uparrow} + \epsilon_{b_\downarrow})\delta_{a_\uparrow c_\uparrow}\delta_{b_\downarrow d_\downarrow} - (\epsilon_{a_\downarrow} + \epsilon_{b_\uparrow})\delta_{a_\downarrow c_\uparrow}\delta_{b_\uparrow d_\downarrow} + \langle a_\uparrow b_\downarrow || c_\uparrow d_\downarrow \rangle - \langle a_\downarrow b_\uparrow || c_\uparrow d_\downarrow \rangle}{\sqrt{1+\delta_{ab}}\sqrt{1+\delta_{cd}}} \\ &= \frac{(\epsilon_a + \epsilon_b)\delta_{ac}\delta_{bd} + \langle ab|cd \rangle + \langle ab|dc \rangle}{\sqrt{1+\delta_{ab}}\sqrt{1+\delta_{cd}}}. \end{aligned} \tag{96} $$

Hence, the singlet eigenvalue problem is

$$ {}^1C_{ab,cd} = \frac{(\epsilon_a + \epsilon_b)\delta_{ac}\delta_{bd} + \langle ab|cd \rangle + \langle ab|dc \rangle}{\sqrt{1+\delta_{ab}}\sqrt{1+\delta_{cd}}}, \tag{97a} $$

$$ {}^1B_{ab,ij} = \frac{\langle ab|ij \rangle + \langle ab|ji \rangle}{\sqrt{1+\delta_{ab}}\sqrt{1+\delta_{ij}}}, \tag{97b} $$

$$ {}^1D_{ij,kl} = \frac{-(\epsilon_i + \epsilon_j)\delta_{ik}\delta_{jl} + \langle ij|kl \rangle + \langle ij|lk \rangle}{\sqrt{1+\delta_{ij}}\sqrt{1+\delta_{kl}}}. \tag{97c} $$

### C. Static $GW$ kernel

Before spin-adapting the static $GW$ kernel, we recall that the screened interaction is spin-independent [10], *i.e.*,

$$ \begin{aligned} W_{p_\uparrow q_\uparrow r_\uparrow s_\uparrow} &= W_{p_\downarrow q_\downarrow r_\downarrow s_\downarrow} = W_{p_\uparrow q_\downarrow r_\uparrow s_\downarrow} = W_{p_\downarrow q_\uparrow r_\downarrow s_\uparrow}, \\ W_{p_\uparrow q_\downarrow r_\downarrow s_\uparrow} &= W_{p_\downarrow q_\uparrow r_\uparrow s_\downarrow} = 0, \end{aligned} \tag{98} $$

and the non-zero elements will be denoted as $W_{pqrs}$. These tensor elements in spatial orbitals are

$$ W_{pqrs}(\omega) = \langle pq|rs \rangle + W^{\text{c}}_{pqrs}(\omega), \tag{99} $$

where

$$W^{\mathrm{c}}_{pqrs}(\omega) = 2 \sum_{\mu} \left[ \frac{M_{pr,\mu} M^*_{sq,\mu}}{\omega - \Omega_\mu + \mathrm{i}\eta} - \frac{M^*_{rp,\mu} M_{qs,\mu}}{\omega + \Omega_\mu - \mathrm{i}\eta} \right]. \tag{100}$$

The screened integrals are defined as

$$M_{pq,\mu} = \sum_{ia} [X_{ia,\mu} \langle ap|iq \rangle + Y_{ia,\mu} \langle ip|aq \rangle], \tag{101}$$

with $X_{ia,\mu}$ and $Y_{ia,\mu}$ the eigenvectors of the singlet eh-RPA eigenvalue problem. Therefore, the derivation of the singlet and triplet blocks closely follows the previous subsection and yields

$$^3C_{ab,cd} = (\epsilon_a + \epsilon_b)\delta_{ac}\delta_{bd} + \langle ab||cd \rangle + (W^{\mathrm{c}}_{abcd} - W^{\mathrm{c}}_{bacd}), \tag{102a}$$

$$^3B_{ab,ij} = \langle ab||ij \rangle + (W^{\mathrm{c}}_{abij} - W^{\mathrm{c}}_{baij}), \tag{102b}$$

$$^3D_{ij,kl} = -(\epsilon_i + \epsilon_j)\delta_{ik}\delta_{jl} + \langle ij||kl \rangle + (W^{\mathrm{c}}_{ijkl} - W^{\mathrm{c}}_{jikl}), \tag{102c}$$

and

$$^1C_{ab,cd} = \frac{(\epsilon_a + \epsilon_b)\delta_{ac}\delta_{bd} + \langle ab|cd \rangle + \langle ab|dc \rangle + W^{\mathrm{c}}_{abcd} + W^{\mathrm{c}}_{bacd}}{\sqrt{1+\delta_{ab}}\sqrt{1+\delta_{cd}}}, \tag{103a}$$

$$^1B_{ab,ij} = \frac{\langle ab|ij \rangle + \langle ab|ji \rangle + W^{\mathrm{c}}_{abij} + W^{\mathrm{c}}_{baij}}{\sqrt{1+\delta_{ab}}\sqrt{1+\delta_{ij}}}, \tag{103b}$$

$$^1D_{ij,kl} = \frac{-(\epsilon_i + \epsilon_j)\delta_{ik}\delta_{jl} + \langle ij|kl \rangle + \langle ij|lk \rangle + W^{\mathrm{c}}_{ijkl} + W^{\mathrm{c}}_{jikl}}{\sqrt{1+\delta_{ij}}\sqrt{1+\delta_{kl}}}. \tag{103c}$$

### D. Static second-order kernel

In this case, the interaction is not spin-independent and we start by focusing on the spin-adaptation of the effective interaction before turning to the spin-adapted pp-BSE blocks. The $\uparrow\uparrow\uparrow\uparrow$ contribution reads

$$\begin{aligned} W^{\mathrm{c},(2)}_{p_\uparrow q_\uparrow r_\uparrow s_\uparrow}(\omega) &= \sum_{me}\sum_{\sigma\sigma'} \left[ \frac{\langle p_\uparrow m_\sigma || r_\uparrow e_{\sigma'} \rangle \langle e_{\sigma'} q_\uparrow || m_\sigma s_\uparrow \rangle}{\omega - (\epsilon_{e_{\sigma'}} - \epsilon_{m_\sigma} - 2\mathrm{i}\eta)} - \frac{\langle p_\uparrow e_{\sigma'} || r_\uparrow m_\sigma \rangle \langle m_\sigma q_\uparrow || e_{\sigma'} s_\uparrow \rangle}{\omega - (\epsilon_{m_\sigma} - \epsilon_{e_{\sigma'}} + 2\mathrm{i}\eta)} \right] \\ &= \sum_{me} \left[ \frac{2\langle pm|re \rangle \langle eq|ms \rangle - \langle pm|re \rangle \langle eq|sm \rangle - \langle pm|er \rangle \langle eq|ms \rangle + \langle pm|er \rangle \langle eq|sm \rangle}{\omega - (\epsilon_e - \epsilon_m - 2\mathrm{i}\eta)} \right. \\ &\qquad \left. - \frac{2\langle pe|rm \rangle \langle mq|es \rangle - \langle pe|rm \rangle \langle mq|se \rangle - \langle pe|mr \rangle \langle mq|es \rangle + \langle pe|mr \rangle \langle mq|se \rangle}{\omega - (\epsilon_m - \epsilon_e + 2\mathrm{i}\eta)} \right]. \end{aligned} \tag{104}$$

The $\uparrow\downarrow\uparrow\downarrow$ component is

$$\begin{aligned} W^{\mathrm{c},(2)}_{p_\uparrow q_\downarrow r_\uparrow s_\downarrow}(\omega) &= \sum_{me}\sum_{\sigma\sigma'} \left[ \frac{\langle p_\uparrow m_\sigma || r_\uparrow e_{\sigma'} \rangle \langle e_{\sigma'} q_\downarrow || m_\sigma s_\downarrow \rangle}{\omega - (\epsilon_{e_{\sigma'}} - \epsilon_{m_\sigma} - 2\mathrm{i}\eta)} - \frac{\langle p_\uparrow e_{\sigma'} || r_\uparrow m_\sigma \rangle \langle m_\sigma q_\downarrow || e_{\sigma'} s_\downarrow \rangle}{\omega - (\epsilon_{m_\sigma} - \epsilon_{e_{\sigma'}} + 2\mathrm{i}\eta)} \right] \\ &= \sum_{me} \left[ \frac{2\langle pm|re \rangle \langle eq|ms \rangle - \langle pm|re \rangle \langle eq|sm \rangle - \langle pm|er \rangle \langle eq|ms \rangle}{\omega - (\epsilon_e - \epsilon_m - 2\mathrm{i}\eta)} \right. \\ &\qquad \left. - \frac{2\langle pe|rm \rangle \langle mq|es \rangle - \langle pe|rm \rangle \langle mq|se \rangle - \langle pe|mr \rangle \langle mq|es \rangle}{\omega - (\epsilon_m - \epsilon_e + 2\mathrm{i}\eta)} \right]. \end{aligned} \tag{105}$$

Finally, the $\downarrow\uparrow\uparrow\downarrow$ contribution reads

$$\begin{aligned} W^{\mathrm{c},(2)}_{p_\downarrow q_\uparrow r_\uparrow s_\downarrow}(\omega) &= \sum_{me}\sum_{\sigma\sigma'} \left[ \frac{\langle p_\downarrow m_\sigma || r_\uparrow e_{\sigma'} \rangle \langle e_{\sigma'} q_\uparrow || m_\sigma s_\downarrow \rangle}{\omega - (\epsilon_{e_{\sigma'}} - \epsilon_{m_\sigma} - 2\mathrm{i}\eta)} - \frac{\langle p_\downarrow e_{\sigma'} || r_\uparrow m_\sigma \rangle \langle m_\sigma q_\uparrow || e_{\sigma'} s_\downarrow \rangle}{\omega - (\epsilon_{m_\sigma} - \epsilon_{e_{\sigma'}} + 2\mathrm{i}\eta)} \right] \\ &= \sum_{me} \left[ \frac{\langle pm|er \rangle \langle eq|sm \rangle}{\omega - (\epsilon_e - \epsilon_m - 2\mathrm{i}\eta)} - \frac{\langle pe|mr \rangle \langle mq|se \rangle}{\omega - (\epsilon_m - \epsilon_e + 2\mathrm{i}\eta)} \right]. \end{aligned} \tag{106}$$

The triplet and singlet eigenvalue problems can be deduced

$$
\begin{aligned}
{}^3C_{ab,cd} &= (\epsilon_a + \epsilon_b)\delta_{ac}\delta_{bd} + \langle ab||cd\rangle + ({}^3W^{\text{c},(2)}_{abcd} - {}^3W^{\text{c},(2)}_{bacd}), && \text{(107a)}\\
{}^3B_{ab,ij} &= \langle ab||ij\rangle + ({}^3W^{\text{c},(2)}_{abij} - {}^3W^{\text{c},(2)}_{baij}), && \text{(107b)}\\
{}^3D_{ij,kl} &= -(\epsilon_i + \epsilon_j)\delta_{ik}\delta_{jl} + \langle ij||kl\rangle + ({}^3W^{\text{c},(2)}_{ijkl} - {}^3W^{\text{c},(2)}_{jikl}), && \text{(107c)}
\end{aligned}
$$

where

$$
\begin{aligned}
{}^3W^{\text{c},(2)}_{pqrs}(\omega) = \sum_{me} \Bigg[ &\frac{2\langle pm|re\rangle\langle eq|ms\rangle - \langle pm|re\rangle\langle eq|sm\rangle - \langle pm|er\rangle\langle eq|ms\rangle + \langle pm|er\rangle\langle eq|sm\rangle}{\omega - (\epsilon_e - \epsilon_m - 2\mathrm{i}\eta)} \\
&- \frac{2\langle pe|rm\rangle\langle mq|es\rangle - \langle pe|rm\rangle\langle mq|se\rangle - \langle pe|mr\rangle\langle mq|es\rangle + \langle pe|mr\rangle\langle mq|se\rangle}{\omega - (\epsilon_m - \epsilon_e + 2\mathrm{i}\eta)} \Bigg], \qquad (108)
\end{aligned}
$$

and

$$
\begin{aligned}
{}^1C_{ab,cd} &= \frac{(\epsilon_a + \epsilon_b)\delta_{ac}\delta_{bd} + \langle ab|cd\rangle + \langle ab|dc\rangle + {}^1W^{\text{c},(2)}_{abcd} + {}^1W^{\text{c},(2)}_{bacd}}{\sqrt{1+\delta_{ab}}\sqrt{1+\delta_{cd}}}, && \text{(109a)}\\
{}^1B_{ab,ij} &= \frac{\langle ab|ij\rangle + \langle ab|ji\rangle + {}^1W^{\text{c},(2)}_{abij} + {}^1W^{\text{c},(2)}_{baij}}{\sqrt{1+\delta_{ab}}\sqrt{1+\delta_{ij}}}, && \text{(109b)}\\
{}^1D_{ij,kl} &= \frac{-(\epsilon_i + \epsilon_j)\delta_{ik}\delta_{jl} + \langle ij|kl\rangle + \langle ij|lk\rangle + {}^1W^{\text{c},(2)}_{ijkl} + {}^1W^{\text{c},(2)}_{jikl}}{\sqrt{1+\delta_{ij}}\sqrt{1+\delta_{kl}}}, && \text{(109c)}
\end{aligned}
$$

where

$$
\begin{aligned}
{}^1W^{\text{c},(2)}_{pqrs}(\omega) = \sum_{me} \Bigg[ &\frac{2\langle pm|re\rangle\langle eq|ms\rangle - \langle pm|re\rangle\langle eq|sm\rangle - \langle pm|er\rangle\langle eq|ms\rangle - \langle pm|er\rangle\langle eq|sm\rangle}{\omega - (\epsilon_e - \epsilon_m - 2\mathrm{i}\eta)} \\
&- \frac{2\langle pe|rm\rangle\langle mq|es\rangle - \langle pe|rm\rangle\langle mq|se\rangle - \langle pe|mr\rangle\langle mq|es\rangle - \langle pe|mr\rangle\langle mq|se\rangle}{\omega - (\epsilon_m - \epsilon_e + 2\mathrm{i}\eta)} \Bigg]. \qquad (110)
\end{aligned}
$$

### E. Static $T$-matrix kernel

Once again, the effective interaction is spin-dependent. Before spin-adapting the static $T$-matrix kernel, we recall the tensor elements of $T$ for the various spin cases. The $\uparrow\uparrow\uparrow\uparrow$ contribution reads

$$
\begin{aligned}
T_{p_\uparrow q_\uparrow r_\uparrow s_\uparrow}(\omega) &= \langle p_\uparrow q_\uparrow||r_\uparrow s_\uparrow\rangle + \sum_\nu \frac{M^{N+2}_{p_\uparrow q_\uparrow,\nu}(M^{N+2}_{r_\uparrow s_\uparrow,\nu})^*}{\omega - \Omega^{N+2}_\nu + \mathrm{i}\eta} - \sum_\nu \frac{M^{N-2}_{p_\uparrow q_\uparrow,\nu}(M^{N-2}_{r_\uparrow s_\uparrow,\nu})^*}{\omega - \Omega^{N-2}_\nu - \mathrm{i}\eta} \\
&= \langle pq||rs\rangle + \sum_\nu \frac{{}^3M^{N+2}_{pq,\nu}({}^3M^{N+2}_{rs,\nu})^*}{\omega - {}^3\Omega^{N+2}_\nu + \mathrm{i}\eta} - \sum_\nu \frac{{}^3M^{N-2}_{pq,\nu}({}^3M^{N-2}_{rs,\nu})^*}{\omega - {}^3\Omega^{N-2}_\nu - \mathrm{i}\eta},
\end{aligned} \qquad (111)
$$

where the triplet transition densities are given by

$$
\begin{aligned}
{}^3M^{N+2}_{pq,\nu} &= \sum_{c<d} \langle pq||cd\rangle\, {}^3X^{N+2}_{cd,\nu} + \sum_{k<l} \langle pq||kl\rangle\, {}^3Y^{N+2}_{kl,\nu}, && \text{(112a)}\\
{}^3M^{N-2}_{pq,\nu} &= \sum_{c<d} \langle pq||cd\rangle\, {}^3X^{N-2}_{cd,\nu} + \sum_{k<l} \langle pq||kl\rangle\, {}^3Y^{N-2}_{kl,\nu}. && \text{(112b)}
\end{aligned}
$$

The $\uparrow\downarrow\uparrow\downarrow$ component is

$$
\begin{aligned}
T_{p_\uparrow q_\downarrow r_\uparrow s_\downarrow}(\omega) &= \langle pq|rs\rangle + \sum_\nu \frac{M^{N+2}_{p_\uparrow q_\downarrow,\nu}(M^{N+2}_{r_\uparrow s_\downarrow,\nu})^*}{\omega - \Omega^{N+2}_\nu + \mathrm{i}\eta} - \sum_\nu \frac{M^{N-2}_{p_\uparrow q_\downarrow,\nu}(M^{N-2}_{r_\uparrow s_\downarrow,\nu})^*}{\omega - \Omega^{N-2}_\nu - \mathrm{i}\eta} \\
&= \langle pq|rs\rangle + \frac{1}{2}\left(\sum_\nu \frac{{}^1M^{N+2}_{pq,\nu}({}^1M^{N+2}_{rs,\nu})^*}{\omega - {}^1\Omega^{N+2}_\nu + \mathrm{i}\eta} - \sum_\nu \frac{{}^1M^{N-2}_{pq,\nu}({}^1M^{N-2}_{rs,\nu})^*}{\omega - {}^1\Omega^{N-2}_\nu - \mathrm{i}\eta}\right) + \frac{1}{2}\left(\sum_\nu \frac{{}^3M^{N+2}_{pq,\nu}({}^3M^{N+2}_{rs,\nu})^*}{\omega - {}^3\Omega^{N+2}_\nu + \mathrm{i}\eta} - \sum_\nu \frac{{}^3M^{N-2}_{pq,\nu}({}^3M^{N-2}_{rs,\nu})^*}{\omega - {}^1\Omega^{N-2}_\nu - \mathrm{i}\eta}\right)
\end{aligned} \qquad (113)
$$

where the singlet transition densities are given by

$$ {}^{1}M_{pq,\nu}^{N+2} = \sum_{c\leqslant d} \frac{\langle pq|cd\rangle + \langle pq|dc\rangle}{\sqrt{1+\delta_{cd}}} {}^{1}X_{cd,\nu}^{N+2} + \sum_{k\leqslant l} \frac{\langle pq|kl\rangle + \langle pq|lk\rangle}{\sqrt{1+\delta_{kl}}} {}^{1}Y_{kl,\nu}^{N+2}, \tag{114a} $$

$$ {}^{1}M_{pq,\nu}^{N-2} = \sum_{c\leqslant d} \frac{\langle pq|cd\rangle + \langle pq|dc\rangle}{\sqrt{1+\delta_{cd}}} {}^{1}X_{cd,\nu}^{N-2} + \sum_{k\leqslant l} \frac{\langle pq|kl\rangle + \langle pq|lk\rangle}{\sqrt{1+\delta_{kl}}} {}^{1}Y_{kl,\nu}^{N-2}. \tag{114b} $$

Finally, the $\downarrow\uparrow\uparrow\downarrow$ contribution reads

$$ \begin{aligned} T_{p_\downarrow q_\uparrow r_\uparrow s_\downarrow}(\omega) &= -\langle pq|sr\rangle + \sum_\nu \frac{M_{p_\downarrow q_\uparrow,\nu}^{N+2}(M_{r_\uparrow s_\downarrow,\nu}^{N+2})^*}{\omega - \Omega_\nu^{N+2} + \mathrm{i}\eta} - \sum_\nu \frac{M_{p_\downarrow q_\uparrow,\nu}^{N-2}(M_{r_\uparrow s_\downarrow,\nu}^{N-2})^*}{\omega - \Omega_\nu^{N-2} - \mathrm{i}\eta} \\ &= -\langle pq|sr\rangle - \frac{1}{2}\left( \sum_\nu \frac{{}^{1}M_{pq,\nu}^{N+2}({}^{1}M_{rs,\nu}^{N+2})^*}{\omega - {}^{1}\Omega_\nu^{N+2} + \mathrm{i}\eta} - \sum_\nu \frac{{}^{1}M_{pq,\nu}^{N-2}({}^{1}M_{rs,\nu}^{N-2})^*}{\omega - {}^{1}\Omega_\nu^{N-2} - \mathrm{i}\eta} \right) + \frac{1}{2}\left( \sum_\nu \frac{{}^{3}M_{pq,\nu}^{N+2}({}^{3}M_{rs,\nu}^{N+2})^*}{\omega - {}^{3}\Omega_\nu^{N+2} + \mathrm{i}\eta} - \sum_\nu \frac{{}^{3}M_{pq,\nu}^{N-2}({}^{3}M_{rs,\nu}^{N-2})^*}{\omega - {}^{1}\Omega_\nu^{N-2} - \mathrm{i}\eta} \right) \end{aligned} \tag{115} $$

The spin components of $T$ can be used to compute the spin components of $W^{(2T)}$, as follows

$$ \begin{aligned} W_{p_\uparrow q_\uparrow r_\uparrow s_\uparrow}^{\mathrm{c},(2T)}(\omega) &= \sum_{me}\sum_{\sigma\sigma'} \left[ \frac{T_{p_\uparrow m_\sigma r_\uparrow e_{\sigma'}} T_{e_{\sigma'} q_\uparrow m_\sigma s_\uparrow}}{\omega - (\epsilon_{e_{\sigma'}} - \epsilon_{m_\sigma} - 2\mathrm{i}\eta)} - \frac{T_{p_\uparrow e_{\sigma'} r_\uparrow m_\sigma} T_{m_\sigma q_\uparrow e_{\sigma'} s_\uparrow}}{\omega - (\epsilon_{m_\sigma} - \epsilon_{e_{\sigma'}} + 2\mathrm{i}\eta)} \right] \\ &= \sum_{me} \left[ \frac{T_{p_\uparrow m_\uparrow r_\uparrow e_\uparrow} T_{e_\uparrow q_\uparrow m_\uparrow s_\uparrow}}{\omega - (\epsilon_e - \epsilon_m - 2\mathrm{i}\eta)} - \frac{T_{p_\uparrow e_\uparrow r_\uparrow m_\uparrow} T_{m_\uparrow q_\uparrow e_\uparrow s_\uparrow}}{\omega - (\epsilon_m - \epsilon_e + 2\mathrm{i}\eta)} \right] + \sum_{me} \left[ \frac{T_{p_\uparrow m_\downarrow r_\uparrow e_\downarrow} T_{e_\downarrow q_\uparrow m_\downarrow s_\uparrow}}{\omega - (\epsilon_e - \epsilon_m - 2\mathrm{i}\eta)} - \frac{T_{p_\uparrow e_\downarrow r_\uparrow m_\downarrow} T_{m_\downarrow q_\uparrow e_\downarrow s_\uparrow}}{\omega - (\epsilon_m - \epsilon_e + 2\mathrm{i}\eta)} \right] \end{aligned} \tag{116} $$

$$ \begin{aligned} W_{p_\uparrow q_\downarrow r_\uparrow s_\downarrow}^{\mathrm{c},(2T)}(\omega) &= \sum_{me}\sum_{\sigma\sigma'} \left[ \frac{T_{p_\uparrow m_\sigma r_\uparrow e_{\sigma'}} T_{e_{\sigma'} q_\downarrow m_\sigma s_\downarrow}}{\omega - (\epsilon_{e_{\sigma'}} - \epsilon_{m_\sigma} - 2\mathrm{i}\eta)} - \frac{T_{p_\uparrow e_{\sigma'} r_\uparrow m_\sigma} T_{m_\sigma q_\downarrow e_{\sigma'} s_\downarrow}}{\omega - (\epsilon_{m_\sigma} - \epsilon_{e_{\sigma'}} + 2\mathrm{i}\eta)} \right] \\ &= \sum_{me} \left[ \frac{T_{p_\uparrow m_\uparrow r_\uparrow e_\uparrow} T_{e_\uparrow q_\downarrow m_\uparrow s_\downarrow}}{\omega - (\epsilon_e - \epsilon_m - 2\mathrm{i}\eta)} - \frac{T_{p_\uparrow e_\uparrow r_\uparrow m_\uparrow} T_{m_\uparrow q_\downarrow e_\uparrow s_\downarrow}}{\omega - (\epsilon_m - \epsilon_e + 2\mathrm{i}\eta)} \right] + \sum_{me} \left[ \frac{T_{p_\uparrow m_\downarrow r_\uparrow e_\downarrow} T_{e_\downarrow q_\downarrow m_\downarrow s_\downarrow}}{\omega - (\epsilon_e - \epsilon_m - 2\mathrm{i}\eta)} - \frac{T_{p_\uparrow e_\downarrow r_\uparrow m_\downarrow} T_{m_\downarrow q_\downarrow e_\downarrow s_\downarrow}}{\omega - (\epsilon_m - \epsilon_e + 2\mathrm{i}\eta)} \right] \end{aligned} \tag{117} $$

$$ \begin{aligned} W_{p_\downarrow q_\uparrow r_\uparrow s_\downarrow}^{\mathrm{c},(2T)}(\omega) &= \sum_{me}\sum_{\sigma\sigma'} \left[ \frac{T_{p_\downarrow m_\sigma r_\uparrow e_{\sigma'}} T_{e_{\sigma'} q_\uparrow m_\sigma s_\downarrow}}{\omega - (\epsilon_{e_{\sigma'}} - \epsilon_{m_\sigma} - 2\mathrm{i}\eta)} - \frac{T_{p_\downarrow e_{\sigma'} r_\uparrow m_\sigma} T_{m_\sigma q_\uparrow e_{\sigma'} s_\downarrow}}{\omega - (\epsilon_{m_\sigma} - \epsilon_{e_{\sigma'}} + 2\mathrm{i}\eta)} \right] \\ &= \sum_{me} \left[ \frac{T_{p_\downarrow m_\uparrow r_\uparrow e_\downarrow} T_{e_\downarrow q_\uparrow m_\uparrow s_\downarrow}}{\omega - (\epsilon_e - \epsilon_m - 2\mathrm{i}\eta)} - \frac{T_{p_\downarrow e_\uparrow r_\uparrow m_\downarrow} T_{m_\downarrow q_\uparrow e_\uparrow s_\downarrow}}{\omega - (\epsilon_m - \epsilon_e + 2\mathrm{i}\eta)} \right] \end{aligned} \tag{118} $$

The triplet eigenvalue problem reads

$$ {}^{3}C_{ab,cd} = (\epsilon_a + \epsilon_b)\delta_{ac}\delta_{bd} + \langle ab||cd\rangle + (W_{a_\uparrow b_\uparrow c_\uparrow d_\uparrow}^{\mathrm{c},(2T)} - W_{b_\uparrow a_\uparrow c_\uparrow d_\uparrow}^{\mathrm{c},(2T)}), \tag{119a} $$

$$ {}^{3}B_{ab,ij} = \langle ab||ij\rangle + (W_{a_\uparrow b_\uparrow i_\uparrow j_\uparrow}^{\mathrm{c},(2T)} - W_{b_\uparrow a_\uparrow i_\uparrow j_\uparrow}^{\mathrm{c},(2T)}), \tag{119b} $$

$$ {}^{3}D_{ij,kl} = -(\epsilon_i + \epsilon_j)\delta_{ik}\delta_{jl} + \langle ij||kl\rangle + (W_{i_\uparrow j_\uparrow k_\uparrow l_\uparrow}^{\mathrm{c},(2T)} - W_{j_\uparrow i_\uparrow k_\uparrow l_\uparrow}^{\mathrm{c},(2T)}). \tag{119c} $$

The singlet block is worked out as

$$ \begin{aligned} {}^{1}C_{ab,cd} &= \frac{C_{a_\uparrow b_\downarrow, c_\uparrow d_\downarrow} - C_{a_\downarrow b_\uparrow, c_\uparrow d_\downarrow}}{\sqrt{1+\delta_{ab}}\sqrt{1+\delta_{cd}}} \\ &= \frac{(\epsilon_a + \epsilon_b)\delta_{ac}\delta_{bd} + \Xi_{a_\uparrow b_\downarrow, c_\uparrow d_\downarrow} - \Xi_{a_\downarrow b_\uparrow, c_\uparrow d_\downarrow}}{\sqrt{1+\delta_{ab}}\sqrt{1+\delta_{cd}}} \\ &= \frac{(\epsilon_a + \epsilon_b)\delta_{ac}\delta_{bd} + \langle ab|cd\rangle + \langle ab|dc\rangle + W_{a_\uparrow b_\downarrow, c_\uparrow d_\downarrow}^{\mathrm{c},(2T)} - W_{b_\downarrow a_\uparrow, c_\uparrow d_\downarrow}^{\mathrm{c},(2T)} - W_{a_\downarrow b_\uparrow, c_\uparrow d_\downarrow}^{\mathrm{c},(2T)} + W_{b_\uparrow a_\downarrow, c_\uparrow d_\downarrow}^{\mathrm{c},(2T)}}{\sqrt{1+\delta_{ab}}\sqrt{1+\delta_{cd}}}. \end{aligned} \tag{120} $$

Hence, the singlet eigenvalue problem is

$$ {}^{1}C_{ab,cd} = \frac{(\epsilon_a + \epsilon_b)\delta_{ac}\delta_{bd} + \langle ab|cd\rangle + \langle ab|dc\rangle}{\sqrt{1+\delta_{ab}}\sqrt{1+\delta_{cd}}}, \tag{121a} $$

$$ {}^{1}B_{ab,ij} = \frac{\langle ab|ij\rangle + \langle ab|ji\rangle}{\sqrt{1+\delta_{ab}}\sqrt{1+\delta_{ij}}}, \tag{121b} $$

$$ {}^{1}D_{ij,kl} = \frac{-(\epsilon_i+\epsilon_j)\delta_{ik}\delta_{jl} + \langle ij|kl\rangle + \langle ij|lk\rangle}{\sqrt{1+\delta_{ij}}\sqrt{1+\delta_{kl}}}. \tag{121c} $$

### F. Dynamic $GW$ kernel

For the sake of conciseness, only the kernel matrix elements will be reported in this section. Note that the first-order part of the kernel will also be removed as it has already been spin-adapted in Sec. VII B. The triplet kernel reads

$$ {}^{3}\tilde{\Xi}^{\text{pp}}_{ij,kl}(-\omega) = \tilde{\Xi}^{\text{pp}}_{i_\uparrow j_\uparrow,k_\uparrow l_\uparrow}(-\omega) = -\mathrm{i}\sum_\nu \left[ \frac{M_{ik,\nu}M^*_{lj,\nu} - M_{jk,\nu}M^*_{li,\nu}}{\omega-(-\epsilon_j-\epsilon_l+\Omega_\nu-3\mathrm{i}\eta)} + \frac{M^*_{ki,\nu}M_{jl,\nu} - M^*_{kj,\nu}M_{il,\nu}}{\omega-(-\epsilon_i-\epsilon_k+\Omega_\nu-3\mathrm{i}\eta)} \right. $$
$$ \left. + \frac{M_{ik,\nu}M^*_{lj,\nu} - M_{jk,\nu}M^*_{li,\nu}}{\omega-(-\epsilon_i-\epsilon_l+\Omega_\nu-3\mathrm{i}\eta)} + \frac{M^*_{ki,\nu}M_{jl,\nu} - M^*_{kj,\nu}M_{il,\nu}}{\omega-(-\epsilon_j-\epsilon_k+\Omega_\nu-3\mathrm{i}\eta)} \right]. \tag{122} $$

The two remaining blocks are very similar, *i.e.*, they just have an additional factor 2 with respect to their spinorbital counterpart. The singlet matrix elements are

$$ {}^{1}\tilde{\Xi}^{\text{pp}}_{ij,kl}(-\omega) = \tilde{\Xi}^{\text{pp}}_{i_\uparrow j_\uparrow,k_\uparrow l_\uparrow}(-\omega) = \frac{-\mathrm{i}}{\sqrt{1+\delta_{ij}}\sqrt{1+\delta_{kl}}}\sum_\nu \left[ \frac{M_{ik,\nu}M^*_{lj,\nu} + M_{jk,\nu}M^*_{li,\nu}}{\omega-(-\epsilon_j-\epsilon_l+\Omega_\nu-3\mathrm{i}\eta)} + \frac{M^*_{ki,\nu}M_{jl,\nu} + M^*_{kj,\nu}M_{il,\nu}}{\omega-(-\epsilon_i-\epsilon_k+\Omega_\nu-3\mathrm{i}\eta)} \right. $$
$$ \left. + \frac{M_{ik,\nu}M^*_{lj,\nu} + M_{jk,\nu}M^*_{li,\nu}}{\omega-(-\epsilon_i-\epsilon_l+\Omega_\nu-3\mathrm{i}\eta)} + \frac{M^*_{ki,\nu}M_{jl,\nu} + M^*_{kj,\nu}M_{il,\nu}}{\omega-(-\epsilon_j-\epsilon_k+\Omega_\nu-3\mathrm{i}\eta)} \right]. \tag{123} $$

## VIII. RESULTS

Before presenting the additional results in this section, which supplement the discussion in the main manuscript, Table I provides an overview of the methods used in this study along with their associated computational costs.

TABLE I. Main equation and computational cost associated with the various methods considered in the present study.

| Method | Equation | Cost |
|---|---|---|
| ppRPA | (61) | $\mathcal{O}(V^6)$ |
| TDA@ppRPA | (61a) | $\mathcal{O}(O^6)$ |
| DIP-CCSD | | $\mathcal{O}(O^4V^2)$ |
| ppBSE@$GW$ | (66) | $\mathcal{O}(V^6)$ |
| TDA@ppBSE@$GW$ | (66c) | $\mathcal{O}(O^5V)$ |
| TDA@dynBSE@$GW$ | (81) | $\mathcal{O}(O^5V)$ |
| ppBSE@$GT$ | (79) | $\mathcal{O}(V^6)$ |
| ppBSE@GF(2) | (74) | $\mathcal{O}(V^6)$ |

This section gathers some additional results to complement the discussion contained in the main manuscript. Table IV shows the pp-RPA double ionization potentials (DIPs) obtained with ev$GW$ and qs$GW$ quasiparticle energies and the corresponding histogram of errors are displayed in Fig. 5. The ev$GW$ and qs$GW$ were implemented following the scheme of Ref. 11 and using a flow parameter $s = 500$, except for the HCl molecule where $s = 100$ was used to improve ev$GW$ convergence. The MAE of ppRPA@ev$GW$ and ppRPA@qs$GW$ are 1.74 eV and 1.76 eV, respectively. Therefore, self-consistency provides a slight improvement over the one-shot scheme (ppRPA@$GW$ in the main manuscript) and its MAE of 1.96 eV.

TABLE II. DIPs (in eV) toward the singlet (left panel) and triplet (right panel) dication ground states in the aug-cc-pVTZ basis set computed at the pp-RPA level using ev$GW$ and qs$GW$ quasiparticle energies.

| | Singlet DIPs | | Triplet DIPs | |
|---|---|---|---|---|
| Molecule | ppRPA@ev$GW$ | ppRPA@qs$GW$ | ppRPA@ev$GW$ | ppRPA@qs$GW$ |
| $H_2O$ | 44.76 | 44.77 | 44.17 | 44.27 |
| HF | 54.59 | 54.98 | 52.37 | 52.79 |
| Ne | 68.97 | 69.52 | 66.28 | 66.86 |
| $CH_4$ | 40.88 | 40.70 | 40.18 | 39.99 |
| $NH_3$ | 38.33 | 38.22 | 41.16 | 41.06 |
| CO | 42.58 | 41.82 | 41.84 | 41.67 |
| $N_2$ | 44.00 | 43.20 | 46.04 | 45.47 |
| BF | 35.28 | 34.91 | 37.92 | 38.12 |
| LiF | 43.22 | 43.81 | 41.19 | 41.82 |
| BeO | 34.69 | 35.78 | 33.32 | 34.44 |
| BN | 36.74 | 37.34 | 35.59 | 36.17 |
| $C_2$ | 37.92 | 37.92 | 37.57 | 36.85 |
| CS | 34.72 | 34.22 | 34.07 | 33.48 |
| LiCl | 32.36 | 32.37 | 30.98 | 31.00 |
| $F_2$ | 44.59 | 44.78 | 44.35 | 44.54 |
| $H_2S$ | 32.79 | 32.71 | 34.10 | 34.00 |
| $PH_3$ | 32.26 | 32.14 | 33.32 | 33.16 |
| HCl | 38.68 | 38.65 | 37.21 | 37.18 |
| Ar | 46.26 | 46.22 | 44.54 | 44.50 |
| $SiH_4$ | 33.71 | 33.54 | 33.49 | 33.31 |
| $CH_2O$ | 34.04 | 34.34 | 37.50 | 38.07 |
| $CO_2$ | 38.76 | 38.80 | 38.34 | 38.36 |
| $BH_3$ | 37.63 | 37.48 | 36.34 | 36.18 |
| MSE | 1.71 | 1.70 | 1.91 | 1.97 |
| MAE | 1.71 | 1.70 | 1.96 | 2.00 |
| RMSE | 2.00 | 2.12 | 2.30 | 2.47 |
| SDE | 1.06 | 1.30 | 1.30 | 1.52 |
| Min | 0.11 | 0.26 | -0.55 | -0.35 |
| Max | 3.91 | 4.29 | 4.47 | 4.89 |

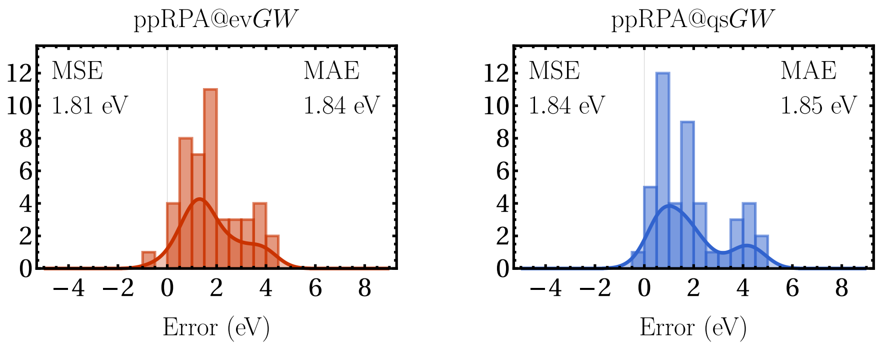


FIG. 5. Histogram of the errors (with respect to FCI) for the singlet and triplet principal DIPs of 23 small molecules in the aug-cc-pVTZ basis set at the pp-RPA level using ev$GW$ and qs$GW$ quasiparticle energies.

Secondly, the effect of the Tamm-Dancoff approximation (TDA) is investigated by computing the DIPs within this approximation for three different kernels: ppRPA@HF, static GF(2) kernel [ppBSE@GF(2)] and static $T$-matrix kernel [ppBSE@$GT$]. The corresponding results and histogram of errors are shown in Fig. 6 and Table III, respectively. These results complement the TDA@ppBSE@$GW$ results of the main text. In the four cases, the TDA leads to an increase of the MSE, *i.e.*, to an increase of the DIPs on average. Hence, if the full pp-BSE scheme has a negative MSE [as for ppBSE@$GW$ and ppBSE@GF(2)], the TDA leads to a decrease in MAE. On the other hand, if the full ppBSE scheme has a positive MSE [as for ppRPA@HF and ppBSE@$GT$], the TDA worsens the MAE.

TABLE III. DIPs (in eV) toward the singlet (left panel) and triplet (right panel) dication ground states in the aug-cc-pVTZ basis set computed at the pp-BSE level using various static kernels: RPA@HF, GF(2) and $T$-matrix.

| | Singlet DIPs | | | Triplet DIPs | | |
|---|---|---|---|---|---|---|
| Molecule | TDA ppRPA@HF | TDA ppBSE@GF(2) | TDA ppBSE@$GT$ | TDA ppRPA@HF | TDA ppBSE@GF(2) | TDA ppRPA@$GT$ |
| $H_2O$ | 47.36 | 38.20 | 42.30 | 46.36 | 36.43 | 41.27 |
| HF | 58.15 | 45.94 | 51.60 | 55.82 | 42.61 | 49.06 |
| Ne | 73.11 | 60.99 | 66.37 | 70.32 | 57.26 | 63.37 |
| $CH_4$ | 41.19 | 38.10 | 39.28 | 40.46 | 37.28 | 38.52 |
| $NH_3$ | 39.82 | 34.49 | 36.60 | 42.12 | 36.20 | 38.95 |
| CO | 44.16 | 42.35 | 42.58 | 42.67 | 41.31 | 41.51 |
| $N_2$ | 46.35 | 43.53 | 44.30 | 46.79 | 43.48 | 44.68 |
| BF | 35.17 | 35.62 | 34.99 | 39.36 | 37.13 | 37.62 |
| LiF | 47.06 | 34.26 | 40.95 | 44.91 | 30.86 | 38.62 |
| BeO | 36.76 | 26.50 | 32.17 | 35.28 | 23.77 | 30.47 |
| BN | 36.34 | 31.40 | 33.42 | 35.19 | 29.84 | 32.25 |
| $C_2$ | 37.58 | 37.10 | 36.70 | 36.50 | 35.88 | 35.61 |
| CS | 35.00 | 33.61 | 33.86 | 34.31 | 32.74 | 33.11 |
| LiCl | 33.37 | 29.87 | 31.41 | 31.93 | 28.10 | 29.91 |
| $F_2$ | 48.93 | 43.01 | 44.91 | 48.66 | 40.52 | 44.37 |
| $H_2S$ | 33.10 | 31.58 | 31.97 | 34.28 | 32.08 | 32.89 |
| $PH_3$ | 32.22 | 31.25 | 31.37 | 33.29 | 31.95 | 32.30 |
| HCl | 39.38 | 36.53 | 37.59 | 37.84 | 34.72 | 35.98 |
| Ar | 47.34 | 44.06 | 45.28 | 45.57 | 42.09 | 43.47 |
| $SiH_4$ | 33.78 | 32.69 | 32.94 | 33.55 | 32.53 | 32.72 |
| $CH_2O$ | 35.80 | 31.44 | 32.97 | 38.45 | 33.74 | 35.85 |
| $CO_2$ | 40.37 | 38.19 | 38.69 | 39.91 | 36.63 | 37.99 |
| $BH_3$ | 37.61 | 36.67 | 36.61 | 36.20 | 35.23 | 35.21 |
| MSE | 3.08 | -1.38 | 0.43 | 3.12 | -1.98 | 0.50 |
| MAE | 3.08 | 1.75 | 0.60 | 3.12 | 2.05 | 0.60 |
| RMSE | 3.74 | 2.51 | 0.74 | 3.88 | 2.90 | 0.75 |
| SDE | 2.16 | 2.15 | 0.62 | 2.35 | 2.16 | 0.57 |
| Min | 0.64 | -5.74 | -1.56 | 0.76 | -6.49 | -0.85 |
| Max | 7.67 | 1.12 | 1.50 | 8.13 | 0.74 | 1.71 |

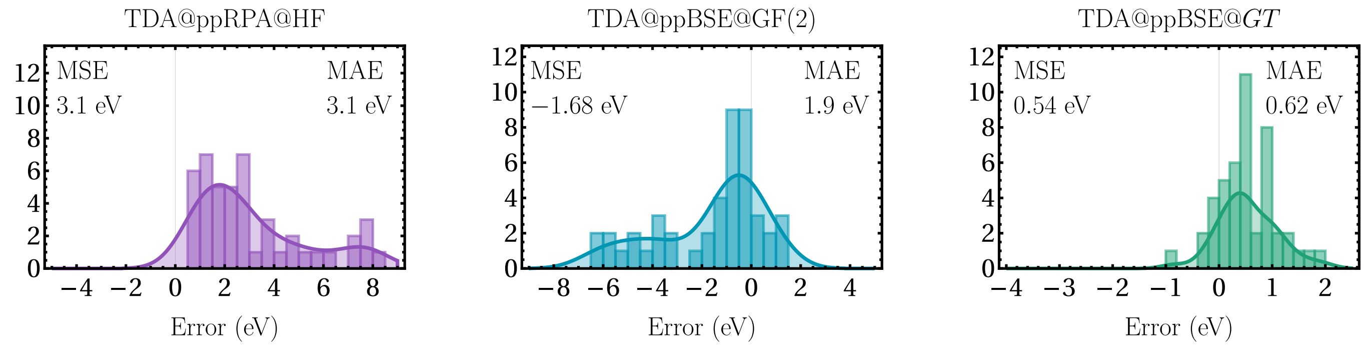


FIG. 6. Histogram of the errors (with respect to FCI) for the singlet and triplet principal DIPs of 23 small molecules in the aug-cc-pVTZ basis set computed at the pp-BSE level using various static kernels: ppRPA@HF, GF(2) and $T$-matrix.

Finally, we also report the main configurations of the singlet and triplet dicationic CI expansions, expressed in terms of the HF neutral ground-state orbitals. The notation $(1b_1)^{-1}(3a_1)^{-1}$ indicates that one electron has been removed from orbital $1b_1$ and another from orbital $3a_1$.

TABLE IV. Main configurations of the CI expansion corresponding to the DIPs benchmarked in this study.

| Molecule | Singlet | Triplet |
|---|---|---|
| $H_2O$ | $(1b_1)^{-2}$ | $(1b_1)^{-1}(3a_1)^{-1}$ |
| HF | $(1\pi)^{-2}$ | $(1\pi)^{-2}$ |
| Ne | $(2p)^{-2}$ | $(2p)^{-2}$ |
| $CH_4$ | $(1t_2)^{-2}$ | $(1t_2)^{-2}$ |
| $NH_3$ | $(3a_1)^{-2}$ | $(3a_1)^{-1}(1e_g)^{-1}$ |
| CO | $(5\sigma)^{-2}$ | $(5\sigma)^{-1}(1\pi)^{-1}$ |
| $N_2$ | $(3\sigma_g)^{-2}$ | $(3\sigma_g)^{-1}(1\pi_u)^{-1}$ |
| BF | $(5\sigma)^{-2}$ | $(5\sigma)^{-1}(1\pi)^{-1}$ |
| LiF | $(1\pi)^{-2}$ | $(1\pi)^{-2}$ |
| BeO | $(1\pi)^{-2}$ | $(1\pi)^{-2}$ |
| BN | $(1\pi)^{-2}$ | $(1\pi)^{-2}$ |
| $C_2$ | $(1\pi_u)^{-2}$ | $(1\pi_u)^{-2}$ |
| CS | $(7\sigma)^{-1}(2\pi)^{-1}$ | $(7\sigma)^{-1}(2\pi)^{-1}$ |
| LiCl | $(2\pi)^{-2}$ | $(2\pi)^{-2}$ |
| $F_2$ | $(1\pi_g)^{-2}$ | $(1\pi_g)^{-2}$ |
| $H_2S$ | $(2b_1)^{-2}$ | $(2b_1)^{-1}(5a_1)^{-1}$ |
| $PH_3$ | $(5a_1)^{-2}$ | $(5a_1)^{-1}(2e_g)^{-1}$ |
| HCl | $(2\pi)^{-2}$ | $(2\pi)^{-2}$ |
| Ar | $(3p)^{-2}$ | $(3p)^{-2}$ |
| $SiH_4$ | $(2t_2)^{-2}$ | $(2t_2)^{-2}$ |
| $CH_2O$ | $(2b_2)^{-2}$ | $(2b_2)^{-1}(1b_1)^{-1}$ |
| $CO_2$ | $(1\pi_g)^{-2}$ | $(1\pi_g)^{-2}$ |
| $BH_3$ | $(1e')^{-2}$ | $(1e')^{-2}$ |

## Appendix A: Gorkov-Hedin equations

The aim of this section is to derive a $GW$-like approximation to the ee anomalous self-energy. This can be done by extending the conventional Hedin equations [12] to the Gorkov propagator [13]. This derivation has already been done in the PhD manuscript of Essenberg [14] but it is reported here for the sake of completeness. The anomalous self-energies are defined through the Gorkov-Dyson equation

$$\boldsymbol{G}(11') = \boldsymbol{G}_0(11') + \int \mathrm{d}(22')\, \boldsymbol{G}_0(12)\, [\boldsymbol{\Sigma}(22') + \boldsymbol{U}(22')]\, \boldsymbol{G}(2'1'), \tag{A1}$$

where the Gorkov propagator and self-energy are

$$\boldsymbol{G}(11') = \begin{pmatrix} G^{\mathrm{he}}(11') & G^{\mathrm{hh}}(11') \\ G^{\mathrm{ee}}(11') & G^{\mathrm{eh}}(11') \end{pmatrix} \qquad \boldsymbol{\Sigma}(11') = \begin{pmatrix} \Sigma^{\mathrm{he}}(11') & \Sigma^{\mathrm{hh}}(11') \\ \Sigma^{\mathrm{ee}}(11') & \Sigma^{\mathrm{eh}}(11') \end{pmatrix}. \tag{A2}$$

The equation of motion for $\boldsymbol{G}$ leads to the following expression of the self-energy [1]

$$\boldsymbol{\Sigma}(22') = -\mathrm{i} \int \mathrm{d}(343'4') \lim_{\delta\to 0^+} \begin{pmatrix} v(24^{--};34'^{-}) & 0 \\ 0 & -v(34^{+};24'^{++}) \end{pmatrix} \boldsymbol{G}_2(4'3;43')\boldsymbol{G}^{-1}(3'2'), \tag{A3}$$

in terms of the external potential

$$\boldsymbol{U}(22') = \begin{pmatrix} U^{\mathrm{eh}}(22') & 0 \\ 0 & -U^{\mathrm{eh}}(22') \end{pmatrix}, \tag{A4}$$

and a generalized two-body Green's function defined as

$$\boldsymbol{G}_2(12;1'2') = (-\mathrm{i})^2 \langle \Psi_0 | \hat{T} \left[ \begin{pmatrix} \hat{\psi}(1)\hat{\psi}(2)\hat{\psi}^\dagger(2')\hat{\psi}^\dagger(1') & \hat{\psi}(1)\hat{\psi}(2)\hat{\psi}(2')\hat{\psi}^\dagger(1') \\ \hat{\psi}(1)\hat{\psi}^\dagger(2)\hat{\psi}^\dagger(2')\hat{\psi}^\dagger(1') & \hat{\psi}(1)\hat{\psi}^\dagger(2)\hat{\psi}(2')\hat{\psi}^\dagger(1') \end{pmatrix} \right] |\Psi_0\rangle\,. \tag{A5}$$

This equation of motion has been derived for the following Hamiltonian $\hat{H}$ in the presence of a potential $\hat{\mathcal{U}}(t)$

$$\begin{aligned} \hat{H}'(t) &= \hat{H} + \hat{\mathcal{U}}(t) \\ &= \int \mathrm{d}(\mathbf{x}_1\mathbf{x}_{1'})\, \hat{\psi}^\dagger(\mathbf{x}_1)h(\mathbf{x}_1\mathbf{x}_{1'})\hat{\psi}(\mathbf{x}_{1'}) + \frac{1}{2}\iint \mathrm{d}(\mathbf{x}_1\mathbf{x}_2\mathbf{x}_{1'}\mathbf{x}_{2'})\, \hat{\psi}^\dagger(\mathbf{x}_1)\hat{\psi}^\dagger(\mathbf{x}_2)v(\mathbf{x}_1\mathbf{x}_2;\mathbf{x}_{1'}\mathbf{x}_{2'})\hat{\psi}(\mathbf{x}_{2'})\hat{\psi}(\mathbf{x}_{1'}) \\ &+ \int \mathrm{d}(\mathbf{x}_1\mathbf{x}_{1'})\, \hat{\psi}^\dagger(\mathbf{x}_1)U^{\mathrm{eh}}(\mathbf{x}_1\mathbf{x}_{1'};t)\hat{\psi}(\mathbf{x}_{1'}). \end{aligned} \tag{A6}$$

The key step of Hedin's derivation is to use the link between the two-body Green's function and the response of the one-body Green's function to an external potential. This is known as the Schwinger relation [15] and it can be easily generalized to the Gorkov propagator

$$\boldsymbol{G}_2(2'3';23) = -\frac{\delta \boldsymbol{G}(3'3)}{\delta U^{\mathrm{eh}}(22')} + G^{\mathrm{he}}(22')\boldsymbol{G}(3'3). \tag{A7}$$

Once injected in the self-energy expression of Eq. (A3), the second term yields

$$\boldsymbol{\Sigma}_{\mathrm{H}}(11') = -\mathrm{i} \int \mathrm{d}(22') \lim_{\delta\to 0^+} \begin{pmatrix} v(12;1'2'^{+})G^{\mathrm{he}}(2'2) & 0 \\ 0 & -v(1'2;12'^{+})G^{\mathrm{he}}(2'2) \end{pmatrix}. \tag{A8}$$

The upper-left block is the usual Hartree self-energy while the lower-right block is the corresponding Hartree term of $\Sigma^{\mathrm{eh}}$ [16]. Therefore, the remaining self-energy term, corresponding to the functional derivative in the Gorkov-Schwinger relation, accounts for the missing static terms, *i.e.*, the exchange (x) term of the normal self-energy and the Bogoliubov (B) term of the anomalous self-energies, as well as the normal and anomalous correlation (c) self-energies. This self-energy can be transformed into the following form

$$\boldsymbol{\Sigma}_{\mathrm{xBc}}(11') = -\mathrm{i} \int \mathrm{d}(22'3'4') \lim_{\delta\to 0^+} \begin{pmatrix} v(12;3'2'^{+}) & 0 \\ 0 & -v(3'2;12'^{+}) \end{pmatrix} \boldsymbol{G}(3'4') \frac{\delta \boldsymbol{G}^{-1}(4'1')}{\delta U^{\mathrm{eh}}(22')}, \tag{A9}$$

using

$$\frac{\delta \boldsymbol{G}(12)}{\delta U^{\mathrm{he}}(1'2')} = -\int \mathrm{d}(44')\, \boldsymbol{G}(14')\frac{\delta \boldsymbol{G}^{-1}(4'4)}{\delta U^{\mathrm{he}}(1'2')}\boldsymbol{G}(42). \tag{A10}$$

Before introducing the inverse dielectric matrix, we take a side step to look at the simplest approximation of the reducible vertex $\boldsymbol{\Gamma}$

$$\boldsymbol{\Gamma}(12;1'2') = -\frac{\delta \boldsymbol{G}^{-1}(11')}{\delta U^{\mathrm{eh}}(2'2)}. \tag{A11}$$

This approximation corresponds to discarding the self-energy in the expression of $\boldsymbol{G}^{-1} = \boldsymbol{G}_0^{-1} - \boldsymbol{U} - \boldsymbol{\Sigma}$. Hence, only the derivative of the potential remains and it yields

$$\boldsymbol{\Gamma}(12;1'2') = \begin{pmatrix} \delta(12')\delta(1'2) & 0 \\ 0 & -\delta(12')\delta(1'2) \end{pmatrix}. \tag{A12}$$

The corresponding self-energy is

$$\begin{aligned}
\boldsymbol{\Sigma}_{\mathrm{xB}}(11') &= \mathrm{i}\int \mathrm{d}(22'3'4') \lim_{\delta\to 0^+} \begin{pmatrix} v(12;3'2'^{+}) & 0 \\ 0 & -v(3'2;12'^{+}) \end{pmatrix} \boldsymbol{G}(3'4') \begin{pmatrix} \delta(4'2)\delta(1'2') & 0 \\ 0 & -\delta(4'2)\delta(1'2') \end{pmatrix} && \text{(A13)}\\
&= \mathrm{i}\int \mathrm{d}(23') \lim_{\delta\to 0^+} \begin{pmatrix} v(12;3'1'^{+}) & 0 \\ 0 & -v(3'2;11'^{+}) \end{pmatrix} \boldsymbol{G}(3'2) \begin{pmatrix} 1 & 0 \\ 0 & -1 \end{pmatrix} && \text{(A14)}\\
&= \mathrm{i}\int \mathrm{d}(22') \lim_{\delta\to 0^+} \begin{pmatrix} v(12;2'1'^{+})G^{\mathrm{he}}(2'2) & -v(12;2'1'^{+})G^{\mathrm{hh}}(2'2) \\ -v(2'1'^{+};12)G^{\mathrm{ee}}(2'2) & v(2'1'^{+};12)G^{\mathrm{eh}}(2'2) \end{pmatrix}. && \text{(A15)}
\end{aligned}$$

This yields the two missing static terms, *i.e.*, the exchange normal self-energy and the Bogoliubov anomalous self-energy [17]. Therefore, this vertex approximation in the Gorkov formalism leads to the Hartree-Fock-Bogoliubov equations while the corresponding approximation applied to a formalism considering only $G^{\mathrm{he}}$ leads to the Hartree-Fock approximation.

Going back to the self-energy expression the next step in Gorkov-Hedin's derivation is to introduce a chain rule with respect to the total potential $V^{\mathrm{he}}(4'4) = U^{\mathrm{eh}}(4'4) + \Sigma_{\mathrm{H}}^{\mathrm{he}}(4'4)$

$$\begin{aligned}
\boldsymbol{\Sigma}(11') &= -\mathrm{i}\int \mathrm{d}(232'3') \lim_{\delta\to 0^+} \begin{pmatrix} v(12;32'^{+}) & 0 \\ 0 & -v(32;12'^{+}) \end{pmatrix} \boldsymbol{G}(33') \frac{\delta \boldsymbol{G}^{-1}(3'1')}{\delta U^{\mathrm{eh}}(22')} \\
&= -\mathrm{i}\int \mathrm{d}(232'3') \lim_{\delta\to 0^+} \begin{pmatrix} v(12;32'^{+}) & 0 \\ 0 & -v(32;12'^{+}) \end{pmatrix} \boldsymbol{G}(33') \frac{\delta V^{\mathrm{eh}}(4'4)}{\delta U^{\mathrm{eh}}(22')} \frac{\delta \boldsymbol{G}^{-1}(3'1')}{\delta V^{\mathrm{eh}}(4'4)} \\
&= -\mathrm{i}\int \mathrm{d}(232'3') \lim_{\delta\to 0^+} \begin{pmatrix} v(12;32'^{+}) & 0 \\ 0 & -v(32;12'^{+}) \end{pmatrix} \boldsymbol{G}(33') \epsilon^{-1}(4'2';42) \frac{\delta \boldsymbol{G}^{-1}(3'1')}{\delta V^{\mathrm{eh}}(4'4)} \\
&= \mathrm{i}\int \mathrm{d}(232'3') \lim_{\delta\to 0^+} \begin{pmatrix} W(14';34) & 0 \\ 0 & -W(34;14') \end{pmatrix} \boldsymbol{G}(33') \tilde{\boldsymbol{\Gamma}}(3'4;1'4')
\end{aligned} \tag{A16}$$

where the irreducible vertex and the screened interaction has been introduced as

$$\tilde{\boldsymbol{\Gamma}}(12;1'2') = -\frac{\delta \boldsymbol{G}^{-1}(11')}{\delta V^{\mathrm{eh}}(2'2)}, \tag{A17}$$

and

$$W(12;1'2') = \int \mathrm{d}(33')\, v(13;1'3')\epsilon^{-1}(23';2'3^{+}), \tag{A18}$$

where the inverse dielectric matrix is

$$\epsilon^{-1}(12;1'2') = \frac{\delta V^{\mathrm{he}}(11')}{\delta U^{\mathrm{eh}}(2'2)}. \tag{A19}$$

The screened interaction admits the same Dyson equation as usual

$$W(12;1'2') = v(12^{-};1'2') - \mathrm{i}W(15;1'5')\tilde{L}(4'5';45)v(24;2'4'), \tag{A20}$$

where the irreducible electron-hole correlation function is

$$\tilde{L}(12;1'2') = \frac{\delta G^{\mathrm{he}}(11')}{\delta V^{\mathrm{he}}(2'2)}. \tag{A21}$$

Its expression can be extracted from the following relation

$$\frac{\delta \boldsymbol{G}(3'3)}{\delta V^{\mathrm{he}}(22')} = -\boldsymbol{G}(3'4')\frac{\delta \boldsymbol{G}^{-1}(4'4)}{\delta V^{\mathrm{he}}(22')}\boldsymbol{G}(43) = \boldsymbol{G}(3'4')\tilde{\boldsymbol{\Gamma}}(4'2';42)\boldsymbol{G}(43), \tag{A22}$$

where one can see that the expression of $\tilde{L}$ is more involved than in the usual Hedin equations because it additionally involves the anomalous Green's functions.

Finally, an expression for the matrix irreducible vertex function is needed

$$\begin{aligned}
\tilde{\boldsymbol{\Gamma}}(4'2';42) &= -\frac{\delta \boldsymbol{G}^{-1}(4'4)}{\delta V^{\mathrm{eh}}(22')} \\
&= \frac{\delta}{\delta V^{\mathrm{eh}}(22')}\left[\begin{pmatrix} V^{\mathrm{eh}}(4'4) & 0 \\ 0 & -V^{\mathrm{eh}}(4'4)\end{pmatrix}\right] + \frac{\delta \boldsymbol{\Sigma}(4'4)}{\delta V^{\mathrm{eh}}(22')} \\
&= \begin{pmatrix} \delta(4'2)\delta(42') & 0 \\ 0 & -\delta(4'2)\delta(42')\end{pmatrix} + \frac{\delta \boldsymbol{\Sigma}(4'4)}{\delta G^{\mathrm{eh}}(55')}\frac{\delta G^{\mathrm{eh}}(55')}{\delta V^{\mathrm{eh}}(22')} + \frac{\delta \boldsymbol{\Sigma}(4'4)}{\delta G^{\mathrm{hh}}(55')}\frac{\delta G^{\mathrm{hh}}(55')}{\delta V^{\mathrm{eh}}(22')} \\
&+ \frac{\delta \boldsymbol{\Sigma}(4'4)}{\delta G^{\mathrm{ee}}(55')}\frac{\delta G^{\mathrm{ee}}(55')}{\delta V^{\mathrm{eh}}(22')} + \frac{\delta \boldsymbol{\Sigma}(4'4)}{\delta G^{\mathrm{eh}}(55')}\frac{\delta G^{\mathrm{eh}}(55')}{\delta V^{\mathrm{eh}}(22')} \\
&= \begin{pmatrix} \delta(4'2)\delta(42') & 0 \\ 0 & -\delta(4'2)\delta(42')\end{pmatrix} \\
&+ \frac{\delta \boldsymbol{\Sigma}(4'4)}{\delta G^{\mathrm{eh}}(55')}[\boldsymbol{G}(56)\tilde{\boldsymbol{\Gamma}}(22';66')\boldsymbol{G}(6'5')]^{\mathrm{eh}} + \frac{\delta \boldsymbol{\Sigma}(4'4)}{\delta G^{\mathrm{hh}}(55')}[\boldsymbol{G}(56)\tilde{\boldsymbol{\Gamma}}(22';66')\boldsymbol{G}(6'5')]^{\mathrm{hh}} \\
&+ \frac{\delta \boldsymbol{\Sigma}(4'4)}{\delta G^{\mathrm{ee}}(55')}[\boldsymbol{G}(56)\tilde{\boldsymbol{\Gamma}}(22';66')\boldsymbol{G}(6'5')]^{\mathrm{ee}} + \frac{\delta \boldsymbol{\Sigma}(4'4)}{\delta G^{\mathrm{eh}}(55')}[\boldsymbol{G}(56)\tilde{\boldsymbol{\Gamma}}(22';66')\boldsymbol{G}(6'5')]^{\mathrm{he}},
\end{aligned}$$

where the notation $[\boldsymbol{G}\tilde{\boldsymbol{\Gamma}}\boldsymbol{G}]^{\mathrm{ee}}$ means the ee matrix element of the product matrix. Due to the chain rule with respect to the Green's functions, this expression is much more cumbersome than the one of Hedin's equations.

This section is concluded by computing the first approximation of $\boldsymbol{\Sigma}$ that stems from Gorkov-Hedin's closed set of equations. The first non-trivial irreducible vertex approximation is

$$\tilde{\boldsymbol{\Gamma}}(4'2';42) = \begin{pmatrix} \delta(4'2)\delta(42') & 0 \\ 0 & -\delta(4'2)\delta(42')\end{pmatrix}. \tag{A23}$$

This leads to the following self-energy

$$\begin{aligned}
\boldsymbol{\Sigma}(11') &= -\mathrm{i}\int \mathrm{d}(33'44')\begin{pmatrix} W(14';34) & 0 \\ 0 & -W(34;14')\end{pmatrix}\boldsymbol{G}(33')\frac{\delta \boldsymbol{G}^{-1}(3'1')}{\delta V^{\mathrm{eh}}(4'4)} \\
&= \mathrm{i}\int \mathrm{d}(33'44')\begin{pmatrix} W(14';34) & 0 \\ 0 & -W(34;14')\end{pmatrix}\boldsymbol{G}(33')\begin{pmatrix} \delta(3'4')\delta(1'4) & 0 \\ 0 & -\delta(3'4')\delta(1'4)\end{pmatrix} \\
&= \mathrm{i}\int \mathrm{d}(33')\begin{pmatrix} W(13';31') & 0 \\ 0 & -W(31';13')\end{pmatrix}\boldsymbol{G}(33')\begin{pmatrix} 1 & 0 \\ 0 & -1\end{pmatrix} \\
&= \mathrm{i}\int \mathrm{d}(33')\begin{pmatrix} W(13';31')G^{\mathrm{he}}(33') & -W(13';31')G^{\mathrm{hh}}(33') \\ -W(31';13')G^{\mathrm{ee}}(33') & W(31';13')G^{\mathrm{eh}}(33')\end{pmatrix} \\
&= \mathrm{i}\int \mathrm{d}(33')\, W(11';33')\begin{pmatrix} G^{\mathrm{he}}(33') & -G^{\mathrm{hh}}(33') \\ -G^{\mathrm{ee}}(33') & G^{\mathrm{eh}}(33')\end{pmatrix}
\end{aligned} \tag{A24}$$

The $GW$ self-energy is recovered in the upper-left block while the anomalous self-energies are also of the $GW$ form. The vertex approximation needs also to be applied to $\tilde{L}$, this is usually referred to as the inner-vertex approximation.

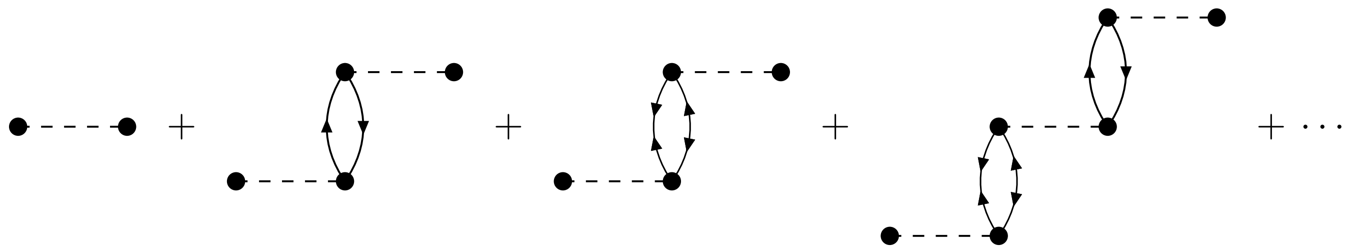

FIG. 7. Diagrammatic representation of the dynamically screened interaction $W$ in the presence of an external pairing field. This corresponds to a resummation of bubble diagrams with two different types of bubbles. The dashed lines represent the Coulomb interaction, the solid lines with arrows denote the one-body propagator while the double-arrowed propagators represent $G^{\text{hh}}$ and $G^{\text{ee}}$.

The resulting electron-hole correlation function is

$$\begin{aligned}\tilde{L}(3'2';32) = \frac{\delta G^{\text{he}}(3'3)}{\delta V^{\text{he}}(22')} &= -\Big(\boldsymbol{G}(3'4')\tilde{\boldsymbol{\Gamma}}(4'2';42)\boldsymbol{G}(43)\Big)^{\text{he}} \\ &= \left(\boldsymbol{G}(3'2')\begin{pmatrix}1 & 0\\ 0 & -1\end{pmatrix}\boldsymbol{G}(23)\right)^{\text{he}} \\ &= G^{\text{he}}(3'2')G^{\text{he}}(23) - G^{\text{hh}}(3'2')G^{\text{ee}}(23)\end{aligned}$$

The first terms of the screened interaction corresponding to this $\tilde{L}$ are represented diagrammatically in Fig. 7. This closely resembles the standard bubble resummation of $GW$ but now two types of bubbles need to be considered.


[1] A. Marie, P. Romaniello, and P.-F. Loos, Anomalous propagators and the particle-particle channel: Hedin's equations, Phys. Rev. B **110**, 115155 (2024).

[2] D. Sangalli, P. Romaniello, G. Onida, and A. Marini, Double excitations in correlated systems: A many-body approach, J. Chem. Phys. **134**, 034115 (2011).

[3] G. Strinati, Application of the Green's functions method to the study of the optical properties of semiconductors, Riv. Nuovo Cimento **11**, 1 (1988).

[4] X. Blase, I. Duchemin, and D. Jacquemin, The Bethe-Salpeter equation in chemistry: relations with TD-DFT, applications and challenges, Chem. Soc. Rev. **47**, 1022 (2018).

[5] X. Blase, I. Duchemin, D. Jacquemin, and P.-F. Loos, The Bethe-Salpeter equation formalism: From physics to chemistry, J. Phys. Chem. Lett. **11**, 7371 (2020).

[6] G. Baym and L. P. Kadanoff, Conservation laws and correlation functions, Phys. Rev. **124**, 287 (1961).

[7] P. Danielewicz, Quantum theory of nonequilibrium processes, I, Ann. Phys. **152**, 239 (1984).

[8] P. Bożek, In medium $T$-matrix for superfluid nuclear matter, Phys. Rev. C **65**, 034327 (2002).

[9] A. Marie, A. Ammar, and P.-F. Loos, The $GW$ approximation: A quantum chemistry perspective, in *Advances in Quantum Chemistry*, Novel Treatments of Strong Correlations, Vol. 90 (2024) pp. 157–184.

[10] E. Rebolini, *Range-Separated Density-Functional Theory for Molecular Excitation Energies*, Ph.D. thesis, Université Pierre et Marie Curie — Paris VI (2014).

[11] A. Marie and P.-F. Loos, A Similarity Renormalization Group Approach to Green's Function Methods, J. Chem. Theory Comput. **19**, 3943 (2023).

[12] L. Hedin, New method for calculating the one-particle Green's function with application to the electron-gas problem, Phys. Rev. **139**, A796 (1965).

[13] L. P. Gorkov, On the energy spectrum of superconductors, Sov. Phys. JETP **34**, 505 (1958).

[14] F. Essenberger, *Density Functional Theory for Superconductors: Extension to a Pairing Mediated by Spin-Fluctuations*, Ph.D. thesis, Max Planck Institute of Microstructure Physics (2014).

[15] P. C. Martin and J. Schwinger, Theory of Many-Particle Systems. I, Phys. Rev. **115**, 1342 (1959).

[16] R. M. Martin, L. Reining, and D. M. Ceperley, *Interacting Electrons: Theory and Computational Approaches* (Cambridge University Press, 2016).

[17] V. Somà, T. Duguet, and C. Barbieri, Ab initio self-consistent Gorkov-Green's function calculations of semimagic nuclei: Formalism at second order with a two-nucleon interaction, Phys. Rev. C **84**, 064317 (2011).
